# Supplementary material for: Large Tandem, Higher Order Repeats and Regularly Dispersed Repeat Units Contribute Substantially to Divergence Between Human and Chimpanzee Y Chromosomes
Source: arXiv:1012.4093 ancillary file (2011-10-08)

**Supplementary text** Description of human and chimpanzee repeats denoted by [b] in Tables 1a and 1b

### *Human 125 bp primary repeat unit*

The GRM peak at 125 bp is due to tandem repeats with 125 bp repeat unit (Fig. 2a). In GRM diagram for Build 37.1 assembly of Y chromosome the 125 bp peak and its multiples present the most pronounced tandem repeat (GRM frequency 77901). This tandem repeat is located in a single array from position 8418147 to 8714453 in NT_011875.12 (chromosome Y positions: 22216726–22513032). Copies of this repeat are not dispersed to other locations in Y chromosome or in any other chromosome.

The 125 bp tandem repeat unit in human Y chromosome was reported previously (Skaletsky et al. 2003; Warburton et al. 2008).

### *Absence of chimpanzee 125 bp primary repeat unit*

In the Build 2.1 assembly for chimpanzee Y chromosome there is no GRM peak at 125 bp repeat unit length (the GRM frequency for the length of 125 bp is smaller than the mean noise in the 20 bp interval from 115 bp to 135 bp). It is possible that the 125 bp tandem repeat lies in the unsequenced section of Y chromosome (the section beyond the 24 Mb position is not sequenced). The BLAST search using the 125 bp human consensus repeat unit shows that such sequence is also not present in any other chimpanzee chromosome of the Build 2.1 ensemble.

### *Chimpanzee 5096 bp primary repeat unit*

The GRM peak at 5096 bp is due to tandem arrays of 5096 primary repeat units in NW_001252916.1 (five highly convergent copies of consensus length 5096 bp, located from position 49181 to 69563, and two highly convergent reverse complement copies, located from position 175432 to 185622). In addition, we find three dispersed copies starting at positions 45312 in contig NW_001252920.1, 53619 and 156334 in contig NW_001252924.1. The GRM diagram of the 5096 bp consensus sequence has no significant peaks, i.e., there is no any internal periodic substructure within this repeat unit. The mean divergence of copies within the tandem with respect to the 5096 bp consensus is 0.1%.

### *Absence of human repeat unit corresponding to the chimpanzee 5096 bp primary repeat unit*

In the Build 37.1 assembly for humane Y chromosome we find no analog of the chimpanzee 5096 bp tandem repeat unit. However, there are two dispersed copies in NT_011875.12 and two in NT_011903.12 having divergence less than 5% with respect to chimpanzee 5096 bp repeat unit. Additionally, there are more than 1500 dispersed partial segments (of ∼3 kb) at the 15-30 % level of divergence.

### *Chimpanzee 10762 bp primary repeat unit*

The GRM peak at 10762 bp is due to two tandem repeat arrays: three copies (consensus length 10762 bp, consensus sequence in Supplementary table 13), from position 276373 to 308349 in NW_001252919.1 (divergence with respect to consensus ∼1%) and two copies, from position 2823896 to 2845204 in NW_001252921.1 (divergence with respect to consensus ∼3%). In addition, there is one dispersed copy in NW_001252925.1 (divergence 2%).

### *Human ∼20309 bp primary repeat unit and its ∼10.8 kb subsequence corresponding to the chimpanzee 10762 bp primary repeat unit*

The GRM peak at 20309 bp is due to highly identical tandem repeat (4 copies) in the NT_011878.9 contig. The corresponding 20309 bp consensus sequence is shown in Supplementary table 14. Divergence of repeat copies with respect to consensus is less than 0.5%.

In the contig NT_086998.1 we identify 3.5 highly identical ∼20346 bp monomer copies (without internal repeat structure) at start position 205852, with divergence below 1%. This tandem gives rise to the GRM peak at ∼20346 bp. Divergences between copies

from these two tandem arrays are below 1%. Additionally, there is one copy and the front segment of the second copy in NT_011896.9.

There is an interesting connection between the human ~20.3 kb primary repeat unit and chimpanzee ~10762 bp primary repeat unit. The ~20.3 kb primary repeat unit can be approximately fragmented into four segments:

20.3 kb sequence ≈ S1(0.3 kb) S2(6.8 kb) S3(3.6 kb) S4(9.7 kb).

This repeat unit is connected to the chimpanzee 10762 bp primary repeat unit which can be approximately (at the level of divergence less than 5%) expressed in the form:

10762 bp sequence ≈ S1(0.3 kb) S3(3.6 kb) S2(6.8 kb)

i.e., the chimpanzee 10762 bp repeat unit contains (at more than 95% identity level) the first three subsections from the human ~20309 bp primary repeat unit (S1, S2, S3), but the ordering of S2(6.8 kb) and S3(3.6 kb) segments is reversed. This reveals that the S1, S2 and S3 segments in human and chimpanzee Y chromosome derive their existence prior to the human – chimpanzee separation.

The ~20.3 kb repeat unit encodes the TSPY gene (Skaletsky et al. 2003; Warburton et al. 2008).

### *Human 10848 bp primary repeat unit*

The GRM peak at 10848 bp (Fig. 2b) is generated by two tandem arrays in NT_011903.12 (repeat unit consensus length 10848 bp, consensus sequence in Supplementary table 16). The first tandem of 2.6 copies is located from position 1361304 to 1389633 and the second tandem of 1.6 reverse complement copies from 3032722 to 3050216. The mean divergence between HOR copies and consensus is below 1%.

The chimpanzee repeat units of ~10853 bp approximately correspond to human ~10848 bp repeat units (divergence ~3%).

We note that the GRM diagram of the 10848 consensus repeat unit exhibits a moderate peak at 2455 bp (Supplementary Fig. 2), revealing that the 10848 consensus repeat unit is not entirely monomeric, but has a moderately pronounced internal repeat structure. Using GRM we obtain its dominant key string GAGCCTTA and performing the corresponding KSA fragmentation we find within the 10848 bp consensus sequence the two dispersed copies of similar ~0.2 kb motifs at a mutual distance of 2452 bp. The first 30 bases in the first of these two subsequences starts with GAGCC TTATC AGCAG CGTAA GAAAT AACTT and in the second subsequence only one of these 30 bases is changed (at the $12^{th}$ position the base G is replaced by C). Going further along these subsequences, divergence between them gradually increases (divergence is 2% for bases No. 1 to 35 in subsequences, 11% for bases No. 36 to 70, 20% for bases No. 71 to 140, 46% for bases No. 141 to 260 and further away similarity rapidly disappears). This peculiar pattern of two distant motifs as approximately similar subrepeat copies within a large repeat monomer could be considered as an internal dispersed repeat pattern *in statu nascendi.*

Previously, one tandem array with 2.4 repeat copies of 10.8 kb was reported (Warburton et al. 2008).

### *Human 15766 bp dispersed repeat*

The GRM peak at 41854 bp is due to duplication of two highly identical 15766 bp copies (divergence 2%) in NT_011875.12, with 41854 bp spacing between their start positions. The first part of these dispersed repeats (from position 1 to 6011 bp) is dispersed (divergence of 10%) throughout the whole human and chimpanzee genomes.

### *Human 15775 bp primary repeat unit*

The 15775 bp peak for human Y chromosome is due to tandem of two highly identical 15775 bp repeat copies (divergence less than 0.1%) in NT_011896.9 (start position 3893852). Additionally, there is one dispersed 15775 bp repeat copy (divergence 2%) in NT_011651.17.

The corresponding repeat unit in chimpanzee Build 2.1 assembly is absent.

### *Chimpanzee 60523 bp repeat unit*

The GRM peak at 60523 bp is due to tandem of two copies in NW_001252918.1, with repeat unit of consensus length 60523 bp (zero divergence). This segmental duplication

extends from position 1 to 121045 in NW_001252918.1. Additionally, single dispersed copies of the 60523 bp sequence appear in contigs NW_001252922.1 (divergence 0.5%) and NW_001252919.1 (divergence 0.7%). GRM analysis does not reveal any internal repeat structure of the 60523 bp repeat unit, showing its monomeric character.

### *Human ∼60910 bp repeat unit*

In the Build 37.1 assembly for human Y chromosome we find no analog of the chimpanzee ∼60523 bp tandem repeat unit. However, we find two dispersed and riddled copies in contig NT_011875.12 (start positions 5898643 and 6622156) with divergence ∼3% with respect to chimpanzee 60523 bp repeat unit.

### *Chimpanzee ∼72140 bp repeat unit*

The GRM peak at 72140 bp is due to approximate tandem in NW_001252923.1, with repeat unit of consensus length 72140 bp (two copies, divergence 0.02%, separated by a small 362 bp spacing). Additionally, single dispersed copies appear in contigs NW_001252925.1 (divergence 0.3%), NW_001252915.1 (divergence 0.3%), NW_001252917.1 (divergence 0.3%), and NW_001252919.1 (divergence 2%). GRM analysis does not reveal any internal repeat structure of the 72140 bp repeat unit.

### *Human ∼72140 bp repeat unit*

In the human Y chromosome assembly we find two riddled and dispersed copies in contig NT_011875.12 (start positions 6031103 and 6480818, divergence to chimpanzee consensus ∼3%).

**Supplementary table** I: Detailed monomer structure of human alphoid HOR copies in contigs NT_011878.9 and NT_087001.1 which corresponds to Fig. 1.

| Segment[a] | Position[b] | Length (bp) | Composition | No.pJ$\alpha$[c] | Divergence (%)[d] |
|---|---|---|---|---|---|
| **Contig NT_011878.9** | | | | | |
| 3 mon. | 792452 | 513 | $m06, m07, m08$ | 2 | 0.4 |
| Q01[e] | 792965 | 210 | | | |
| 3 mon. | 793175 | 513 | $m15, m16, m17$ | 3 | 0.0 |
| 5 mon. | 793688 | 848 | $m19, ..., m23$ | 3 | 0.1 |
| 12 mon. | 794536 | 2041 | $m34, ..., m45$ | 9 | 0.0 |
| 17 mon. | 796577 | 2897 | $m01, ..., m17$ | 7 | 0.3 |
| 4 mon. | 799474 | 682 | $m13, ..., m16$ | 3 | 0.0 |
| Q02[f] | 800156 | 170 | | | |
| Q03[g] | 800326 | 168 | | | |
| 28 mon. | 800494 | 4770 | $m18, ..., m45$ | 18 | 0.4 |
| 17 mon. | 805264 | 2896 | $m01, ..., m17$ | 7 | 0.0 |
| 5 mon. | 808160 | 848 | $m19, ..., m23$ | 3 | 0.1 |
| 7 mon. | 809008 | 1194 | $m34, ..., m40$ | 6 | 0.1 |
| Q04[h] | 810202 | 278 | | | |
| 2 mon. | 810480 | 335 | $m44, m45$ | 0 | 0.6 |
| 15 mon. | 810815 | 2417 | $m01, ..., m14, d15$[i] | 4 | 0.1 |
| **Contig NT_087001.1** | | | | | |
| 5 mon. | 1 | 844 | $d14$[j]$, m15, ..., m18$ | 4 | 1.1 |
| Q05[k] | 845 | 146 | | | |
| 24 mon. | 991 | 3909 | $m45, m01, ..., m23$ | 11 | 0.3 |
| 3 mon. | 4900 | 512 | $m34, m35, m36$ | 2 | 0.0 |
| Q06[l] | 5412 | 171 | | | |
| 9 mon. | 5583 | 1529 | $m37, ..., m45$ | 7 | 0.4 |
| 23 mon. | 7112 | 3912 | $m01, ..., m23$ | 11 | 0.5 |
| 12 mon. | 11024 | 2045 | $m34, ..., m45$ | 9 | 0.3 |
| 23 mon. | 13069 | 3917 | $m01, ..., m23$ | 11 | 0.1 |
| 12 mon. | 16986 | 2041 | $m34, ..., m45$ | 9 | 0.2 |
| 45 mon. | 19027 | 7484 | $m01, ..., m45$ | 26 | 0.3 |
| 5 mon. | 26511 | 848 | $m01, ..., m05$ | 0 | 0.7 |

[a]Subsequence of $n$ alpha monomers.
[b]Start position of segment within contig.
[c]Number of pJ$\alpha$ motifs in segment.
[d]Divergence of segment with respect to consensus.
[e]Segment significantly different from HOR monomers.
[f]Monomer significantly different from HOR monomers. The closest HOR monomers are m24 i m34 (19 base differences).
[g]Monomer significantly different from HOR monomers. The closest HOR monomer is m28 (20 base differences).
[h]Segment significantly different from HOR monomers.
[i]Truncated after the first 34 bases from m15.
[j]Truncated before the last 166 bases from m14.
[k]Monomers of lengths 165 and 146 bp, significantly different from HOR monomers.
[l]Monomer significantly different from HOR monomers. The closest HOR monomer is $m23$ (13 base differences).
Average divergence with respect to consensus HOR: 0.3%.

**Supplementary table** II: Human alpha monomers $m01, ..., m45$ in consensus alphoid 45mer (7,662 bp) determined by GRM analysis of genomic sequence (contigs NT_011878.9 and NT_087001.1). In parentheses: lengths of monomers (in bp).

$m01$(171)
```
GTTAAGAACATCACAAAGAAGTTTCTCAGAATGCTTCTGTGTAGTTCTTACGTAAAGATATTTCCTTTTACAC
AATAGGCAGAAAAGTGCTCCAAATATCCACTTGAAGATTCTACAAAAACCGTGTTTCAAAACTGCCGAATCAA
AAGAAAGGTTCAACTCTGTGAGATG
```

$m02$(171)
```
AATGCACACATAACAAAGGAGTTTCTCAGAATGCTTCTGTGTAGCTTTTATATGAAGACATTTAGTTTTCCAC
AACAGGCCTCAAAGCTCTCTCCATATCCACTTGCAGATTCTACCGAAAGAGTGCTTCCAAACTGCTCAATCAA
AAGAGACATTCAAATCTGTGAGGTG
```

$m03$(167)
```
AATGCAGACATCGTAAAGAAGTTTCTCAGAATGCTTCTGTGTATTTTTTGTGTGAAGTTATTCGTTTTTGCAC
CATAGGCCTCCAAGCGTTCTAAATATCCACTTCTAGATTCTACAAAAAGAGAGTTTCAAAACTACTCAAACAA
AAGGTTCAATTCTGTGAGTTG
```

$m04$(168)
```
AAAGCAAACATCACAAAGAAGTTTCTCAGAATGCGTCTGTGTAGTTTTGATGTGAAGATATTTCCTTTTCACA
GTAGAATGCAAAGGGCTCCAAATATCCACTTGGAGATTCTACAAAAAGAGTTTCAAAACCGCTCTGTCAAATG
ATAGGTTGAACTCCCGGAGGTG
```

$m05$(171)
```
AATACACACATCACAAAGAGGTTTCTCAGCATGCTTCTGTGTAGTTTTTATGTAAACATATTTCCGTTTCTAT
CATAGGCCTCAAAGTGCTCCAAATATTCACTTGTACATTCTACCAAACGAGTATTTCAAAACTGCTCAATCAA
ATGGAAGGTTCAAAACCGTGACATG
```

$m06$(172)
```
AATGCCCACATCACAAAGTAGTTTCTCAGAATGCTTCTGTGTAGTTTTTATGTGAAGATATTTCCTTTTCCAC
AACAGCGTGCAAAACGCTTCAAATATGCCCTTAGAGATTCCACAAAAAGAGTGTTTCCAAACTACTCAAATCA
AAAAATGATTTCAACTCTGTGAGATG
```

$m07$(170)
```
AATGCACACATCACAAACTAGTTTCTCAGAATGTTTCTGCCTGGTTCTCATGCGAAGATAGTTCCTTTTTCAC
CATAGGCCGCAATGTACTCCAAATATCCACCTGCAGATTCTACAAAAGTGAGTTTCAAAACTGCTCTATCAAA
AGATCAGTTCGTCTCTGTGAGTTG
```

$m08$(171)
```
AATGCATACATCAAAAAGAAGCTTCTCAAAATGCTTCTGTGTGGTTTTTCGGTGAAGATAGTTCTTTTTCTAC
CATAGGTCTCAAACCACTCCAAATATCCACTTGTAGATTCTATAAAAAGGAATGTTCAAAATTGCTCAATAAA
AATAAAGTTTCAACACCGTGAGATG
```

$m09$(171)
```
AGTGCACAAATCACAAAGGAGTTTCTCAAAATGCTTCTGGGTAGTTTTTCTGTGAAGATAGTTCCTTTTCTAC
CATGGGCCACAAAGGGCTCCAAATACCCACTTGCAGATTCTACAAAAAGAGAGTTTCACAACTGCTCTATCAA
ACAATATGTTCAACTTTGTGGGTTG
```

$m10$(170)
```
AACACAAATATCACAAGAATTTTCTCCCAATGCTTCTGTGTAGTTTTTATGTGAAGACATTTCTTTTCCCTCC
ATAGTCCACAAAGTGCTCCAAATATCCACTTACATATTCTAGAAAAAGATTGCTTGGAAACTGCACAATGAAA
AGAAAGGTTCAAATATATGAGATG
```

$m11$(170)
```
AATGCACACATCACAAAGAAGTTTCTCAGAATCTCTCTGTGTAATTTTTATGTGAAGATATTTCCTTTCCCAC
CTTAGGTCTTAAAACGCTCCAAATATCCACTTGCAGATACTACAAGAAGATTGTTTCAAAACTGCACAAAAAA
AGAAATGTTCAATTCTGTTTGATG
```

$m12$(171)
```
AATGCACACATCACAAAGAAGTTTCTCAGAATGCTTCTCTGTAGTTTTTATGTGAAGATATTTCCTTTTCCAC
AATAGGCCTCAAAGGGCTCCAAATATCCACTTCCAGATTCTATGAAAAGAATATTTCCAAACTGCTCAATCAT
```

AGGAAATGTTCAACTCTGTGAGATG

$m13(170)$
AATGCACACATCACAAGAAATTTCTCAGAATCCTTCAGTGTAGGTTTTATGAGAAGATAATTCCTTTTCCACA
ATAGTTCTCAAAGCACTCAAAATATCCACTTGCAGATTCTACAAAAGGAGTATTTCAAAACTGCTCAATCAAA
AGAAAGGTTCAACTCTGTGAGATG

$m14(170)$
AATGGACACATCACAAAGAAGTTTCTCAGAATGCTTCTGTGTAGTATTTTTGTGAAGATATTTCTTTTCCACC
ATAGACCGCCAGGGGACACAAATATCCACTTTCAGATTCTACAACAAGAGAGGTTCAAAACTACTCGATCAAG
AGATGGTTTCAACTATGTGAGTTG

$m15(171)$
AATGCACACATCACAAAGAACTATGTCGGAATTCTTCTGTGTAGTTTTTATGTGAAGATATTTCCTTTTCCAC
AATAGACGTCAAAGTGATCCAGATATCCACTTGCAGATTCCACAAAAAGAGTGTTTCAAAAGTGCACAACCAA
AAGAAAGGTTCAACTAGGTGAGATG

$m16(171)$
AATGCACACATCAGAAGGAAGTTTCTCAGAATGCTTCTGCATAGCTTTTAAGGGAAGATACTTCCTTTTCCAA
CATAGGCCTCAAAGCACTCCAAATATCCTCCTGGAGATACCACAAAAAGAGTGTTTGCAAACTGCTCAATCAA
AAGAAAGATTTAACTCTGTGAGATG

$m17(171)$
AATCCACACATGACAAAGAAGTTTCTCAGAATGCTTCTGTGTAGTTTTTATGTGAAGATATTTCCTTTTCCAC
AATAAGACCCAAAAGGCTCCAAATATTCACTTGCAGATTCTAAAAAAAACAGTGTTTCAAAACTGCTCAATCA
AAAGATAGTTCAACTCTGTGAGAAG

$m18(172)$
AATGCTCACATCACTGAGAAGTTTCTCAGAATGCTTCTGTGTAGTTTTTATGTGAAGATATTTCCTTTTCCAC
AATAAGACCCAAAAGGCTCCAAATATTCACTTGCAGATTCTAAAAAAAACAGTGTTTCAAAACTGCTCAATCA
AAAGAAAGGTTCAACTCTGTGAGAAG

$m19(171)$
AATGCTCACATCACTGAGAAGTTTCTCAGAATGCTTCTGTGTAGTTTTTATATGAAGATATTTCCTTTCCCAC
CGTAGGCCACAAAAGGCTCCAAATATCCACTTGCAGATACTATGAAAAGAGAGTTTCAAAACTGCTCATTCAA
AAGATAGGTTCAACTCTGTGGTTTG

$m20(168)$
AATGCACACAGCACAAAGAAGTTTCACAGAATGTGTCTGTGTAGTTTTTATGTGCGGATGTTTCCTTTTCCAC
CATATGCCTAAATATTTCCCAATTTCCACTTGCAGATTCCACAAGAAGAGTGTTTCAAAACTGCTGTATCAAA
TAAAGTTGAACTCTGTGAGGTG

$m21(171)$
AATGCACACAGCACAAAATGGTTTCTCAGAATGCTTCCTTGTTGTTTTTATATGAAGATGTTTCCTTTTCAAC
AATAGGCCTCAAAGTGCTTCAAATGTCCACTTGCAGATTCTACAAAAAGAGTGTTTCAAAACTGCTCAATCAA
AAGAAAGGTTCGACTCTGGGAAATT

$m22(167)$
AATGCACACATCACAAAGAAGTTTCTCAGCTTCTGTGTAGTTTTCATGTGAAGTTATTTCCTTTTCCACAATA
GGCCGCAAAGGGCTCCAAATATCAACTTACAGATTCTAGGAAAAGAGAGTTTCAAAACTGCTCTACGAAAAGA
TAGGTTGAACTCTGTGAGATG

$m23(171)$
AATGCACACATCACAAAGAAGTTTCTCAGAATGCATCTGTGTAGTTTTTACGGGAAGATATTTCCTTTTCCAC
CATCTTCCACAAAGGTCTCCAAGTAACCACTTGCAGATTCTACAGAAAGACACTTTAAAAACTGCTCTATCAA
AAGATCAGTTCAAGTCTGTGGTTTG

$m24(171)$
AATGCACACATCACAAAGAATTTTCTCAGAATGCTTCTGTGTAGTTTTCATATGAAGATATTTTCTTTTCCAC
CATAGGCCTCAAAGTGCTCCAAATATCCACTTGCAGATTCTACAAAAAGAGTGTTTCAAAACTGCTCAATCAA
AAGAAAGGTACAACTCTTTGTGATG

$m25(171)$
AATTCACTAATAACAAAGACGTTTCTCACAATGCTTCTCTGTAGTTTTTATGTGAAGATCTTTCCTTTTCTAC
CATAGGCATCAAAGCACTACAAATATCCAATAGCAGATTCTACAAAAAGAGTGTTTCAAAACTGCTCAATCAA
ATGAAACGTTCAACCCTGTGAGATG

$m26(169)$
AATGCAGACATTAAAAGATAGTTTCTCATTATGGTTCTGGGTAGTTTTTATGTGAACTTATTTCCTTTTCCAA
AATAGGCCGGAAAGGGCTCCAAGTATCCACTTGCAGATTCTACAAAAAGAGATTCAAAACTCCTCAATCAAAA
GATAGGTTGAACTCCGTGAGATT

$m27(171)$
AATGCATACATCACAACGAAGTTTCTCAGAGGGCTTCATTGTAGTTTTATGGGAAGATATTTCCTTTTCCACT
ATATGTCTCAAAGATATCCAAATATACACTTGCAGATTCTACAAAATGAGAGTTTCAAAACTGCTCTGTCAAA
AAAAGAGGTTCAGCTGCATGAGTTG

$m28(171)$
AATGCACACATCACAAAGAAGTTTCTCAGAATGCTTCTGTGTATTTTTTATGTTAAGATATTTTCTTTTCCAC
CATAGGCTGCAAAGGGCTCCAAATATCCACTTGCAGATTCTACAAAAAGAGATTTTCAAAACTGCTCAATCAA
AAGAAAGGCTCAACTCTGTGAGATG

$m29(171)$
AATGCACACAAAACAAAGGAGTTTCTGCAAATGCTTCTGTGTAGTTTTTAAGTGAAGATACTTCCTTTTCCAC
AATAGGTCTCGAAGCCCTCCAAATATCCAAATGTGGATTCTACAAAAAGAGTGTTTCAAAACTGCTCAATCAA
ATGGAAGCTTCAACTCTAAGAAATG

$m30(171)$
AATACACACCTGACAAAGAAGTTTCTCAGAATGATTTTGTGTAGTTTTTTGGGGAAGGCGTTTTCCTTTCCAC
CATCGGTCACAAAGGCCTCCAAATAACCACATGCAGATTCTACACAAGGAGAGTTTCAAAACTGCTCTGTCAA
AAGATAGGTTCAGCTCTGCGAGTTG

$m31(171)$
AATGCACACATCACAGACAAGTTTCTCAGAATGCTTCTGTGTAGTTTTCATGTGAAGATATTTCCTTTTCCAC
TTTAGGCCACAAAGCACTCCAAATATCCACTTGCAGAAACTACAAAAAGAGTCTTTCAAAACTGCTCAAGCAA
AAGAAAAGTTCAACTCTGTGAGATG

$m32(170)$
AATGCACACATCACAAAGGAGTTTCTGAGAATGCTTCTGTGTAGTTTTTATGTGAAATATTTCCTTATCCACC
ATAGGCTTCAAAGTGCTCCAAATATTCACTTGCAAATTATAAAAACAGAATTTTTCAAAAATGCTCAGTTAAA
AGAATGTTTCAACACTGTGAGATG

$m33(169)$
AATGCACACATCACAAAAAGTTTCTGGGAATGCTTCTGTGTGGTTTTTATGTGAGGATATTTCCTTTTCCACC
ATAGACTACAAAGGGCTCCAAATATCCACTTGCAGATTCTACAAAAAGAGAGTTTCGAAATGCTCTATCAAAA
GATAGGTTCAAATATGTGATATG

$m34(171)$
AATGCACACATCACAAAGAATTTTCTCAGAATGCTTCTGTGTAGTTTTCATATGAAGATATTTCCTTTTCCAC
CATAGGCCTCAAAGCACTCCAAATATCCACTTGCAGATTCTACAAAAAGAGATTTTCAAAACTAGTCAATCAA
AAGAAAGGTTCAACTCTGTCAGTTG

$m35(170)$
AATGCACATATCACAAACAAGTTTCTCGGAATGCGTCTGTGTAGTTTTTATGTGAAGATATTTCCTTCTCCAC
AACAGGCCTCAAAGTGCTCCGAATATCCACTTGCAGATTTTACTAAAGAGTGTTTCCAAACTGCTCAATCAAG
AGGAAGTTTCAAGTCTGTGAGCTG

$m36(171)$
AACGCACACATCACAAAGTAGTTTCTGAGAATGCTTCTGTGTAGTTTTTATGTGAAGATGTTTCCTTTTCCAC
CATAGGCTGCAAAGGGCTCCAAATATCCACTTGCAGATTCTACAAAAAGAGAGTTTCAAAAGTGCTCTATCAA
AAGATAGGTTCAACTATGTGATATG

$m37(171)$
AATGCACACATCACAAAGTAGTTTCTCAGAATGCTTCTGTGTAGTTTTTATGTAAAGATATTTCCTTTTCCAC

CATAGGCCTCAAAGCACTCCAAATATCCACTTGCAGATTCTACAAAAAGAGATTTTCAAAACTATTTAATCAA
AAGAAAGGTTCAAATCTGTCAGTTG

$m38(171)$
AAGGTACATATCACAAACAAGTTTATTGGAATGCTTCTGTGTAGTTTTTATGTGAAGATATTTCCTTTTCCAC
AACAGGCCTCAAGGTGCTCCAAATATCCACTTGCAGATTTCACTAAAAGTGTGTTTCCAAGCTGCTCAATCAA
GAGGAAGTTTCAAGTCTGTGAGGTG

$m39(171)$
AATGCACACATTACAAAGAAGTTACTGAGAATGCTTCTGTGTAGTTTTTATGTGAAGATATTTCCTTTTCCAC
CGCAGGCCTCAAAGCGCTGCAAATATCCACTTGCAGATTCTACAAAAAGAGAGTTTCAAAACTGCTGTATCAA
AAGATAGGGTCAACTCTGCGAGTTG

$m40(169)$
AATAAACACATCACAAATAAGTTTCTGGGAACGCTTCTGTATAGTTTTATGTGAATATATTTCCTTTTCCACC
ATATGCCTCAAAGCACTCCAAATATCCACTTGCACATTATAGAAACATAGTCTTTCAAAACTTGTCAATCAAA
GAAAGGTTCAACTCCGTGAGATG

$m41(171)$
AGTGCACACATCACAGAGAAGTTTCTCGGAATGTTTCTGTGTAGTTTTTATGTGAAGATATTGCCTTTTCCAC
AATAGGCCTCAAAGCGTTCCAAATATCCAATTGCAGATTCCACAAAAAAAGTTTTTTAAAACTGCTCAATCAA
ATGATAGATTAAACTCTGTGAGATT

$m42(171)$
AGTGCACACATGTCAAAAAAGTTTCTCAGAATGCTTCTGTGTACTTTTTAGGGGAAGATATTTCCTTTTCCAC
CATCGGCCACAAAGGACTCCAAATAACCACATGCAGATTCTAGTAACACAGAGTTTCAAAACTGCTCTATCAA
AAGATAAGTTCAACTCTGAGAGTTT

$m43(170)$
AGTGCAACCATCGTGAAGAAGTTTCTCAGAATGCTTCTGAGTAGTGTTTATGTGAAGATATTTCCTTTTCCAC
CATAGGCCTGAAAGCCCTCCAAATATCCACTTGCAGATCCTACAAAAAGAAAGTTTCGAAATGCTCTCTCAAA
CGATAGTTTCGACTCTGTGGTATG

$m44(169)$
AATACACACATCACAAAGAAGTTTCTCAGAATGCTTCTGTGTAGTTTTTAAATGAAGATATTTCTTTTTCCAC
CATAGGCCTCAAAGCACTCCAAATATGCACTTCCAGATTCTACAAAAAGAGTGTTTCAGAACTGCTCAATCAA
AAGGAAGGTTCCAGTCTGAGACA

$m45(166)$
AATACACACATCAAAAGGTAGTTTCTCAGAATGCTTCTGTGTAGTTTTTATGTGAAGATATTTTCCTTTCCAC
CATAGGCCACAAATGGCTCTAAATACCCACTTACATTTTCCACAAAAAGAGAGTTTCAAAACTGCTCTACCAA
AGGTAAGTTTAACGCTGTGA

**Supplementary table** III: Human alpha monomers, denoted by $w01, ..., w35$, determined by GRM analysis of genomic sequence of the 5,941 secondary unit repeat in DYZ3 alphoid block from (Skaletsky et al. 2003), corresponding to internal HOR. For sequences of monomers $w20$ and $w29$ we found a 67-bp deletion and 53-bp insertion, respectively.

$w01(169)$
GATATTTCTTTTTCCACCATAGGCCTCAAAGCACTCCAAATATGCACTTCCAGATTCTACAAAAAGAGTGTTT
CAGAACTGCTCAATCAAAAGGAAGGTTCCAGTCTGAGACAAATACACACATCAAAAGGTAGTTTCTCAGAATG
CTTCTGTGTAGTTTTTATGTGAA

$w02(166)$
GATATTTTCCTTTCCACCATAGGCCACAAATGGCTCTAAATACCCACTTACATTTTCCACAAAAAGAGAGTTT
CAAAACTGCTCTACCAAAGGTAAGTTTAACGCTGTGAGTTAAGAACATCACAAAGAAGTTTCTCAGAATGCTT
CTGTGTAGTTCTTACGTAAA

$w03(171)$
GATATTTCCTTTTACACAATAGGCAGAAAAGTGCTCCAAATATCCACTTGAAGATTCTACAAAAACCGTGTTT
CAAAACTGCCGAATCAAAAGAAAGGTTCAACTCTGTGAGATGAATGCACACATAACAAAGGAGTTTCTCAGAA
TGCTTCTGTGTAGCTTTTATATGAA

$w04(171)$
GACATTTAGTTTTCCACAACAGGCCTCAAAGCTCTCTCCATATCCACTTGCAGATTCTACCGAAAGAGTGCTT
CCAAACTGCTCAATCAAAAGAGACATTCAAATCTGTGAGGTGAATGCAGACATCGTAAAGAAGTTTCTCAGAA
TGCTTCTGTGTATTTTTTGTGTGAA

$w05(167)$
GTTATTCGTTTTTGCACCATAGGCCTCCAAGCGTTCTAAATATCCACTTCTAGATTCTACAAAAAGAGAGTTT
CAAAACTACTCAAACAAAAGGTTCAATTCTGTGAGTTGAAAGCAAACATCACAAAGAAGTTTCTCAGAATGCG
TCTGTGTAGTTTTGATGTGAA

$w06(168)$
GATATTTCCTTTTCACAGTAGAATGCAAAGGGCTCCAAATATCCACTTGGAGATTCTACAAAAAGAGTTTCAA
AACCGCTCTGTCAAATGATAGGTTGAACTCCCGGAGGTGAATACACACATCACAAAGAGGTTTCTCAGCATGC
TTCTGTGTAGTTTTTATGTAAA

$w07(171)$
CATATTTCCGTTTCTATCATAGGCCTCAAAGTGCTCCAAATATTCACTTGTACATTCTACCAAACGAGTATTT
CAAAACTGCTCAATCAAATGGAAGGTTCAAAACCGTGACATGAATGCCCACATCACAAAGTAGTTTCTCAGAA
TGCTTCTGTGTAGTTTTTATGTGAA

$w08(172)$
GATATTTCCTTTTCCACAACAGCGTGCAAAACGCTTCAAATATGCCCTTAGAGATTCCACAAAAAGAGTGTTT
CCAAACTACTCAAATCAAAAAATGATTTCAACTCTGTGAGATGAATGCACACATCACAAACTAGTTTCTCAGA
ATGTTTCTGCCTGGTTCTCATGCGAA

$w09(170)$
GATAGTTCCTTTTTCACCATAGGCCGCAATGTACTCCAAATATCCACCTGCAGATTCTACAAAAGTGAGTTTC
AAAACTGCTCTATCAAAAGATCAGTTCGTCTCTGTGAGTTGAATGCATACATCAAAAAGAAGCTTCTCAAAAT
GCTTCTGTGTGGTTTTTCGGTGAA

$w10(171)$
GATAGTTCTTTTTCTACCATAGGTCTCAAACCACTCCAAATATCCACTTGTAGATTCTATAAAAAGGAATGTT
CAAAATTGCTCAATAAAAATAAAGTTTCAACACCGTGAGATGAGTGCACAAATCACAAAGGAGTTTCTCAAAA
TGCTTCTGGGTAGTTTTTCTGTGAA

$w11(170)$
GATAGTTCCTTTTCTACCATGGGCCACAAAGGGCTCCAAATACCCACTTGCAGATTCTACAAAAAGAGAGTTT
CACAACTGCTCTATCAAACAATATGTTCAACTTTGTGGGTTGAACACAAATATCACAAGAATTTTCTCCCAAT
GCTTCTGTGTAGTTTTTATGTGAA

$w12(171)$
GACATTTCTTTTCCCTCCATAGTCCACAAAGTGCTCCAAATATCCACTTACATATTCTAGAAAAAGATTGCTT

GGAAACTGCACAATGAAAAGAAAGGTTCAAATATATGAGATGAATGCACACATCACAAAGAAGTTTCTCAGAA
TCTCTCTGTGTAATTTTTATGTGAA

$w13(170)$
GATATTTCCTTTCCCACCTTAGGTCTTAAAACGCTCCAAATATCCACTTGCAGATACTACAAGAAGATTGTTT
CAAAACTGCACAAAAAAAGAAATGTTCAATTCTGTTTGATGAATGCACACATCACAAAGAAGTTTCTCAGAAT
GCTTCTCTGTAGTTTTTATGTGAA

$w14(170)$
GATATTTCCTTTTCCACAATAGGCCTCAAAGGGCTCCAAATATCCACTTCCAGATTCTATGAAAAGAATATTT
CCAAACTGCTCAATCATAGGAAATGTTCAACTCTGTGAGATGAATGCACACATCACAAGAAATTTCTCAGAAT
CCTTCAGTGTAGGTTTTATGAGAA

$w15(171)$
GATAATTCCTTTTCCACAATAGTTCTCAAAGCACTCAAAATATCCACTTGCAGATTCTACAAAAGGAGTATTT
CAAAACTGCTCAATCAAAAGAAAGGTTCAACTCTGTGAGATGAATGGACACATCACAAAGAAGTTTCTCAGAA
TGCTTCTGTGTAGTATTTTTGTGAA

$w16(170)$
GATATTTCTTTTCCACCATAGACCGCCAGGGGACACAAATATCCACTTTCAGATTCTACAACAAGAGAGGTTC
AAAACTACTCGATCAAGAGATGGTTTCAACTATGTGAGTTGAATGCACACATCACAAAGAACTATGTCGGAAT
TCTTCTGTGTAGTATTTATGTGAA

$w17(171)$
GATATTTCCTTTTCCACAATAGACGTCAAAGTGATCCAGATATCCACTTGCAGATTCCACAAAAAGAGTGTTT
CAAAAGTGCACAACCAAAAGAAAGGTTCAACTAGGTGAGATGAATGCACACATCAGAAGGAAGTTTCTCAGAA
TGCTTCTGCATAGCTTTTAAGGGAA

$w18(171)$
GATACTTCCTTTTCCAACATAGGCCTCAAAGCACTCCAAATATCCTCCTGGAGATACCACAAAAAGAGTGTTT
GCAAACTGCTCAATCAAAAGAAAGATTTAACTCTGTGAGATGAATCCACACATGACAAAGAAGTTTCTCAGAA
TGCTTCTGTGTAGTTTTTATGTGAA

$w19(170)$
GATATTTCCTTTTCCACAATAAGACCCAAAAGGCTCCAAATATTCACTTGCAGATTCTAAAAAAAACAGTGTT
TCAAAACTGCTCAATCAAAAGATAGTTCACTCTGTGAGAAGAATGCTCACATCACTGAGAAGTTTCTCAGAAT
GCTTCTGTGTAGTTTTTATGTGAA

$w20(104)$
GATATT--------------------------------CTATAATTTATGAGATTCATACAAA----------
-------------------------TTCAACTCTGTGAGAAGAATGCTCACATCACTGAGAAGTTTCTCAGAA
TGCTTCTGTGTAGTTTTTATATGAA

$w21(171)$
GATATTTCCTTTCCCACCGTAGGCCACAAAAGGCTCCAAATATCCACTTGCAGATACTATGAAAAGAGAGTTT
CAAAACTGCTCATTCAAAAGATAGGTTCAACTCTGTGGTTTGAATGCACACAGCACAAAGAAGTTTCACAGAA
TGTGTCTGTGTAGTTTTTATGTGCG

$w22(168)$
GATGTTTCCTTTTCCACCATATGCCTAAATATTTCCCAATTTCCACTTGCAGATTCCACAAGAAGAGTGTTTC
AAAACTGCTGTATCAAATAAAGTTGAACTCTGTGAGGTGAATGCACACAGCACAAAATGGTTTCTCAGAATGC
TTCCTTGTTGTTTTTATATGAA

$w23(167)$
GATGTTTCCTTTTCAACAATAGGCCTCAAAGTGCTTCAAATGTCCACTTGCAGATTCTACAAAAAGAGTGTTT
CAAAACTGCTCAATCAAAAGAAAGGTTCGACTCTGGGAAATTAATGCACACATCACAAAGAAGTTTCTCAGCT
TCTGTGTAGTTTTCATGTGAA

$w24(171)$
GTTATTTCCTTTTCCACAATAGGCCGCAAAGGGCTCCAAATATCAACTTACAGATTCTAGGAAAAGAGAGTTT
CAAAACTGCTCTACGAAAAGATAGGTTGAACTCTGTGAGATGAATGCACACATCACAAAGAAGTTTCTCAGAA
TGCATCTGTGTAGTTTTTACGGGAA

*w*25(171)
GACATTTCCTTTTCCACCATCTTCCACAAAGGTCTCCAAGTAACCACTTGCAGATTCTACAGAAAGACACTTT
AAAAACTGCTCTATCAAAAGATCAGTTCAAGTCTGTGGTTTGAATGCACACATCACAAAGAATTTTCTCAGAA
TGGTTCTGTGTAGTTTTCATATGAA

*w*26(171)
GATATTTCCTTTTCCACCATAGGCCTCAAAGCACTCCAAATATCCACTTGCAGATTCTACAAAAAGAGATTTT
CAAAACTAGTCAATCAAAAGAAAGGTTCAACTCTGTCAGTTGAATGCACATATCACAAACAAGTTTCTCGGAA
TGCGTCTGTGTAGTTTTTATGTGAA

*w*27(170)
GATATTTCCTTCTCCACAACAGGCCTCAAAGTGCTCCGAATATCCACTTGCAGATTTTACTAAAGAGTGTTTC
CAAACTGCTCAATCAAGAGGAAGTTTCAAGTCTGTGAGCTGAACGCACACATCACAAAGTAGTTTCTGAGAAT
GCTTCTGTGTAGTTTTTATGTGAA

*w*28(171)
GATGTTTCCTTTTCCACCATAGGCTGCAAAGGGCTCCAAATATCCACTTGCAGATTCTACAAAAAGAGAGTTT
CAAAAGTGCTCTATCAAAAGATAGGTTCAACTATGTGATATGAATGCACACATCACAAAGTAGTTTCTCAGAA
TGCTTCTGTGTAGTTTTTATGTAAA

*w*29(171 + insertion 53)
GATATTTCCTTTTCCACCATAGGCCTCAAAGCACTCCAAATATCCACTTGCAGATTCTACAAAAAGAGATTTT
CAAAACTATTTAATCAAAAGAAAGGTTCAAATCTGTCAGTTGAAGGTACATATCACAAACAAGTTTATTGGAA
TGCTTCTGTGTAGTTTTTATGTGAA
53–bp nonalphoid insertion after the base C at position 57:
*TACAAATTAAATGTATTTTTTACACCAAGTCTTTTAAGTTCAAGCACATGCAA*

*w*30(171)
GATATTTCCTTTTCCACAACAGGCCTCAAGGTGCTCCAAATATCCACTTGCAGATTTCACTAAAAGTGTGTTT
CCAAGCTGCTCAATCAAGAGGAAGTTTCAAGTCTGTGAGGTGAATGCACACATTACAAAGAAGTTACTGAGAA
TGCTTCTGTGTAGTTTTTATGTGAA

*w*31(170)
GATATTTCCTTTTCCACCACAGGCCTCAAAGCGCTGCAAATATCCACTTGCAGATTCTACAAAAAGAGAGTTT
CAAAACTGCTGTATCAAAAGATAGGGTCAACTCTGCGAGTTGAATAAACACATCACAAATAAGTTTCTGGGAA
CGCTTCTGTATAGTTTTATGTGAA

*w*32(170)
TATATTTCCTTTTCCACCATATGCCTCAAAGCACTCCAAATATCCACTTGCACATTATAGAAACATAGTCTTT
CAAAACTTGTCAATCAAAGAAAGGTTCAACTCCGTGAGATGAGTGCACACATCACAGAGAAGTTTCTCGGAAT
GTTTCTGTGTAGTTTTTATGTGAA

*w*33(171)
GATATTGCCTTTTCCACAATAGGCCTCAAAGCGTTCCAAATATCCAATTGCAGATTCCACAAAAAAAGTTTTT
TAAAACTGCTCAATCAAATGATAGATTAAACTCTGTGAGATTAGTGCACACATGTCAAAAAAGTTTCTCAGAA
TGCTTCTGTGTACTTTTTAGGGGAA

*w*34(171)
GATATTTCCTTTTCCACCATCGGCCACAAAGGACTCCAAATAACCACATGCAGATTCTAGTAACACAGAGTTT
CAAAACTGCTCTATCAAAAGATAAGTTCAACTCTGAGAGTTTAGTGCAACCATCGTGAAGAAGTTTCTCAGAA
TGCTTCTGAGTAGTGTTTATGTGAA

*w*35(170)
GATATTTCCTTTTCCACCATAGGCCTGAAAGCCCTCCAAATATCCACTTGCAGATCCTACAAAAAGAAAGTTT
CGAAATGCTCTCTCAAACGATAGTTTCGACTCTGTGGTATGAATACACACATCACAAAGAAGTTTCTCAGAAT
GCTTCTGTGTAGTTTTTAAATGAA

**Supplementary table** IV: Alignment of shifted consensus human alpha monomers, denoted $\{n\}$, (corresponding to peripheral HORs) and of human monomers $\{w\}$ from Supplementary table 3 (corresponding to internal HORs). Shifted monomers $\{n\}$ are defined by a shift of monomers $\{m\}$ from Supplementary Table 1. Here, $m44(\ldots 113)$ denotes the subsequence consisting of the last 113 bases in monomer $m44$, $m45(056\ldots)$ denotes the subsequence consisting of the first 56 bases from monomer $m45$, etc. Notation $n01(169)$ denotes the monomer $n01$ of length 169 bp, $w01(169)$ denotes the monomer $w01$ of length 169, etc. Underbar: single base substitution. Italics: 53–bp insertion in $w29(170) + \text{ins.}(053)$ with respect to the corresponding monomer $m37$. Notations $S$, $I$ and $D$ denote the number of base substitutions, insertions and deletions, respectively, in each of monomers in $\{w\}$ with respect to the corresponding monomers in $\{n\}$.

$n01(169) = m44(...113) + m45(056\ldots)$
GATATTTCTTTTTCCACCATAGGCCTCAAAGCACTCCAAATATGCACTTCCAGATTCTACAAAAAGAGTGTTT
CAGAACTGCTCAATCAAAAGGAAGGTTCCAGTCTGAGACAAATACACACATCAAAAGGTAGTTTCTCAGAATG
CTTCTGTGTAGTTTTTATGTGAA
$w01(169)$
GATATTTCTTTTTCCACCATAGGCCTCAAAGCACTCCAAATATGCACTTCCAGATTCTACAAAAAGAGTGTTT
CAGAACTGCTCAATCAAAAGGAAGGTTCCAGTCTGAGACAAATACACACATCAAAAGGTAGTTTCTCAGAATG
CTTCTGTGTAGTTTTTATGTGAA
$S = 0, I = 0, D = 0$

$n02(166) = m45(...110) + m01(056\ldots)$
GATATTTTCCTTTCCACCATAGGCCACAAATGGCTCTAAATACCCACTTACATTTTCCACAAAAAGAGAGTTT
CAAAACTGCTCTACCAAAGGTAAGTTTAACGCTGTGAGTTAAGAACATCACAAAGAAGTTTCTCAGAATGCTT
CTGTGTAGTTCTTACGTAAA
$w02(166)$
GATATTTTCCTTTCCACCATAGGCCACAAATGGCTCTAAATACCCACTTACATTTTCCACAAAAAGAGAGTTT
CAAAACTGCTCTACCAAAGGTAAGTTTAACGCTGTGAGTTAAGAACATCACAAAGAAGTTTCTCAGAATGCTT
CTGTGTAGTTCTTACGTAAA
$S = 0, I = 0, D = 0$

$n03(171) = m01(...115) + m02(056\ldots)$
GATATTTCCTTTTACACAATAGGCAGAAAAGTGCTCCAAATATCCACTTGAAGATTCTACAAAAACCGTGTTT
CAAAACTGCCGAATCAAAAGAAAGGTTCAACTCTGTGAGATGAATGCACACATAACAAAGGAGTTTCTCAGAA
TGCTTCTGTGTAGCTTTTATATGAA
$w03(171)$
GATATTTCCTTTTACACAATAGGCAGAAAAGTGCTCCAAATATCCACTTGAAGATTCTACAAAAACCGTGTTT
CAAAACTGCCGAATCAAAAGAAAGGTTCAACTCTGTGAGATGAATGCACACATAACAAAGGAGTTTCTCAGAA
TGCTTCTGTGTAGCTTTTATATGAA
$S = 0, I = 0, D = 0$

$n04(171) = m02(...115) + m03(056\ldots)$
GACATTTAGTTTTCCACAACAGGCCTCAAAGCTCTCTCCATATCCACTTGCAGATTCTACCGAAAGAGTGCTT
CCAAACTGCTCAATCAAAAGAGACATTCAAATCTGTGAGGTGAATGCAGACATCGTAAAGAAGTTTCTCAGAA
TGCTTCTGTGTATTTTTTGTGTGAA
$w04(171)$
GACATTTAGTTTTCCACAACAGGCCTCAAAGCTCTCTCCATATCCACTTGCAGATTCTACCGAAAGAGTGCTT
CCAAACTGCTCAATCAAAAGAGACATTCAAATCTGTGAGGTGAATGCAGACATCGTAAAGAAGTTTCTCAGAA
TGCTTCTGTGTATTTTTTGTGTGAA
$S = 0, I = 0, D = 0$

$n05(167) = m03(...111) + m04(056\ldots)$
GTTATTCGTTTTTGCACCATAGGCCTCCAAGCGTTCTAAATATCCACTTCTAGATTCTACAAAAAGAGAGTTT
CAAAACTACTCAAACAAAAGGTTCAATTCTGTGAGTTGAAAGCAAACATCACAAAGAAGTTTCTCAGAATGCG
TCTGTGTAGTTTTGATGTGAA
$w05(167)$
GTTATTCGTTTTTGCACCATAGGCCTCCAAGCGTTCTAAATATCCACTTCTAGATTCTACAAAAAGAGAGTTT
CAAAACTACTCAAACAAAAGGTTCAATTCTGTGAGTTGAAAGCAAACATCACAAAGAAGTTTCTCAGAATGCG
TCTGTGTAGTTTTGATGTGAA
$S = 0, I = 0, D = 0$

$n06(168) = m04(...112) + m05(056\ldots)$
GATATTTCCTTTTCACAGTAGAATGCAAAGGGCTCCAAATATCCACTTGGAGATTCTACAAAAAGAGTTTCAA
AACCGCTCTGTCAAATGATAGGTTGAACTCCCGGAGGTGAATACACACATCACAAAGAGGTTTCTCAGCATGC
TTCTGTGTAGTTTTTATGTAAA
$w06(168)$
GATATTTCCTTTTCACAGTAGAATGCAAAGGGCTCCAAATATCCACTTGGAGATTCTACAAAAAGAGTTTCAA
AACCGCTCTGTCAAATGATAGGTTGAACTCCCGGAGGTGAATACACACATCACAAAGAGGTTTCTCAGCATGC
TTCTGTGTAGTTTTTATGTAAA
$S = 0, I = 0, D = 0$

$n07(171) = m05(...115) + m06(056\ldots)$
CATATTTCCGTTTCTATCATAGGCCTCAAAGTGCTCCAAATATTCACTTGTACATTCTACCAAACGAGTATTT
CAAAACTGCTCAATCAAATGGAAGGTTCAAAACCGTGACATGAATGCCCACATCACAAAGTAGTTTCTCAGAA
TGCTTCTGTGTAGTTTTTATGTGAA
$w07(171)$
CATATTTCCGTTTCTATCATAGGCCTCAAAGTGCTCCAAATATTCACTTGTACATTCTACCAAACGAGTATTT
CAAAACTGCTCAATCAAATGGAAGGTTCAAAACCGTGACATGAATGCCCACATCACAAAGTAGTTTCTCAGAA
TGCTTCTGTGTAGTTTTTATGTGAA
$S = 0, I = 0, D = 0$

$n08(172) = m06(...116) + m07(056\ldots)$
GATATTTCCTTTTCCACAACAGCGTGCAAAACGCTTCAAATATGCCCTTAGAGATTCCACAAAAAGAGTGTTT
CCAAACTACTCAAATCAAAAAATGATTTCAACTCTGTGAGATGAATGCACACATCACAAACTAGTTTCTCAGA
ATGTTTCTGCCTGGTTCTCATGCGAA
$w08(172)$
GATATTTCCTTTTCCACAACAGCGTGCAAAACGCTTCAAATATGCCCTTAGAGATTCCACAAAAAGAGTGTTT
CCAAACTACTCAAATCAAAAAATGATTTCAACTCTGTGAGATGAATGCACACATCACAAACTAGTTTCTCAGA
ATGTTTCTGCCTGGTTCTCATGCGAA
$S = 0, I = 0, D = 0$

$n09(170) = m07(...114) + m08(056\ldots)$
GATAGTTCCTTTTTCACCATAGGCCGCAATGTACTCCAAATATCCACCTGCAGATTCTACAAAAGTGAGTTTC
AAAACTGCTCTATCAAAAGATCAGTTCGTCTCTGTGAGTTGAATGCATACATCAAAAAGAAGCTTCTCAAAAT
GCTTCTGTGTGGTTTTTCGGTGAA
$w09(170)$
GATAGTTCCTTTTTCACCATAGGCCGCAATGTACTCCAAATATCCACCTGCAGATTCTACAAAAGTGAGTTTC
AAAACTGCTCTATCAAAAGATCAGTTCGTCTCTGTGAGTTGAATGCATACATCAAAAAGAAGCTTCTCAAAAT
GCTTCTGTGTGGTTTTTCGGTGAA
$S = 0, I = 0, D = 0$

$n10(171) = m08(...115) + m09(056\ldots)$
GATAGTTCTTTTTCTACCATAGGTCTCAAACCACTCCAAATATCCACTTGTAGATTCTATAAAAAGGAATGTT
CAAAATTGCTCAATAAAAATAAAGTTTCAACACCGTGAGATGAGTGCACAAATCACAAAGGAGTTTCTCAAAA
TGCTTCTGGGTAGTTTTTCTGTGAA
$w10(171)$
GATAGTTCTTTTTCTACCATAGGTCTCAAACCACTCCAAATATCCACTTGTAGATTCTATAAAAAGGAATGTT
CAAAATTGCTCAATAAAAATAAAGTTTCAACACCGTGAGATGAGTGCACAAATCACAAAGGAGTTTCTCAAAA
TGCTTCTGGGTAGTTTTTCTGTGAA
$S = 0, I = 0, D = 0$

$n11(170) = m09(...115) + m10(055\ldots)$
GATAGTTCCTTTTCTACCATGGGCCACAAAGGGCTCCAAATACCCACTTGCAGATTCTACAAAAAGAGAGTTT
CACAACTGCTCTATCAAACAATATGTTCAACTTTGTGGGTTGAACACAAATATCACAAGAATTTTCTCCCAAT
GCTTCTGTGTAGTTTTTATGTGAA
$w11(170)$
GATAGTTCCTTTTCTACCATGGGCCACAAAGGGCTCCAAATACCCACTTGCAGATTCTACAAAAAGAGAGTTT
CACAACTGCTCTATCAAACAATATGTTCAACTTTGTGGGTTGAACACAAATATCACAAGAATTTTCTCCCAAT
GCTTCTGTGTAGTTTTTATGTGAA
$S = 0, I = 0, D = 0$

$n12(171) = m10(...115) + m11(056\ldots)$
GACATTTCTTTTCCCTCCATAGTCCACAAAGTGCTCCAAATATCCACTTACATATTCTAGAAAAAGATTGCTT

GGAAACTGCACAATGAAAAGAAAGGTTCAAATATATGAGATGAATGCACACATCACAAAGAAGTTTCTCAGAA
TCTCTCTGTGTAATTTTTATGTGAA
$w12(171)$
GACATTTCTTTTCCCTCCATAGTCCACAAAGTGCTCCAAATATCCACTTACATATTCTAGAAAAAGATTGCTT
GGAAACTGCACAATGAAAAGAAAGGTTCAAATATATGAGATGAATGCACACATCACAAAGAAGTTTCTCAGAA
TCTCTCTGTGTAATTTTTATGTGAA
$S = 0, I = 0, D = 0$

$n13(170) = m11(...114) + m12(056\ldots)$
GATATTTCCTTTCCCACCTTAGGTCTTAAAACGCTCCAAATATCCACTTGCAGATACTACAAGAAGATTGTTT
CAAAACTGCACAAAAAAAGAAATGTTCAATTCTGTTTGATGAATGCACACATCACAAAGAAGTTTCTCAGAAT
GCTTCTCTGTAGTTTTTATGTGAA
$w13(170)$
GATATTTCCTTTCCCACCTTAGGTCTTAAAACGCTCCAAATATCCACTTGCAGATACTACAAGAAGATTGTTT
CAAAACTGCACAAAAAAAGAAATGTTCAATTCTGTTTGATGAATGCACACATCACAAAGAAGTTTCTCAGAAT
GCTTCTCTGTAGTTTTTATGTGAA
$S = 0, I = 0, D = 0$

$n14(170) = m12(...115) + m13(055\ldots)$
GATATTTCCTTTTCCACAATAGGCCTCAAAGGGCTCCAAATATCCACTTCCAGATTCTATGAAAAGAATATTT
CCAAACTGCTCAATCATAGGAAATGTTCAACTCTGTGAGATGAATGCACACATCACAAGAAATTTCTCAGAAT
CCTTCAGTGTAGGTTTTATGAGAA
$w14(170)$
GATATTTCCTTTTCCACAATAGGCCTCAAAGGGCTCCAAATATCCACTTCCAGATTCTATGAAAAGAATATTT
CCAAACTGCTCAATCATAGGAAATGTTCAACTCTGTGAGATGAATGCACACATCACAAGAAATTTCTCAGAAT
CCTTCAGTGTAGGTTTTATGAGAA
$S = 0, I = 0, D = 0$

$n15(171) = m13(...115) + m14(056\ldots)$
GATAATTCCTTTTCCACAATAGTTCTCAAAGCACTCAAAATATCCACTTGCAGATTCTACAAAAGGAGTATTT
CAAAACTGCTCAATCAAAAGAAAGGTTCAACTCTGTGAGATGAATGGACACATCACAAAGAAGTTTCTCAGAA
TGCTTCTGTGTAGTATTTTTGTGAA
$w15(171)$
GATAATTCCTTTTCCACAATAGTTCTCAAAGCACTCAAAATATCCACTTGCAGATTCTACAAAAGGAGTATTT
CAAAACTGCTCAATCAAAAGAAAGGTTCAACTCTGTGAGATGAATGGACACATCACAAAGAAGTTTCTCAGAA
TGCTTCTGTGTAGTATTTTTGTGAA
$S = 0, I = 0, D = 0$

$n16(170) = m14(...114) + m15(056\ldots)$
GATATTTCTTTTCCACCATAGACCGCCAGGGGACACAAATATCCACTTTCAGATTCTACAACAAGAGAGGTTC
AAAACTACTCGATCAAGAGATGGTTTCAACTATGTGAGTTGAATGCACACATCACAAAGAACTATGTCGGAAT
TCTTCTGTGTAGTTTTTATGTGAA
$w16(170)$
GATATTTCTTTTCCACCATAGACCGCCAGGGGACACAAATATCCACTTTCAGATTCTACAACAAGAGAGGTTC
AAAACTACTCGATCAAGAGATGGTTTCAACTATGTGAGTTGAATGCACACATCACAAAGAACTATGTCGGAAT
TCTTCTGTGTAGTATTTATGTGAA
$S = 1, I = 0, D = 0$

$n17(171) = m15(...115) + m16(056\ldots)$
GATATTTCCTTTTCCACAATAGACGTCAAAGTGATCCAGATATCCACTTGCAGATTCCACAAAAAGAGTGTTT
CAAAAGTGCACAACCAAAAGAAAGGTTCAACTAGGTGAGATGAATGCACACATCAGAAGGAAGTTTCTCAGAA
TGCTTCTGCATAGCTTTTAAGGGAA
$w17(171)$
GATATTTCCTTTTCCACAATAGACGTCAAAGTGATCCAGATATCCACTTGCAGATTCCACAAAAAGAGTGTTT
CAAAAGTGCACAACCAAAAGAAAGGTTCAACTAGGTGAGATGAATGCACACATCAGAAGGAAGTTTCTCAGAA
TGCTTCTGCATAGCTTTTAAGGGAA
$S = 0, I = 0, D = 0$

$n18(171) = m16(...115) + m17(056\ldots)$
GATACTTCCTTTTCCAACATAGGCCTCAAAGCACTCCAAATATCCTCCTGGAGATACCACAAAAAGAGTGTTT
GCAAACTGCTCAATCAAAAGAAAGATTTAACTCTGTGAGATGAATCCACACATGACAAAGAAGTTTCTCAGAA
TGCTTCTGTGTAGTTTTTATGTGAA

$w18(171)$
GATACTTCCTTTTCCAACATAGGCCTCAAAGCACTCCAAATATCCTCCTGGAGATACCACAAAAAGAGTGTTT
GCAAACTGCTCAATCAAAAGAAAGATTTAACTCTGTGAGATGAATCCACACATGACAAAGAAGTTTCTCAGAA
TGCTTCTGTGTAGTTTTTATGTGAA
$S = 0, I = 0, D = 0$

$n19(171) = m17(...115) + m18(056\ldots)$
GATATTTCCTTTTCCACAATAAGACCCAAAAGGCTCCAAATATTCACTTGCAGATTCTAAAAAAAACAGTGTT
TCAAAACTGCTCAATCAAAAGATAGTTCAACTCTGTGAGAAGAATGCTCACATCACTGAGAAGTTTCTCAGAA
TGCTTCTGTGTAGTTTTTATGTGAA
$w19(170)$
GATATTTCCTTTTCCACAATAAGACCCAAAAGGCTCCAAATATTCACTTGCAGATTCTAAAAAAAACAGTGTT
TCAAAACTGCTCAATCAAAAGATAGTTCA-CTCTGTGAGAAGAATGCTCACATCACTGAGAAGTTTCTCAGAA
TGCTTCTGTGTAGTTTTTATGTGAA
$S = 0, I = 0, D = 1$

$n20(172) = m18(...116) + m19(056\ldots)$
GATATTTCCTTTTCCACAATAAGACCCAAAAGGCTCCAAATATTCACTTGCAGATTCTAAAAAAAACAGTGTT
TCAAAACTGCTCAATCAAAAGAAAGGTTCAACTCTGTGAGAAGAATGCTCACATCACTGAGAAGTTTCTCAGA
ATGCTTCTGTGTAGTTTTTATATGAA
$w20(104)$
GATATT---------------------------------CTATAATTTATGAGATTCATACAAA---------
--------------------------TTCAACTCTGTGAGAAGAATGCTCACATCACTGAGAAGTTTCTCAGA
ATGCTTCTGTGTAGTTTTTATATGAA
$S = 11, I = 0, D = 68$

$n21(171) = m19(...115) + m20(056\ldots)$
GATATTTCCTTTCCCACCGTAGGCCACAAAAGGCTCCAAATATCCACTTGCAGATACTATGAAAAGAGAGTTT
CAAAACTGCTCATTCAAAAGATAGGTTCAACTCTGTGGTTTGAATGCACACAGCACAAAGAAGTTTCACAGAA
TGTGTCTGTGTAGTTTTTATGTGCG
$w21(171)$
GATATTTCCTTTCCCACCGTAGGCCACAAAAGGCTCCAAATATCCACTTGCAGATACTATGAAAAGAGAGTTT
CAAAACTGCTCATTCAAAAGATAGGTTCAACTCTGTGGTTTGAATGCACACAGCACAAAGAAGTTTCACAGAA
TGTGTCTGTGTAGTTTTTATGTGCG
$S = 0, I = 0, D = 0$

$n22(168) = m20(...112) + m21(056\ldots)$
GATGTTTCCTTTTCCACCATATGCCTAAATATTTCCCAATTTCCACTTGCAGATTCCACAAGAAGAGTGTTTC
AAAACTGCTGTATCAAATAAAGTTGAACTCTGTGAGGTGAATGCACACAGCACAAAATGGTTTCTCAGAATGC
TTCCTTGTTGTTTTTATATGAA
$w22(168)$
GATGTTTCCTTTTCCACCATATGCCTAAATATTTCCCAATTTCCACTTGCAGATTCCACAAGAAGAGTGTTTC
AAAACTGCTGTATCAAATAAAGTTGAACTCTGTGAGGTGAATGCACACAGCACAAAATGGTTTCTCAGAATGC
TTCCTTGTTGTTTTTATATGAA
$S = 0, I = 0, D = 0$

$n23(167) = m21(...115) + m22(052\ldots)$
GATGTTTCCTTTTCAACAATAGGCCTCAAAGTGCTTCAAATGTCCACTTGCAGATTCTACAAAAAGAGTGTTT
CAAAACTGCTCAATCAAAAGAAAGGTTCGACTCTGGGAAATTAATGCACACATCACAAAGAAGTTTCTCAGCT
TCTGTGTAGTTTTCATGTGAA
$w23(167)$
GATGTTTCCTTTTCAACAATAGGCCTCAAAGTGCTTCAAATGTCCACTTGCAGATTCTACAAAAAGAGTGTTT
CAAAACTGCTCAATCAAAAGAAAGGTTCGACTCTGGGAAATTAATGCACACATCACAAAGAAGTTTCTCAGCT
TCTGTGTAGTTTTCATGTGAA
$S = 0, I = 0, D = 0$

$n24(171) = m22(...115) + m23(056\ldots)$
GTTATTTCCTTTTCCACAATAGGCCGCAAAGGGCTCCAAATATCAACTTACAGATTCTAGGAAAAGAGAGTTT
CAAAACTGCTCTACGAAAAGATAGGTTGAACTCTGTGAGATGAATGCACACATCACAAAGAAGTTTCTCAGAA
TGCATCTGTGTAGTTTTTACGGGAA
$w24(171)$
GTTATTTCCTTTTCCACAATAGGCCGCAAAGGGCTCCAAATATCAACTTACAGATTCTAGGAAAAGAGAGTTT

CAAAACTGCTCTACGAAAAGATAGGTTGAACTCTGTGAGATGAATGCACACATCACAAAGAAGTTTCTCAGAA
TGCATCTGTGTAGTTTTTACGGGAA
$S = 0, I = 0, D = 0$

$n25(171) = m23(...115) + m24(056\ldots)$
GATATTTCCTTTTCCACCATCTTCCACAAAGGTCTCCAAGTAACCACTTGCAGATTCTACAGAAAGACACTTT
AAAAACTGCTCTATCAAAAGATCAGTTCAAGTCTGTGGTTTGAATGCACACATCACAAAGAATTTTCTCAGAA
TGCTTCTGTGTAGTTTTCATATGAA
$w25(171)$
GACATTTCCTTTTCCACCATCTTCCACAAAGGTCTCCAAGTAACCACTTGCAGATTCTACAGAAAGACACTTT
AAAAACTGCTCTATCAAAAGATCAGTTCAAGTCTGTGGTTTGAATGCACACATCACAAAGAATTTTCTCAGAA
TGGTTCTGTGTAGTTTTCATATGAA
$S = 2, I = 0, D = 0$

$n26(171) = m24(...115) + m25(056\ldots)$
GATATTTTCTTTTCCACCATAGGCCTCAAAGTGCTCCAAATATCCACTTGCAGATTCTACAAAAAGAGTGTTT
CAAAACTGCTCAATCAAAAGAAAGGTACAACTCTTTGTGATGAATTCACTAATAACAAAGACGTTTCTCACAA
TGCTTCTCTGTAGTTTTTATGTGAA

$n27(171) = m25(...115) + m26(056\ldots)$
GATCTTTCCTTTTCTACCATAGGCATCAAAGCACTACAAATATCCAATAGCAGATTCTACAAAAAGAGTGTTT
CAAAACTGCTCAATCAAATGAAACGTTCAACCCTGTGAGATGAATGCAGACATTAAAAGATAGTTTCTCATTA
TGGTTCTGGGTAGTTTTTATGTGAA

$n28(168) = m26(...113) + m27(055\ldots)$
CTTATTTCCTTTTCCAAAATAGGCCGGAAAGGGCTCCAAGTATCCACTTGCAGATTCTACAAAAAGAGATTCA
AAACTCCTCAATCAAAAGATAGGTTGAACTCCGTGAGATTAATGCATACATCACAACGAAGTTTCTCAGAGGG
CTTCATTGTAGTTTTATGGGAA

$n29(172) = m27(...116) + m28(056\ldots)$
GATATTTCCTTTTCCACTATATGTCTCAAAGATATCCAAATATACACTTGCAGATTCTACAAAATGAGAGTTT
CAAAACTGCTCTGTCAAAAAAAGAGGTTCAGCTGCATGAGTTGAATGCACACATCACAAAGAAGTTTCTCAGA
ATGCTTCTGTGTATTTTTTATGTTAA

$n30(171) = m28(...115) + m29(056\ldots)$
GATATTTTCTTTTCCACCATAGGCTGCAAAGGGCTCCAAATATCCACTTGCAGATTCTACAAAAAGAGATTTT
CAAAACTGCTCAATCAAAAGAAAGGCTCAACTCTGTGAGATGAATGCACACAAAACAAAGGAGTTTCTGCAAA
TGCTTCTGTGTAGTTTTTAAGTGAA

$n31(171) = m29(...115) + m30(056\ldots)$
GATACTTCCTTTTCCACAATAGGTCTCGAAGCCCTCCAAATATCCAAATGTGGATTCTACAAAAAGAGTGTTT
CAAAACTGCTCAATCAAATGGAAGCTTCAACTCTAAGAAATGAATACACACCTGACAAAGAAGTTTCTCAGAA
TGATTTTGTGTAGTTTTTTGGGGAA

$n32(171) = m30(...115) + m31(056\ldots)$
GGCGTTTTCCTTTCCACCATCGGTCACAAAGGCCTCCAAATAACCACATGCAGATTCTACACAAGGAGAGTTT
CAAAACTGCTCTGTCAAAAGATAGGTTCAGCTCTGCGAGTTGAATGCACACATCACAGACAAGTTTCTCAGAA
TGCTTCTGTGTAGTTTTCATGTGAA

$n33(171) = m31(...115) + m32(056\ldots)$
GATATTTCCTTTTCCACTTTAGGCCACAAAGCACTCCAAATATCCACTTGCAGAAACTACAAAAAGAGTCTTT
CAAAACTGCTCAAGCAAAAGAAAAGTTCAACTCTGTGAGATGAATGCACACATCACAAAGGAGTTTCTGAGAA
TGCTTCTGTGTAGTTTTTATGTGAA

$n34(169) = m32(...114) + m33(055\ldots)$
ATATTTCCTTATCCACCATAGGCTTCAAAGTGCTCCAAATATTCACTTGCAAATTATAAAAACAGAATTTTTC
AAAAATGCTCAGTTAAAAGAATGTTTCAACACTGTGAGATGAATGCACACATCACAAAAAGTTTCTGGGAATG
CTTCTGTGTGGTTTTTATGTGAG

$n35(170) = m33(...114) + m34(056\ldots)$
GATATTTCCTTTTCCACCATAGACTACAAAGGGCTCCAAATATCCACTTGCAGATTCTACAAAAAGAGAGTTT
CGAAATGCTCTATCAAAAGATAGGTTCAAATATGTGATATGAATGCACACATCACAAAGAATTTTCTCAGAAT

GCTTCTGTGTAGTTTTCATATGAA

$n36(171) = m34(...115) + m35(056\ldots)$
GATATTTCCTTTTCCACCATAGGCCTCAAAGCACTCCAAATATCCACTTGCAGATTCTACAAAAAGAGATTTT
CAAAACTAGTCAATCAAAAGAAAGGTTCAACTCTGTCAGTTGAATGCACATATCACAAACAAGTTTCTCGGAA
TGCGTCTGTGTAGTTTTTATGTGAA
$w26(171)$
GATATTTCCTTTTCCACCATAGGCCTCAAAGCACTCCAAATATCCACTTGCAGATTCTACAAAAAGAGATTTT
CAAAACTAGTCAATCAAAAGAAAGGTTCAACTCTGTCAGTTGAATGCACATATCACAAACAAGTTTCTCGGAA
TGCGTCTGTGTAGTTTTTATGTGAA
$S = 0, I = 0, D = 0$

$n37(170) = m35(...114) + m36(056\ldots)$
GATATTTCCTTCTCCACAACAGGCCTCAAAGTGCTCCGAATATCCACTTGCAGATTTTACTAAAGAGTGTTTC
CAAACTGCTCAATCAAGAGGAAGTTTCAAGTCTGTGAGCTGAACGCACACATCACAAAGTAGTTTCTGAGAAT
GCTTCTGTGTAGTTTTTATGTGAA
$w27(170)$
GATATTTCCTTCTCCACAACAGGCCTCAAAGTGCTCCGAATATCCACTTGCAGATTTTACTAAAGAGTGTTTC
CAAACTGCTCAATCAAGAGGAAGTTTCAAGTCTGTGAGCTGAACGCACACATCACAAAGTAGTTTCTGAGAAT
GCTTCTGTGTAGTTTTTATGTGAA
$S = 0, I = 0, D = 0$

$n38(171) = m36(...115) + m37(056\ldots)$
GATGTTTCCTTTTCCACCATAGGCTGCAAAGGGCTCCAAATATCCACTTGCAGATTCTACAAAAAGAGAGTTT
CAAAAGTGCTCTATCAAAAGATAGGTTCAACTATGTGATATGAATGCACACATCACAAAGTAGTTTCTCAGAA
TGCTTCTGTGTAGTTTTTATGTAAA
$w28(171)$
GATGTTTCCTTTTCCACCATAGGCTGCAAAGGGCTCCAAATATCCACTTGCAGATTCTACAAAAAGAGAGTTT
CAAAAGTGCTCTATCAAAAGATAGGTTCAACTATGTGATATGAATGCACACATCACAAAGTAGTTTCTCAGAA
TGCTTCTGTGTAGTTTTTATGTAAA
$S = 0, I = 0, D = 0$

$n39(171) = m37(...115) + m38(056\ldots)$
GATATTTCCTTTTCCACCATAGGCCTCAAAGCACTCCAAATATCCACTTGCAGATTCTACAAAAAGAGATTTT
CAAAACTATTTAATCAAAAGAAAGGTTCAAATCTGTCAGTTGAAGGTACATATCACAAACAAGTTTATTGGAA
TGCTTCTGTGTAGTTTTTATGTGAA
$w29(171 + \mathrm{insertion}53)$
GATATTTCCTTTTCCACCATAGGCCTCAAAGCACTCCAAATATCCACTTGCAGATTC̃TACAAAAAGAGATTTT
CAAAACTATTTAATCAAAAGAAAGGTTCAAATCTGTCAGTTGAAGGTACATATCACAAACAAGTTTATTGGAA
TGCTTCTGTGTAGTTTTTATGTGAA
53-bp insertion after C̃ at position 57:
*TACAAATTAAATGTATTTTTTACACCAAGTCTTTTAAGTTCAAGCACATGCAA*
$S = 0, I = 53, D = 0$

$n40(171) = m38(...115) + m39(056\ldots)$
GATATTTCCTTTTCCACAACAGGCCTCAAGGTGCTCCAAATATCCACTTGCAGATTTCACTAAAAGTGTGTTT
CCAAGCTGCTCAATCAAGAGGAAGTTTCAAGTCTGTGAGGTGAATGCACACATTACAAAGAAGTTACTGAGAA
TGCTTCTGTGTAGTTTTTATGTGAA
$w30(171)$
GATATTTCCTTTTCCACAACAGGCCTCAAGGTGCTCCAAATATCCACTTGCAGATTTCACTAAAAGTGTGTTT
CCAAGCTGCTCAATCAAGAGGAAGTTTCAAGTCTGTGAGGTGAATGCACACATTACAAAGAAGTTACTGAGAA
TGCTTCTGTGTAGTTTTTATGTGAA
$S = 0, I = 0, D = 0$

$n41(170) = m39(...115) + m40(055\ldots)$
GATATTTCCTTTTCCACCGCAGGCCTCAAAGCGCTGCAAATATCCACTTGCAGATTCTACAAAAAGAGAGTTT
CAAAACTGCTGTATCAAAAGATAGGGTCAACTCTGCGAGTTGAATAAACACATCACAAATAAGTTTCTGGGAA
CGCTTCTGTATAGTTTTATGTGAA
$w31(170)$
GATATTTCCTTTTCCACCACAGGCCTCAAAGCGCTGCAAATATCCACTTGCAGATTCTACAAAAAGAGAGTTT
CAAAACTGCTGTATCAAAAGATAGGGTCAACTCTGCGAGTTGAATAAACACATCACAAATAAGTTTCTGGGAA
CGCTTCTGTATAGTTTTATGTGAA

$S = 1, I = 0, D = 0$

$n42(170) = m40(...114) + m41(056\ldots)$
TATATTTCCTTTTCCACCATATGCCTCAAAGCACTCCAAATATCCACTTGCACATTATAGAAACATAGTCTTT
CAAAACTTGTCAATCAAAGAAAGGTTCAACTCCGTGAGATGAGTGCACACATCACAGAGAAGTTTCTCGGAAT
GTTTCTGTGTAGTTTTTATGTGAA
$w32(170)$
TATATTTCCTTTTCCACCATATGCCTCAAAGCACTCCAAATATCCACTTGCACATTATAGAAACATAGTCTTT
CAAAACTTGTCAATCAAAGAAAGGTTCAACTCCGTGAGATGAGTGCACACATCACAGAGAAGTTTCTCGGAAT
GTTTCTGTGTAGTTTTTATGTGAA
$S = 0, I = 0, D = 0$

$n43(171) = m41(...115) + m42(056\ldots)$
GATATTGCCTTTTCCACAATAGGCCTCAAAGCGTTCCAAATATCCAATTGCAGATTCCACAAAAAAAAGTTTTT
TAAAACTGCTCAATCAAATGATAGATTAAACTCTGTGAGATTAGTGCACACATGTCAAAAAAGTTTCTCAGAA
TGCTTCTGTGTACTTTTTAGGGGAA
$w33(171)$
GATATTGCCTTTTCCACAATAGGCCTCAAAGCGTTCCAAATATCCAATTGCAGATTCCACAAAAAAAAGTTTTT
TAAAACTGCTCAATCAAATGATAGATTAAACTCTGTGAGATTAGTGCACACATGTCAAAAAAGTTTCTCAGAA
TGCTTCTGTGTACTTTTTAGGGGAA
$S = 0, I = 0, D = 0$

$n44(171) = m42(...115) + m43(056\ldots)$
GATATTTCCTTTTCCACCATCGGCCACAAAGGACTCCAAATAACCACATGCAGATTCTAGTAACACAGAGTTT
CAAAACTGCTCTATCAAAAGATAAGTTCAACTCTGAGAGTTTAGTGCAACCATCGTGAAGAAGTTTCTCAGAA
TGCTTCTGAGTAGTGTTTATGTGAA
$w34(171)$
GATATTTCCTTTTCCACCATCGGCCACAAAGGACTCCAAATAACCACATGCAGATTCTAGTAACACAGAGTTT
CAAAACTGCTCTATCAAAAGATAAGTTCAACTCTGAGAGTTTAGTGCAACCATCGTGAAGAAGTTTCTCAGAA
TGCTTCTGAGTAGTGTTTATGTGAA
$S = 0, I = 0, D = 0$

$n45(170) = m43(...114) + m44(056\ldots)$
GATATTTCCTTTTCCACCATAGGCCTGAAAGCCCTCCAAATATCCACTTGCAGATCCTACAAAAAGAAAGTTT
CGAAATGCTCTCTCAAACGATAGTTTCGACTCTGTGGTATGAATACACACATCACAAAGAAGTTTCTCAGAAT
GCTTCTGTGTAGTTTTTAAATGAA
$w35(170)$
GATATTTCCTTTTCCACCATAGGCCTGAAAGCCCTCCAAATATCCACTTGCAGATCCTACAAAAAGAAAGTTT
CGAAATGCTCTCTCAAACGATAGTTTCGACTCTGTGGTATGAATACACACATCACAAAGAAGTTTCTCAGAAT
GCTTCTGTGTAGTTTTTAAATGAA
$S = 0, I = 0, D = 0$

**Supplementary table** V: Detailed monomer structure of chimpanzee alphoid HOR copies in contig NW_001252921.1 which corresponds to Fig. 4.

| Segment | Position | Length (bp) | Composition | No.pJ$\alpha$ | Divergence (%) |
|---|---|---|---|---|---|
| 30 mon. | 264 | 5061 | $e01, ..., e30$ | 11 | 0,8 |
| 11 mon. | 5325 | 1868 | $e01, ..., e11$ | 4 | 0,6 |
| 16 mon. | 7193 | 2683 | $e13, ..., e28$ | 8 | 1,0 |
| 7 mon. | 9876 | 1198 | $e05, ..., e11$ | 3 | 0,9 |
| 18 mon. | 11074 | 3028 | $e13, ..., e30$ | 7 | 0,8 |
| 11 mon. | 14102 | 1872 | $e01, ..., e11$ | 4 | 0,4 |
| 18 mon. | 15974 | 3023 | $e13, ..., e30$ | 8 | 0,3 |
| 6 mon | 18997 | 1022 | $e01, ..., e06$ | 1 | 0,5 |
| C01 | 2019 | 599 | | | |
| 13 mon. | 20618 | 2210 | $e13, ..., e01$ | 5 | 0,9 |
| 18 mon. | 22828 | 3030 | $e30, ..., e13$ | 9 | 0,5 |
| 11 mon. | 25858 | 1865 | $e11, ..., e01$ | 4 | 1,0 |
| 18 mon. | 27723 | 3029 | $e30, ..., e13$ | 9 | 0,4 |
| 7 mon. | 30752 | 1189 | $e11, ..., e05$ | 3 | 1,1 |
| 8 mon. | 31941 | 1310 | $e28, ..., e21$ | 3 | 0,7 |
| C02 | 33251 | 41 | | | |
| 20 mon. | 33292 | 3416 | $e20, ..., e01$ | 8 | 2,4 |
| 18 mon. | 36708 | 3026 | $e30, ..., e13$ | 9 | 0,6 |
| 11 mon. | 39734 | 1870 | $e11, ..., e01$ | 3 | 3,4 |
| 5 mon. | 41604 | 855 | $e30, ..., e26$ | 2 | 5,5 |

For comparison see Supplementary table 1.

**Supplementary table** VI: Chimpanzee alpha monomers, denoted $e01, ..., e30$, in consensus alphoid 30mer (5,066 bp) determined by GRM analysis of genomic sequence of chromosome Y (contig NW_001252921.1). In parentheses: lengths of monomers (in bp).

$e01$(171)
TGACAAATTACTTTATGCTGTGTGCATTGATCTCACAGAGTTGAACATTTCTTTTCATTGACCAGTTTTGAAA
CACTGTTTTAGTAGAATCTGGAAGTGGACATTTGGAGCACCTTGGGGCCTGTGGTGGAAAAGGAAATCCCTTC
ACATAAAAACTAGACAGAAGCATTT

$e02$(170)
TGACAAACTCCTTTGGATGTGTGCATGCATCTCATGGCGTGGAATATTTCTGTTGATTGAGCAGCTTTGAAAC
ACTCTTTTCCTAGAATCTTCAAGGGGACATTTGGAGCAATTTCAGGCCTATGGTTCAATAGGAAATATCTTCA
CATAAAAACTAGACAGAAGCATAC

$e03$(171)
TGACAAACTTCTCTGTGATGTGTGCATACATCTCAGAGAGTTGAACATTTCTTTTGATAGACCAGCTTTGAAA
CACTCCATTTGTAGAATGTGGGAGTGGACATTTGGAGTGCTTTGAGGCTTATGGTAGAAAGGGAAATATCTTC
ATATAAAAACTAGACAGAAGCATTC

$e04$(167)
TGAAAAACTTCTTTGTGATATGTGCATTCATGTCAAAGAGTTGAACTTTTCTTTTGATTGAACAGTCATGAAA
CTCTCTGTAGAATCTGCAAACGGACATTTGTTGTGCTTTGAGGCCTATGGTGGAAAAGAAAATATCTTCACAT
AAATACTAGTCAGAAGCATTC

$e05$(170)
TGAAAACTGTCTTTGTGATACGTGCATTCATCTCACAGAGTTGAACCTCACTTTTGATTGAGCAGTTTGAAAG
ACTTTTTTTGTACTATAGGAAAGTGGATAATTGGAGTGCTTTGAGGCCGATCATGGAAAATTAAATATCTTCA
CATAAGAACAAGACAGAAGCATTC

$e06$(171)
TGACAAATTTCTTTGTGATATGTGCATTCATCTCACAGAGTTGAACCTTAATTTTCATTGAGCAGTTTTGAAA
CACTCTTTTTGTAGAATCTGCAAGTAGTCATTTGGAGCGCTTTGAGGCCTTTGTTGGAAAACGAAATGTCTTC
ATATAATAACTAGACAGAAGCATTC

$e07$(171)
TGAGAAACTTATTTGTGATATCTGCACTCATCTCACAGAGTTGAATCTTTCCTTTGATGGAGCAGCTTTGAAA
CACTCTTTTCGTAGAATCTGCTAGTGGACCTTTGCAGCGCTTTGAGGCCTATGGTGGAAAAGGCAATATCTTC
ACATAAAAACTAGACAGAAGCATTC

$e08$(170)
TGACAAACTTGTTTGTGATGTGTGAATTTACTTCATAGATTTCAACTTTCTTGTGATTGAGCAGTTTTGAAAC
ACTCTTTTTGTGGAATCTGCAAGTGGACATTTGAAACGCTATGAAGCCTAAGGTGGAAAAGGAAATATCTTCA
CATAAAAATTAGACGGACGCATTT

$e09$(171)
TGACAAACTTCTTCGAGATGTGTGCATTCATCTCACAGAGTTGAACCTTTCTTTTGATTAAGCAATCTTGAAA
CACTCTATTTGTAGAATCTGCAAGTGGATATTTGTTGTGCTTTGAGGCCTACGGTGGAAAAGGAAATATCTTC
ACATAAAAACTTGACAGAAGCACTC

$e10$(171)
TGAGAGCCTCCTTTGGGATGTGTGAATTTATCTCTCAGACTTGACCCTTACTTTTGATTGAGCATCTTTGAAA
GACCACTTTTGTAATAAATGCAAGTGGACATTCGAAGTGCTTTGAGGCCTACGGTGGAAAAGAAAATATCTTC
ACATCAGAAGGAGACAGAAGCATTC

$e11$(169)
TGACCAATTTCTTTGTGGTGTGTGCATTAATCTCACAGAGTTAAACCTTACTTTCAATTGAGCCATTTTGAAA
CACTTTTCGTAGAATCTGCAAGTGGACATTTGAAGCGCTTTGAGGCCTAGGGTCGAAAAAGAAATATATTCAC
ATAAAAACTAGATGGAAGCCTTC

$e12$(171)
TGACAAACTTCTTTGTGATGTGTGCATTCATCTCACAGAGTTGATCCTTACTTTTCATTGAGCAGTTTTGAAA
CACTCTTTTTGTAGAATCTGCAGGTGGATATTTGGAGGGCTTTGAGGCCTAGGGTCGAAAAAGAAATATATTC

ACATAAAAACTAGATGGAAGCCTTC

$e13(171)$
TGACAAACTTCTTTCCGATGTGTGCATTCATCTCACAGAGTTGAACCTTTCTTTTGATTGAGCAGCTTTGAAA
CCCTCTTTTGGTAGAATTTGCATGTGAACATTTGAAGCGCTTTGAGGCCTGTGGAGGAAAAGGAAATATCTCC
ACCTAAAAACTAGACAGAAGCATTC

$e14(171)$
TGGCAAACTTCTTTGTGATGTGTGCATTCATCTCACAGAGTTGATCCTTACTTTTCATTGAGCAGTTTTGAAA
CACTCTTTTTGTAGAATCTGCAGGTGGATATTTGGAGGGCTTTGAGGCCTCTGGTGGATAACGAAATATCTTC
ACATAATAACTAGACAGAAGAATTC

$e15(171)$
TCACAAACTTCTTTGTAATGTGAGCATTCGTCTCACAGAGTTGAACTGTTCTTTTGACTGAGCAGCTTTGAAA
CAGTATTTTTATAAAATCTGCAAGTGGACATTTGGATCGCTTTGAGGCCTCTGGTGGAACAGGAAATAGCTTC
ACAATAAAACTGGAGAGAAGCGTTC

$e16(170)$
TGACAAACTTCTTTGTGATGTGTACATTCATCTCACAGAGTTGAACCTTGCTTTTGATTGAGCAGTTTTGAAA
CACACTTTTTGTAGAATTTGAAAGTGGACCTTTGGATTGCTTTGAGGCCTATGGTGGAAAAGGAAATATCTTC
ATAAAAGACTAGACAGAAGCATTG

$e17(171)$
CGACAAACTCCTTCGTGATGTGTGCATTCAACTCACAGAGTTGAACCTTTCTTTTGACTGAGCAACTTTGAAA
CACTCTATCTGTAGAATCTCCCAGTGGATATTTGCAGTGGCTTGAGGCCTCTGACGGAAAAGGAAATATCTTC
ACATAACGACTACACAGAAGCACTC

$e18(171)$
TGACAAACTATTTTGTGATGTGTGCATTCTTCTCACAGAGTTGAACCTTACTTTTCATTGAGGAATTTTTAAA
TACTCATTTTGTAGAATCTGCAAGATGACATTTGGAGCGCTTCAAGGCCTATGGTGGATAACGAAACGTCTTC
ATGTAATAACTAGGCAGAAGCATTA

$e19(176)$
TGAGAAACTCCAATGTGATGTGTGCTTTCGTATCACACAGAGTTTCACTTTTCTTTTGATTGAGCAGCTTTGA
AACATTCTTTTTGTAGAATCTGAAAGTGGATATTTGGAGCTCTTGGAGGCCTATGGTGGATAACGAAATGTCT
TCGTATAATAATAACTAGAGAGAAGCATTC

$e20(170)$
TGAGAAGCTTCTTTGTGACGTGAGAATTCATCTCACAGATTTGAACCTTCGTTTGATGGAGTAGCTTTGAAGC
ACTCTTTTTGTAGAATCTGCAAATGGACATTTGGAGCGGTTTGAGGCCTATAGTGGAAAAGGAATCGTCTTCA
CATAAAAAGGAGACAGAAGCATTC

$e21(171)$
TCACAACATACTTTGTGACATATGCATTCATCTCACAAAGCTGAACCTTACTTTTGATTGAGCAGTTTGGAAA
CCCCCTTTTTCTACTATCTGCAAGTGGACCTTTGGAGTGCTTTGAGGCCTATGGTGGAAAAGGAAATATCTTC
ACTTAAGAAGTAGACAGAAGGATTC

$e22(170)$
TGATAAATTTCTTTGTGATGTGTGCATTCATCTCACAGAGTTGAACCTTACTCTGGTTGAACAGTTTTGAAAC
ACTGTTTTCGTAGAATCTGCAAGTGGACATTTTGAGCGCTTGGAGGGCTATGGTGTTAAAGGAAATATCTTCC
CATAAGAACTAGACACAAGCATTC

$e23(171)$
TGACAAGCTTCTTTGTGATGTGTGCCTTCGTCTCACAGAGTTGAAACTATCTTTTGATTGAGCAGCTTTGAAA
CACTCTTTCTGTAGAATCTGCAAGTAGGCATTTGGAAGGTTTGGGGCCTGTGGTGGAAAAGGAAATATCTTCA
CACAAAAATGAGACAGAAGCCCTCG

$e24(170)$
GACAACCTTCTTTGTGATATGTGCACTTATCACACAGAGTGAAACCTTAGTGTTTATTGAGCAGTTTTGAAAC
ACCCTTTTTGAATGATCTGCATGTGGACATTTGGAGTGCTTTGAGGTCTACTGTGGCAAAGGAAATATCTTCA
CCTAAGAACTAGACAGAAGCATTC

*e*25(117)
```
GGAGAATTTTCTTGTGATATGTGTATTCATCTCACAGAGTTGAACCTTACTTTGGATTGACCAGTTTTGAAAC
AC-----------------------------------------------------GAAAAGGAAATATCTTCA
CATTAAAACTAGACAGAAGGATTT
```

*e*26(169)
```
TGACAAACTACTTTGTGATGTGTACATTCATCTCACAGAGTTGAACCTTACTTTCCATTGAGCAGTTTTGAAA
CCTTCCTCTGGGGAATCTGCAAGTGGATTTTTGGAGCACTTTGAGGCCTTTGCTGGAAAGGAAATACATTCAC
AAAAAACCTAGACAGAAGCATTC
```

*e*27(171)
```
TCACAAACTACTTTGGGATGCATGCATTCATCTCACGGGGCTGAACCTTGCTTTTCATTGAGTAGTTTTGAAA
CACTCTTTTGTAGCATCTGCAAGTGGACATTTCGAGTGCTCTGAGGCCTACGGTGGATAACGAAATATCTTCA
TATCACAGCTAGACAGAAGCTATCT
```

*e*28(171)
```
GAGAAGCTTTCTATGTGATGTGTGCATTCATCTCACAGAGTTGAACCTTACTTTTCATTGAACAGTTTTGAAA
CACTCTTTTGGCAGAATCTACAAGTGGACCTTTGGAACGCTTTGAGGCCTACGGTGGAAAAGGAAATATCTTC
ACATAAGAACTAGACAGAAGCATAC
```

*e*29(171)
```
TGACAAATTTCTTTTTCGTGTGCGCATTCATCTCACAGCGTTGAAAGTTAATTTTCATTGAGCAGTTATGAAA
CATACTTTTTGTGGAATCTGGATGACGACATTTGGAGCACTTTGAGGCCTATCACGGAAAGGGAAATATCTTC
ATATAAAAATTAGATGGAGGCATTC
```

*e*30(171)
```
TGAAAAACATCTTTGTGATGTGTGCATTCCTCTCACAGAGTTGAACCTTTCTTTTGATTGACCAGCTTCGAAA
TGCTCTTTTAGTAGAACCTGGAAGTGGACACTTGGAGCCTTTTGTGGCCTAATGCGGAAGAGGAAATATCTTC
ACGTAAAAAGTAGATAGAAGCATTC
```

**Supplementary table** VII: Divergence between human consensus alpha monomers $\{m\}$ (from Supplementary table 2) and reverse complement shifted chimpanzee monomers $\{\bar{e}\}$ (from Supplementary table 6).

| | $\bar{e}$01 | $\bar{e}$02 | $\bar{e}$03 | $\bar{e}$04 | $\bar{e}$05 | $\bar{e}$06 | $\bar{e}$07 | $\bar{e}$08 | $\bar{e}$09 | $\bar{e}$10 | $\bar{e}$11 | $\bar{e}$12 | $\bar{e}$13 | $\bar{e}$14 | $\bar{e}$15 | $\bar{e}$16 | $\bar{e}$17 | $\bar{e}$18 | $\bar{e}$19 | $\bar{e}$20 | $\bar{e}$21 | $\bar{e}$22 | $\bar{e}$23 | $\bar{e}$24 | $\bar{e}$25 | $\bar{e}$26 | $\bar{e}$27 | $\bar{e}$28 | $\bar{e}$29 | $\bar{e}$30 |
|---|---|---|---|---|---|---|---|---|---|---|---|---|---|---|---|---|---|---|---|---|---|---|---|---|---|---|---|---|---|---|
| $m01$ | 24 | 25 | 25 | 28 | 25 | 23 | 21 | 26 | 22 | 29 | 27 | 23 | 24 | 22 | 27 | 21 | 25 | 27 | 25 | 25 | 26 | 22 | 26 | 26 | 26 | 25 | 29 | 22 | 30 | 23 |
| $m02$ | 22 | 24 | 22 | 23 | 21 | 17 | 20 | 23 | 20 | 25 | 24 | 20 | 19 | 18 | 23 | 20 | 21 | 24 | 21 | 20 | 24 | 23 | 20 | 27 | 23 | 23 | 24 | 21 | 27 | 24 |
| $m03$ | 22 | 25 | 24 | 25 | 25 | 20 | 20 | 23 | 21 | 28 | 25 | 20 | 20 | 19 | 25 | 20 | 24 | 26 | 24 | 21 | 26 | 20 | 23 | 27 | 28 | 25 | 25 | 20 | 28 | 26 |
| $m04$ | 25 | 25 | 23 | 25 | 26 | 22 | 22 | 22 | 22 | 29 | 25 | 22 | 23 | 22 | 26 | 23 | 23 | 29 | 26 | 24 | 28 | 23 | 25 | 26 | 23 | 25 | 26 | 23 | 29 | 24 |
| $m05$ | 23 | 22 | 20 | 23 | 23 | 20 | 20 | 23 | 20 | 26 | 23 | 19 | 19 | 19 | 26 | 19 | 23 | 24 | 24 | 22 | 26 | 22 | 26 | 27 | 19 | 20 | 25 | 19 | 27 | 23 |
| $m06$ | 21 | 21 | 22 | 23 | 22 | 20 | 18 | 22 | 20 | 28 | 24 | 19 | 18 | 18 | 24 | 20 | 21 | 25 | 24 | 20 | 24 | 21 | 19 | 24 | 19 | 22 | 26 | 21 | 25 | 23 |
| $m07$ | 22 | 24 | 22 | 22 | 24 | 22 | 20 | 25 | 20 | 25 | 25 | 19 | 22 | 19 | 25 | 20 | 23 | 24 | 24 | 24 | 23 | 22 | 23 | 25 | 24 | 22 | 26 | 21 | 28 | 26 |
| $m08$ | 24 | 24 | 23 | 25 | 26 | 21 | 22 | 26 | 20 | 28 | 23 | 19 | 22 | 20 | 25 | 20 | 23 | 25 | 26 | 22 | 24 | 24 | 22 | 23 | 24 | 24 | 24 | 21 | 27 | 26 |
| $m09$ | 21 | 23 | 21 | 23 | 24 | 20 | 19 | 23 | 21 | 29 | 26 | 20 | 22 | 20 | 25 | 20 | 23 | 26 | 24 | 22 | 24 | 23 | 23 | 24 | 22 | 23 | 28 | 22 | 28 | 24 |
| $m10$ | 24 | 27 | 26 | 25 | 25 | 21 | 23 | 26 | 24 | 30 | 27 | 22 | 24 | 22 | 29 | 23 | 27 | 27 | 25 | 24 | 26 | 26 | 28 | 28 | 20 | 26 | 29 | 24 | 29 | 26 |
| $m11$ | 21 | 23 | 21 | 22 | 23 | 19 | 19 | 20 | 18 | 25 | 23 | 17 | 20 | 17 | 23 | 19 | 22 | 24 | 21 | 21 | 23 | 20 | 22 | 22 | 21 | 21 | 24 | 19 | 26 | 22 |
| $m12$ | 16 | 18 | 16 | 19 | 19 | 16 | 13 | 19 | 15 | 24 | 19 | 15 | 16 | 15 | 18 | 15 | 20 | 21 | 17 | 18 | 20 | 16 | 20 | 22 | 17 | 17 | 23 | 16 | 21 | 15 |
| $m13$ | 20 | 24 | 18 | 20 | 21 | 17 | 18 | 22 | 16 | 24 | 21 | 16 | 19 | 16 | 23 | 16 | 20 | 22 | 22 | 20 | 21 | 17 | 22 | 22 | 14 | 20 | 22 | 18 | 25 | 21 |
| $m14$ | 23 | 26 | 24 | 22 | 24 | 22 | 21 | 24 | 20 | 29 | 25 | 21 | 22 | 20 | 25 | 18 | 23 | 27 | 23 | 22 | 26 | 21 | 23 | 25 | 23 | 22 | 25 | 23 | 30 | 25 |
| $m15$ | 19 | 22 | 20 | 23 | 23 | 17 | 19 | 20 | 16 | 27 | 22 | 17 | 18 | 15 | 22 | 16 | 19 | 23 | 23 | 21 | 22 | 18 | 21 | 22 | 18 | 19 | 25 | 18 | 24 | 22 |
| $m16$ | 22 | 22 | 20 | 21 | 20 | 19 | 17 | 22 | 16 | 25 | 23 | 17 | 17 | 16 | 22 | 17 | 19 | 22 | 22 | 22 | 20 | 20 | 21 | 22 | 18 | 22 | 24 | 19 | 24 | 23 |
| $m17$ | 17 | 21 | 19 | 22 | 20 | 17 | 17 | 20 | 17 | 25 | 22 | 17 | 17 | 16 | 19 | 17 | 21 | 21 | 20 | 19 | 23 | 18 | 18 | 22 | 15 | 20 | 25 | 19 | 24 | 18 |
| $m18$ | 17 | 21 | 17 | 22 | 20 | 16 | 17 | 21 | 16 | 25 | 22 | 16 | 16 | 16 | 19 | 17 | 20 | 21 | 20 | 18 | 22 | 17 | 19 | 21 | 14 | 19 | 25 | 17 | 24 | 17 |
| $m19$ | 21 | 22 | 20 | 22 | 23 | 19 | 18 | 22 | 17 | 26 | 22 | 18 | 19 | 18 | 22 | 18 | 20 | 25 | 21 | 20 | 23 | 20 | 22 | 23 | 19 | 22 | 24 | 18 | 27 | 19 |
| $m20$ | 23 | 24 | 22 | 24 | 26 | 22 | 20 | 19 | 21 | 28 | 25 | 21 | 22 | 20 | 26 | 21 | 24 | 26 | 25 | 22 | 27 | 23 | 24 | 27 | 23 | 23 | 29 | 22 | 27 | 26 |
| $m21$ | 18 | 20 | 19 | 22 | 22 | 16 | 17 | 18 | 18 | 24 | 18 | 16 | 18 | 18 | 23 | 17 | 22 | 20 | 20 | 19 | 23 | 20 | 21 | 23 | 21 | 20 | 24 | 19 | 23 | 20 |
| $m22$ | 19 | 22 | 21 | 23 | 23 | 18 | 18 | 23 | 19 | 28 | 22 | 18 | 19 | 17 | 23 | 19 | 23 | 23 | 23 | 22 | 23 | 20 | 21 | 25 | 19 | 20 | 24 | 19 | 26 | 20 |
| $m23$ | 24 | 27 | 23 | 23 | 23 | 22 | 22 | 23 | 22 | 28 | 25 | 21 | 22 | 20 | 25 | 22 | 24 | 26 | 24 | 25 | 26 | 22 | 22 | 27 | 23 | 24 | 30 | 22 | 30 | 22 |
| $m24$ | 15 | 18 | 15 | 16 | 18 | 12 | 13 | 18 | 13 | 21 | 18 | 13 | 14 | 12 | 18 | 12 | 18 | 19 | 15 | 17 | 18 | 15 | 18 | 19 | 15 | 17 | 20 | 15 | 20 | 18 |
| $m25$ | 21 | 23 | 18 | 19 | 21 | 19 | 16 | 20 | 16 | 25 | 22 | 16 | 18 | 17 | 22 | 16 | 20 | 24 | 22 | 19 | 21 | 20 | 22 | 23 | 18 | 23 | 23 | 20 | 25 | 23 |
| $m26$ | 22 | 24 | 26 | 25 | 25 | 22 | 22 | 25 | 22 | 31 | 24 | 22 | 22 | 22 | 26 | 22 | 26 | 23 | 26 | 24 | 27 | 24 | 24 | 27 | 24 | 23 | 26 | 22 | 28 | 22 |
| $m27$ | 27 | 27 | 23 | 24 | 27 | 23 | 23 | 26 | 21 | 29 | 26 | 20 | 23 | 22 | 24 | 22 | 23 | 28 | 26 | 26 | 25 | 24 | 24 | 28 | 25 | 26 | 25 | 24 | 30 | 27 |
| $m28$ | 16 | 19 | 17 | 16 | 18 | 15 | 14 | 17 | 13 | 20 | 19 | 13 | 14 | 12 | 19 | 13 | 18 | 20 | 18 | 17 | 19 | 16 | 17 | 21 | 16 | 18 | 22 | 15 | 22 | 16 |
| $m29$ | 23 | 23 | 23 | 23 | 24 | 20 | 20 | 22 | 20 | 26 | 25 | 18 | 20 | 17 | 24 | 19 | 21 | 24 | 24 | 22 | 23 | 22 | 24 | 24 | 21 | 24 | 25 | 20 | 27 | 24 |
| $m30$ | 26 | 30 | 25 | 26 | 28 | 24 | 25 | 29 | 25 | 31 | 30 | 23 | 23 | 22 | 26 | 24 | 26 | 28 | 27 | 25 | 28 | 26 | 26 | 28 | 26 | 24 | 31 | 27 | 32 | 27 |
| $m31$ | 18 | 21 | 16 | 18 | 17 | 16 | 15 | 18 | 13 | 20 | 20 | 14 | 16 | 14 | 19 | 15 | 19 | 21 | 19 | 18 | 19 | 18 | 19 | 20 | 14 | 20 | 21 | 16 | 25 | 18 |
| $m32$ | 20 | 22 | 21 | 23 | 23 | 19 | 19 | 23 | 18 | 24 | 22 | 18 | 18 | 17 | 20 | 19 | 20 | 22 | 21 | 23 | 23 | 21 | 23 | 24 | 21 | 19 | 23 | 20 | 25 | 24 |
| $m33$ | 22 | 25 | 21 | 23 | 24 | 20 | 19 | 20 | 19 | 27 | 24 | 19 | 20 | 19 | 24 | 19 | 22 | 24 | 24 | 20 | 23 | 21 | 22 | 25 | 22 | 23 | 25 | 20 | 29 | 21 |
| $m34$ | 16 | 20 | 14 | 16 | 18 | 13 | 15 | 19 | 13 | 21 | 18 | 13 | 15 | 13 | 19 | 12 | 16 | 19 | 18 | 17 | 18 | 16 | 19 | 20 | 15 | 19 | 19 | 15 | 22 | 18 |
| $m35$ | 19 | 22 | 22 | 21 | 21 | 17 | 16 | 20 | 18 | 23 | 22 | 18 | 18 | 16 | 22 | 19 | 20 | 23 | 23 | 20 | 22 | 19 | 21 | 21 | 17 | 19 | 25 | 19 | 25 | 21 |
| $m36$ | 18 | 20 | 18 | 19 | 21 | 17 | 16 | 19 | 15 | 25 | 21 | 16 | 16 | 15 | 20 | 16 | 19 | 20 | 19 | 18 | 19 | 19 | 19 | 24 | 19 | 19 | 22 | 17 | 26 | 19 |
| $m37$ | 17 | 20 | 16 | 16 | 19 | 16 | 15 | 18 | 12 | 21 | 20 | 14 | 15 | 13 | 20 | 13 | 16 | 19 | 19 | 16 | 18 | 16 | 19 | 21 | 19 | 18 | 20 | 15 | 24 | 19 |
| $m38$ | 20 | 23 | 23 | 23 | 23 | 19 | 17 | 21 | 20 | 25 | 25 | 20 | 19 | 19 | 21 | 18 | 20 | 26 | 24 | 22 | 22 | 20 | 21 | 21 | 20 | 20 | 27 | 21 | 25 | 22 |
| $m39$ | 19 | 22 | 18 | 19 | 21 | 16 | 15 | 19 | 13 | 22 | 20 | 15 | 15 | 14 | 19 | 16 | 17 | 23 | 22 | 19 | 20 | 19 | 19 | 23 | 19 | 20 | 22 | 16 | 26 | 20 |
| $m40$ | 22 | 23 | 19 | 22 | 21 | 20 | 18 | 23 | 17 | 23 | 22 | 18 | 20 | 18 | 20 | 18 | 21 | 24 | 25 | 22 | 21 | 19 | 24 | 24 | 18 | 21 | 23 | 20 | 30 | 24 |
| $m41$ | 21 | 23 | 20 | 22 | 21 | 18 | 15 | 19 | 18 | 26 | 22 | 18 | 19 | 18 | 22 | 18 | 22 | 24 | 22 | 19 | 24 | 20 | 20 | 21 | 19 | 20 | 27 | 17 | 26 | 22 |
| $m42$ | 21 | 24 | 22 | 22 | 24 | 22 | 19 | 24 | 19 | 25 | 24 | 20 | 19 | 20 | 24 | 21 | 24 | 27 | 26 | 24 | 22 | 22 | 24 | 24 | 21 | 24 | 28 | 22 | 27 | 22 |
| $m43$ | 25 | 25 | 23 | 23 | 25 | 23 | 19 | 26 | 19 | 29 | 26 | 20 | 20 | 20 | 25 | 21 | 21 | 27 | 25 | 23 | 25 | 23 | 23 | 23 | 28 | 25 | 27 | 23 | 28 | 26 |
| $m44$ | 19 | 20 | 16 | 19 | 19 | 16 | 18 | 19 | 16 | 22 | 20 | 15 | 17 | 15 | 22 | 14 | 20 | 20 | 19 | 19 | 20 | 19 | 20 | 20 | 20 | 22 | 21 | 18 | 23 | 20 |
| $m45$ | 23 | 24 | 23 | 26 | 26 | 23 | 22 | 24 | 24 | 27 | 27 | 23 | 23 | 22 | 27 | 23 | 26 | 27 | 24 | 25 | 27 | 23 | 25 | 27 | 24 | 23 | 29 | 24 | 26 | 23 |

**Supplementary table** VIII: Human alpha monomers (from human alphoid HOR) and the corresponding closest chimpanzee alpha monomers (from chimpanzee HOR) with lowest mutual divergence.

| Human monomer | Chimp monomer | Divergence(%) |
|---|---|---|
| $m01$ | $\bar{e}07$ | $21,1$ |
| $m02$ | $\bar{e}06$ | $17,4$ |
| $m03$ | $\bar{e}14$ | $19,2$ |
| $m04$ | $\bar{e}14$ | $21,5$ |
| $m05$ | $\bar{e}14, \bar{e}28$ | $18,6$ |
| $m06$ | $\bar{e}07, \bar{e}14$ | $18,3$ |
| $m07$ | $\bar{e}14$ | $18,6$ |
| $m08$ | $\bar{e}12$ | $19,2$ |
| $m09$ | $\bar{e}07$ | $18,7$ |
| $m10$ | $\bar{e}25$ | $20,3$ |
| $m11$ | $\bar{e}14$ | $16,9$ |
| $m12$ | $\bar{e}07$ | $13,5$ |
| $m13$ | $\bar{e}25$ | $13,6$ |
| $m14$ | $\bar{e}16$ | $18,0$ |
| $m15$ | $\bar{e}14$ | $15,2$ |
| $m16$ | $\bar{e}09$ | $15,5$ |
| $m17$ | $\bar{e}25$ | $15,1$ |
| $m18$ | $\bar{e}25$ | $13,6$ |
| $m19$ | $\bar{e}09$ | $17,0$ |
| $m20$ | $\bar{e}08$ | $19,3$ |
| $m21$ | $\bar{e}06$ | $16,3$ |
| $m22$ | $\bar{e}14$ | $17,0$ |
| $m23$ | $\bar{e}14$ | $20,3$ |
| $m24$ | $\bar{e}06, \bar{e}14, \bar{e}16$ | $12,3$ |
| $m25$ | $\bar{e}07, \bar{e}09$ | $15,8$ |
| $m26$ | $\bar{e}01, \bar{e}07, \bar{e}09, \bar{e}12, \bar{e}14$ | $21,5$ |
| $m27$ | $\bar{e}12$ | $20,4$ |
| $m28$ | $\bar{e}14$ | $12,3$ |
| $m29$ | $\bar{e}14$ | $17,4$ |
| $m30$ | $\bar{e}14$ | $22,1$ |
| $m31$ | $\bar{e}09$ | $13,5$ |
| $m32$ | $\bar{e}14$ | $17,0$ |
| $m33$ | $\bar{e}14$ | $18,5$ |
| $m34$ | $\bar{e}16$ | $12,3$ |
| $m35$ | $\bar{e}07$ | $15,7$ |
| $m36$ | $\bar{e}09, \bar{e}14$ | $15,2$ |
| $m37$ | $\bar{e}09$ | $12,3$ |
| $m38$ | $\bar{e}07$ | $16,9$ |
| $m39$ | $\bar{e}09$ | $13,5$ |
| $m40$ | $\bar{e}09$ | $17,4$ |
| $m41$ | $\bar{e}07$ | $14,6$ |
| $m42$ | $\bar{e}07$ | $19,2$ |
| $m43$ | $\bar{e}07, \bar{e}09$ | $18,7$ |
| $m44$ | $\bar{e}16$ | $14,0$ |
| $m45$ | $\bar{e}14$ | $21,5$ |

**Supplementary table** IX: Chimpanzee 550 bp monomers *mc*01, *mc*02 and *mc*03 in consensus 3mer (1,651 bp) determined by GRM analysis of genomic sequence (contigs NW_001252915.1, NW_001252919.1, NW_001252921.1, NW_001252925.1 and NW_001252926.1 NCBI Build 2.1). In parentheses: lengths of monomers (in bp).

*mc*01(550)

```
AGGTACTGTACCTTTTTCTGGATTTGTCAAATAGATTTCTTAAATTGTTCATTCCAACTAACGTTCTATCAGG
GCTCCAATTTATCTACATCCTCTCAAACACTTGTTATTTCCTGCTTTTGAAAATTTATTGCCCTTCCAGTGTG
TGTGTGTGAAATATGATATCCCATTCTGGATTTGAAATGCATTTTCTGCACCCATTAACTCATCATGCACATG
TACCCTAGAACTTAAAGTATAATAAAAAAAAAGAAATGCATTTTCTGAATCACTGAATATGTGTATCTGTCCC
ATGTGCATCTTGGGCATTTGCCCATTTTATTTGGAGAAATATCTATTTAGATGTTTGGCCTTTTAATTTTGTT
TAAGTTGTAAGTTAGTCATATATCGGATACTAGAAGTTGAAAATTTAAAATTTGTTGCTTAAACTTATGCATA
CAGAAATCATCGAAGCTCCCGAGAAACTAGGGATTATGCTCCACCATCTAGAGGCCATGCATACCGTGATTGT
GGTCATTCTCATCGGCATGAAACTTATTCCAGAGGATAT
```

*mc*02(551)

```
AGGTACTGTACCATTTTCTGGATTTGTCAAATAGATTTCTCAAATTGTTCGTTCCAACTAACATTGTATCAGG
GCTCCAATTTACCGACATCCTCTCAAACACTTGTTATTTCCTGCTTTTGAAAATTTATTGCCATTCATCGGTG
TGTGTGAAATATGATATCTCATTTTGGATTTGAAATGCATTTTCTGCACCCATTAACTCATCATGCACATGTA
CCCTAGAACTTAAAGTATAATAAAAAAAAAAAAGAAATGCATTTTCTCAATCACTGAATATGAGTATCTGTCC
CATGTGCTTTTTGGGCATTTGCCCATTTTATTTGGAGAAATATCTGTTTAGATGTTTGGCCTTTTAATTTTGT
TTAAGTTGTAAGTTAGTCATATATCAGATACTAGAAGTAGAAAATTTAAAATTTGTTGCTTAAACTTATGCAT
ACAGAAATCATCGAAGTTCCCGAGAAACTAGGGATTATCCTCCACCATCTAGAGGCCATGCTTACCGTGATTA
TGGTCATTCTCGTCGGCATGAAAGTTATTCTAGAGGATAT
```

*mc*03(550)

```
AGGTACTGTACCTCTTCTGGATTTGTCAAATAGATTTCTTAAATTGTTCATTCCAACTAACATTGTATCAGGG
CTCCAATTTATCTACATCCTCTCAAACACTTTTTATTTCCTGCTTTTGAAAATTTATTGCCATTCATCTGTGT
GTGTGAAATATGATATCTCATTTTGGATTTGAAATGCATTTTCTGCACCCATTAACTCATCATGCACATGTAT
CCTAGAACTTAAAGTATAATAAAACAAAAAGAAATGCATTTTCTGAATCACTGAATATGAGTATCTGTCCCTT
GTGCTTTTTGGCCATTTGCCTATTTTATTTGGAGAAATATCTATTTAGATGTTTGGCCTTTTAATTTAAAGTT
GTAAGTTAGTCATGTATTCGATACTAGAAGATGAAAAGTTAAAATTTGTTGCTTAAACTTATGCACAGAGAAA
TCATCCAAGTTCCCGAGAAACTAGGGATTATGCTCCACCATCTAGAGGCTAGGCATACTGAGACTATGGTCAT
TCTAGGCAGGATGAACATTCCTCTAGAGGATATAGATAC
```

**Supplementary table** X: Human consensus ∼2.4 kb DAZ monomers in consensus 5mer HOR unit determined by GRM analysis of genomic sequence.

$m01(2446)$

TATTTTTAATGATTCTTTATATTGATGTGTTAACGTTTTGTTACTTTCTTTTTAACCCAATTATAATCTCCCA
TGGGAGAAACAGTGCCTTTTTCTCTCTCAGGTTTTTGTATGCTTAAGCAATGGCTTCTCCAAATTATGACAAG
TGTTCAGTTACTTGTTGATAGATTATTTAATCTAAGAAAGGTAGTCCTAATGTGGCTTTATCTAAGAAAGGTA
GTATTAATTTGGCTTTAGAATAGCATGTATCTGATGAGAATCTGCATCTGGATGTACCAACCATAAAAAATTT
CATAAAAGAAACAGAAATGTTTTGCTGTTAATTACTCTTAAATAAGAATAGGATTAAAAAGAGTATTACCTCT
ATAACACCTGAGCTGCTTTCCCCCATATAACTAAAATATTTAAAAGCAGTTCTCCTCATGTGTCTGCCTGCTT
TATTCTTCTCTAAGTTTAGCAGTTAATCCAGGTATTCTTTATTTGAAATGATTTCCAGATGCCTCTGCATATT
AAATTGCTGACTTCCAGATATATTCTGGTTCTGGAATGGGTAGATTTCTGATATGTTTTAGGTATCTGTAAAT
CCCGCAAGTTTCTGGCATGTAGTGTCTCTGATCCTTGTTAGTTTGCTATTTAAAGTAGATTTGACATATTCTG
TCACTTACTGGTGGTAAATAACGTTTATTTTCTTCTTAGTTCATTTTATTTATATCTTAGTTTAAAAGACATT
TTCTTTGATGGAAAATAAAGTAACAGAATAGTAGTGAAGTAGTTATATTCAGTGTTTCTCATTTGTTGACATT
TTCCCTGTACTTGAAACATGTACGGTATACCTCATCTTCTTTTTCCTTCTGTGAACAATGGCTGGAATAAAAG
CCCTACTTCTATCATTTACTGTGAGCCATTACTGAATCTGGGTGTATTGATGCATGCTGCTTACCTATATGTG
TTGAAACAATAAGTATTTATTGAAACATATGAGACATTATACTGTCTCTTTTCCAGTATTGGATTCTATACTG
CACTTAGTTTTTCAACATGAAGTACAGAAAACGCCGTAAATTCTGCAGAACTACGTATTACCTTATAATATTG
TCAAATACACATCAGTCTGGAAGCATTTTTACAGGGAAATAGCAAATGTATTAATTTAACTTACATTGAACTC
TGTCTTAATGCAGCCTTATCACCAGTGCAAGAAATAACTTCTGGGTGGGCATAAGTACACAATATAAGTAAGG
TTAACTTTGCCTGGTGTCATAGCCAGTTCTTTTGACATTTGTCTGTTCCCCCTCCACGCCCAACCATAGCACT
TGACCGAGAATAATACGTTCTTCATAAATCAGTCAGTCACTTACAATTCTACATTGTTGCAGATAGAAAAATA
ATTAGTATTTCGAAATTTTTCATAGTTTTGTTATATTGGGACTAATTCTTCCTAATTAAAAATAATGTTTTAA
CGTATTAATTCATTCTTTCTGTATAATTTATTTTCAGGAATATCCTACTTATCCCGATTCAGCATTTCAGGTC
ACCACTGGATATCAGTTGCCTGTATATAATTATCAGGTAATGTAAGAGGGGAGTAAAATGATTTGCTTTCAGGT
ATTATTGGGGCCTTTAACTTTTTTAGACAAATTTCCTGAACAGTTGGTCATTTTAAACTAGTGAAGTGTACCT
AAAATTTAAGGAAACACTTAGAATTAGTGTAGAATGAAGACATCTGTCTTATTTAGAAGTAATGAAGTAGTAT
TTTGAGAGGAATATACCTGGCAATAACATTTCTGTAGAAGAGATTTCTGAGATGTGGTGTTCTCTCCTTTACT
TCTGGATGTAGTTTTCATCTTTACTGTGAAATAGCTGAATGAAACATCCAAACTGACTTTCATGAATTTTCTT
AGGGAGATAGAGTGAAATAAATTTCTGCTGCACTTTTCAGAGCACAGAATCCCAATTACATTTTCATTTTAGC
TGGCTGTTTGAAGATAGTAATTCTCTGGATCTCTTTTCATAGATACAAGTATATCTATGACCCATAATTATAT
CTATGGTAATAAACTGAAAGAGGTAGTATCTTGGAGGTTTCCACATTGCCAACTCCTGAAAATTTGGAGAAAG
ATGAAGTTTCAAATATAAAAGTAAGAAGAATGTCATGGACTAGAAACATGATGTACTTAAGTTTTCCTTTCTG
TTACTTTTATTATAATAAAAAAGGAGACAGCAGGATAAGGACTTCAATATTGTGTTTCTCATGAGTTTTTGAA
AATGTGTAGGAATACTTTAATAGTTTTGGTGTCCTTTTTTTTTTTTTTTTTTTTTTTTTTTAAGATGCCACCAT
AGGGGCCTGTTGGGGAGCAAAGGGATTCCGTTCTTGACGTTAAGTGAATTAGCCAAACATAGACTTCCTGTTC
ATTCTTGATTTTTTTCCATGTCCTATATGCCTATAAA

$m02(2404)$

TATTTTTAAGTGATTCTTTATATTAATTTTTTTGTCGTTGTTACCTTCTTGTTAACCCGATTATAAACTCCCA
TGGCAGCAACAGTGCCTTTTTTGCCCTCAGGTTTTTATGTGCCTAAGCAATGGCAGGTCCACATAATGATAGA
CTATATAATCAAAGAAAAGGAGTATTCACGTGACTTTAGAATTAGCACGTATCTGCAAAGAATATGCCTCTGG
CTTTACCAGCAATAGAAAATTTATAGAAGAGAAACAGAAATGCTTTGCTGTTAATGACGCCTAAATAAGAACA
GGAGTAAACGAGAGTATTACCTCCAAATCACCGGAGCTGCTTTCCCCCTTATAAGCAGTTCCTAAAGTGAATG
AAAGCAGCTCTCCTTATGTGTCTGCCTACTTTATTCTTCGGTAAGTTTAGCAGTTCATCTAGCTATCCTTTAT
TTGAAATGATTTCCAGATGCCTCCTCATATAAATTGCTGACTTCTGGATATTTCCTGGTTCTGGAATGGGTAG
ATTTCTGATGTGGTTTAGTATATATATGTAAACCCCGTGAGCTTCTGGCATCTAATTTCTCTGATCCTGGTTA
CATTGATATTTAAAGTAGGGTTTGACATACTCTGTCACCTACTGTTGATAAATAACGTTTATATTCTTCTTAG
TTCATTTTATTGACGTGTTAGCTTTAAAGACATTTTCTTTGACGGAAAATGAAGTAACAAAATAATAGTGAAA
TAGTTATGCAGTGTCTCTAATTTGTTGATATTTTCCATGTACTTGAAACTTGTATGGTATACCTCTTCTTTTT
CCTTCTCTGAACAATGGCTAGAAAAAAAGTCCTACTTTTTTCTGTCATTTACTGTGAGGCATCACTGATTCTG
GGTGTATTCATGTATGCTGCTACCTGTATGTTTTCAAACAATAAGAATTTATTGAAACATGTAAGACATTATA
CTTTCTCTTCTCCAGTATTGGATCATAGACTGCACTTAGTTTTTCGTAATGAAGTACAGACAAAGCCATAACA
TCTGTCGAACTACATATTACCCTATAATATTGTCTGATACAAAACAGTCTAGAAATATTCTTACAGAGAAATT
GCAAATGTATTAATTTAACTTACCTTGCAATCTCTCTTAATGGAGCCTTACCACCAGTGTAAGAAATAACGTC
TGGGTGTGAATAAGTACACAGTATAAGGTAAACTTTGGTGAAGTAGTCAATTCTTTTGTCATTTGTTCCCCCT
TCACACCCATAGTGTAGCACTTGACCTAGAATCTTTCTTTCTTCATAAAGTCAGTCATTCATTTGGAATTCTG
CATTGTTGTACGTAGAAAAAGGATATTTTACCTTTTGTAATATTTTTGTTATATTGGGAATTATATTTCTTTG
TAATTTTAAAAAGTGGTTTACCATATTCATTTTTTTCTGCAACCTTTCTTTTCAGCCATTTCCTGCTTATCCA
AGATCACCATTTCAGGTCACTGCTGGATATCAGTTGCCTGTATATAATTATCAGGTAATGTAAGAAGGAGTAA
AATGATTTACTTTCAGGTATTACTGAGGCATTCAACTTGTTTATACAAATTTCCTGAATAGCTGGTCATTTTA

```
AATTAGTGAAGTGTACCTAAAATTTAAGGAAACACGTAGAAGTAGTGTAGAATGAAGACCTCTGTCTTATTTA
GAAGTAATGAAGTAGTATTTTGAGAGGAATATACTTGGCAATAACTTTTCTGTAGAAGAGATTTCTGAGATGT
GGTGTTCTCTTCTTTATTTCTGGATGCAGTTTTCATCTTTACTGTGAAATAGCTGAATGAAACATCCAAACTG
ACTTTCATGAATTTTCTTAGGGAGATAGAGTGAAATAAATTTATGCTGCACTTTTCAGAGCACAGAATCCCAA
TTACATTTTCATTTTAGCTGGCTGTTTGAAGATAGTAATGCTCTGGATCTCTTTTCATAGATACAAGTATATC
TATGACCCATAATTACATCTATGGTAAGAAACTGAAAGAGGTAGTATCTTTGAGGTTTCCACCTTGCCAACTC
CCGAAAATTTGGAGAAAGGTGAAGTTTCCAATATAAAAGTAACAAGAATGTCATGGACTAGAAACATAAAGTA
CTTAAGTTTTCCTTTCTGTTACTTTTATTATAATGAAAAAGGAGACAGCCGGATAAGTACTTCAATGTTGTAT
TTCTCATGTGTTTTTGAAAATGTGTAGGAATACATATAATAGTTTCGGTGTCCTTTTTTTTTCTTTCTTTTTC
TTTCTTTTTTTTTTTTAAGATGCCACCATAAGGTCCTGTTGGGGAGCAAAGGATTATGTTGTCCTTGACGTTA
AGTGAATTAGCCAAACATAGATTTCCTGTTCATTCTTGATTTTTTTCCATGTCATATATGCCTATAAA
```

$m03(2376)$

```
TATTTTTAAGTGATTCTTTATATTAATTTTTTTGTTGTTGTTACTTTCTTGTTAACCCGATTATAAACTCCCA
TGGGAGCAAGAGTGCCTTTTTTGCCCTCAGGTTTTTATGTGGTTAAGCAATGGCAGGTCCATATAATGACAGA
CTATATAATCAAAGAAAGGTAGTGTTCATGTGACTTTACAATTAGCATGTATCTGCATAGAATCTGCCTCTGG
CTTTACCAGCAATAGAATATTTATAGAAGAGAAACAGAAATGCTTTGCTGTTAATGACGCTTAAATGAGAATA
GGAGTAAACGAGAGTATTACCGCCAAATCACCGGAGCTGCTTTCCCCCTTATAACCAGTTCCTAAAGTGAATG
AAAGCAGCTCCCCTTATGTGTCTGCCTACTTTATTCTTTGGTAAGTTTAGCAGTTCATCTAGCTATTCTTTAT
TTGAAATGATTTCCGGATGCCTCCTCATATAAATTGCTGACTTCTGGAAATATTCTTCTTCTGGAATGGGTAG
ATTTCTGATGTGGTTTAGTATATATATAAACCCCGTGAGCTTCTGGCGTCTAATTTCTCTGATTCTGGTTACA
CTGATATTTAAAGTAGGGTTTGACATACTCCATCACTTAATGTTGATAACTAACCTTTATATTCTTCTTAGTT
CGTTTTATTTATGTGTTAGCTTAAAAGACATTTTCTTTGATGGAAAATGAAGTAACAAAATAATAGTGAAATA
GTTCTGCGGTTGTCTCTAATTTCGTGATATTTTCCATGTACTTGAAACATGTATGGTATACCTCTTCTTTTTC
CTTCTCTGAACAATGGCTAGAAAAAAAGCCTTACTTGTTTCTGTCATTTACTGTGAGCGATTACTGAATCTGG
GTGTATTCATGTATGCTGCTACCTGTATGTTTTCAGATAATAAAAATTTTTTGAAACATATAAGACATTATAC
TTTCTCTTGTCCAGTATTGGATTATAGACTGCACTTAGTTTTTCGTAATGAAGTACAGACAAAGCCATAACAT
CTGTCAAACTATATATTGTCCTATAATATTGTCTGATACAAAACAGTCTAGAAATATTCTGACAGGGAAATAG
CAAATGTATTAATTTAACTTACCTTGCAATCTCTCTTAATGGAGCCTTACCACCAGTGTAAGAAATAACTTCT
GGGTGTGAATAAGTACACAGTATAAGGTAAACTTTGGTGAAATAGTCAATTCTTTTGTCATTAGTTCCCCCTT
CACTCCCAAAGTGTAGCACTTGTCATAGAATCTTTCTTTCTTCATAAAGTCAGTCATTCATTTAGAATTCTGC
ATTATTGTATGTAGAAAAACAATATTTTACCTATTTTTGTTATATTCAGAATTATATTTCTTTCTAATTTTAA
AAAAATGGTTTACCGTATTCATTTTTTTCTGGAACCTTTCTTTTCAGGCATTTCCTGCTTATCCAAATTCACC
ATTTCAAGTCGCCACTGGATATCAGTTCCCTGTATACAATTATCAGGTAATGTCAGAGGGAGTAAAATGATTT
GCTTTTAGGTATTATTGAGGCCTTTAACTTGTTCATACAAATTTCCTGAATAGTTGCTCATTTTAAACTAGTG
AATTGTACCTAAAATTTAAGGAAACACTTAGTGTAGAATGAAGACCTCTGTGTTATTTAGAATAATGAGGTAG
TATTTTGACAGGAATATACTTGGCAATAACTTTTCTGTAGAACAGATTTCTGAGATTTGGTGTTCTCTTCTTC
ATTTCTGGATGTAGTTTTCATCTTTACTGTCAAATAGCTAAATGAAACGTCCAAAGTGTCTTTCATGAATTTT
CTTAGGGAGATAGACTGAAATAAAATTATGCTGCACTTTTCAGAGCACAGAATCCCAATTACATTTTCATTTT
AGCTGGCTGTTTGACGATAGTAATGCTCTGGATCTCTTTTCATAGATACAAGTGTATCTGTGACCCATAATTA
TATCTACGGTAATAAACTGAAAGAGCTAGTATCTTTGAGGTTTCCACATTGCGAAATCCCGAAAATGTGGAGA
GAGCTGAAGTTTCCAATGTAAAAGTAACAAGAATGTCATGGACTAGAAACATAAAGTATTTGAGTTTTCCTTT
CTGTTACTTTTATTACAATAAAAAAGGAGACAGCAGGATAAGTACTTTAATATTGTGTTTCTCATGTGTTTTT
GAAAATGTGTAGTAATACTTCAATAGTTTTGGTTTCCTTTTATTTATTGATTGATTTTTTAAGATTCCACCTT
AGGGGCCTGTTGGGTAGCAAAGGGATTATGTTGTCCTTGACGTTAAGGGAATTAGCCAAACATAGACTTCCTG
TTCATTCTTGATTTTTTTCCATGTCATATATGCCTACAAA
```

$m04(2375)$

```
TATTTTTAAGTGACTTTTTATGTTAATGTTTTTTTTGTTGTTGTTTCCTTCTTGTTAACCCGATTATAAACTC
CCATGGCAGCAACAGTGCCTTTTTTGTCCTCAGGTTTTTATGTGCTTAAGCAATGGCAGGTCTACATAATGAT
AGACTATATAATCAAAGAAAGGGAGTATTCACGTGACTTTAGAATTAGCATGTGTCTGCACAGAATATGCCTC
TGGCTTTACCAGCAGTAGAAAATTTATAGAAGAGAAACAGAAATGCTTTGCTGTTAATGACGCCTAAATAAGA
ATAGGAGTAAAGGAGAGTATTACCTCCAACTCACCGGAGCTGCTTTCCCCCTTATAAGCAGTTCCTAAAGTGA
ATGAAAGCAGCTCTCCTTATGTGTCTGCCTACTTTATTCTTCGGTAAGTTTAGCAGTTTATCTAGCTATCCTT
TATTTGAAATGATTGCCACATGCCTCCTCATATAAATGGCTGACTTCTGGATATATTCTGGTTCTGGAATGGG
CAGATTTCTGACGTGGTTTAGTATATATATATAAACCCGGTGAGTTTCTGGCATGTAATTTCTCTGATCGTGG
TTACATTGATATTTAAAGTAGGGTTTGACATAGTGTGTCACTTACTGTTGATAAATATCGTTTATTTTCTTCT
TAGTTCATTTCATTGATGTGTTAGCTTAAAAGACATTTTCTTTGACAGAAAATGAAGTAATGAAATAATAGTG
AAATCGTTCTGCTGTGTCTCTAATTTGTTGATATTTTCCATGTACTTGAAACATGTATGGTATACCTCTTCTT
TTTCCTTCTCTGAACCATGGCTAGAAAAAAAGCCCTACTTGTTTCTCTCGTTTACTGTGAGGCATTAGTGATT
CTGGGTGTATTCATGTATGCTGCTAACTGTATGTTTTCAAACAATAAGAATTTGTTGAAACATGTCAGACATT
ATACTTTTTATTCTCCAGTATTGGAATATAGACTGCAATTAGTTTTTTGGAATGAAATACAGACAAAGCCATA
```

ACATCTATAGAACTACATATTACCCTACAATATTGTCTGATACAAAACAGTCTGGAAATATTCTTACAGCGAA
ATTGCAAATGTATTGATTTACCTTACATTGCAATCTGTCTTAGTGGAACCTTATCACCAGTGTAAGACATAAT
TTCTGGGTGTGAATAAGTACACAGTATAAGGTAAATTTTGGTGAAGTAGTCAGTTCTTTGTCATTTGTTCCCC
CTTCACACCCAAAGTGTAGCACTTGACATAGAATCTTTCTTTCCTCATAAAGTCATTCATTTGGAATTCTGCA
TTGTTGTATGTAGAAAAAGGATATTTTCCGTTTTGTAATATTTTTCTTATATTGGGAATTATATTTCTTTCTA
ATTTTAAAATGTGGTTTACCATATTCATTTTTTCTGCAACCTTTTCAGGCATTTCCTGCTTATCCAAATTCAC
CAGTTCAGGTCACCACTGGATATCAGTTGCCTGTATACAATTATCAGGTAATGTAAGAGGTAGTAAAATGGTT
TGCTTTCAGGTATTATTGAGGCCTTTAACTTGTTTATAGAAATTTCCTGAATAGTTGGTCATTTTTAACTAGT
GAAGTGTCCCTAAAATTTAAGGAAAGACTTAGTGTAGAATGAAGACCTCTGTCTTATTTAGAAGTAATGAAGT
AATATTTTTACAGGAATATCCTTGGCAATAACATTTGTGTAGAAGAGATTTCTGAGATTTGGTGTCCCCTTCT
TCATTTGTGGATATAGTTTTCATCTTTGCTGTCAAATAGCTGAATGAAACATCCAAACTGACTTTCATGAATT
TTTTTAGGGAGATAGAGTGAAATAAAATTATGATCCACTTTTCAGAGCACAGAATTCCAATTATATTTTCATT
TTAGCTGGCTGTTTGACGGTAGTCATTCTCAGGATCTCTTCTCATAGATACAAGTATATCTATGACCCATAAC
TATATCTATGGTAATAAACTGAAAGAGCTAGTATTTTTGAGGTTTCCACATTGCCAACTCCCAAAAATTTGGA
GAAAGGTGAAGATTCAAATTTAAAGTAACAAGAATGTCATGGACAAGAAACATAAAGTACTTAAGTTTTCCTT
TCTGTTACTTTTATTATAATAAAAAAGGAGACAGCGGAATAAGTACTTCAATACTGTGTTTCTCATGTGTGTT
TGAAAATATGTAGGAATAGTTTAATAGTTTTGGTTTCCTTTTTTTTTTTTTTTTTTTAAAGATGCCACCTTAG
GGGCCTGTTGGGGAGCAAAGGGATTATGTTGTCCTTGACGTTAAGGGAATTAGCCAAACATAGACTTCCTGTT
CATTCTTGATTTTTTTTCCATGTCATATATGCCTATAAA

$m05(2385)$
TATTTTTAAGTGATTTTTATATCAATGTTTTAGTTTATTTTTTTACTTTCTTGTTAACCCGATTATAAACTCC
CATGGGAGCAACAGTGCCTTTTTTGCCCTGAGGTTTTTATTTGCTTAAGCAATGGCAGGTCCACTTAATGATA
GACCATATCATCAAAGAAAGGTAGTATTCATGTGGCTTTTGAATTAGCATGCATCTGCGTAGATTCTGCCTCT
GGCTTTACCAGCAACAGAAAATTTGTAGAACAGAGACAGAAATGCTTTGCTGTTAATTGCGCTTAAATAAGAA
TAGGAGTAAACGAGAGTATTACCTCCAAAGCACCAGAGCTGCTTTCCTCCTTATAACCAGTTCCTAAAGTGAA
TGAAAGCAGCTCTCCTTATGTGTCTGCCTACTTCATTCTTCGGTAAGTTTAACAGTTCATCTAGCTACCCTTT
ATTTGAAATGATTTCCAGATGCCTCCTCATATAAATTGCTGACTTCTGGATATATTCTGGTTCGGGAATGGGT
AGATTTCTGATGTGGTTTAGTAGGTATATAAATCCCGTGAGCTTCTTGCATCTAATTTCTCTGATCCTGCTTA
CACTGATATTTAAAGTAGGTTTTGACATACTCCATCACTTAATGTTGATAAAGGACGTTTATATTCTTCTTAG
TTCGTTTTATTTATGTGTTAGCTTTAAAGACATTTTCTTTGACGGAAAGTGAAGTAACAAAATAATAGTCGAA
TAGTTCTGCCGTGTCTCTAATTTGTTGATATTTTCCATGTACTTGAAACATGTATGGTACACCTCTTCTTTTT
CCTTCTCTGAACAATGGCTAGAAAAAAAAACCCTACTTCTTTCTGTCATTTACTGTGAGGCATTACTGAATCTG
GGTGTATTCATGTATGCTGCTACCTGTATGTTTTCAAACAATAAGAATTCATTGAAACATATAAGACATTATA
CTTTCTCTTCTCCAGTATTGGATTATAGACTGCACTTAGTTTTCCGGAATGAAGTACAGACAAAGCCATAACG
CGTGTACAACTACACATTGTCCTATAATATTGTCTGATAAAAAACAGTGTAGAAATATTCTGACAGGGAAATA
GCAAATGTATTAATTTAACTTACCTTGCAATCTCTCTTAATGGAGCCTTATCACCAGTGTAAGAAATAACGTC
TGGGTGTGAATACGTACACAGTATAAGGTAAACTTTGGTGAAGTCGTCAATTCTTTTGTCATTTCTTCCCCCT
TCACAGCCAAAGTGTAGCACTTGACATGGAATCTTTCTTTCTTCATAAATCAGTCATTCATTTGGAATTCTGC
ATTGTTGTATGTAGAAAAACGATATTTTCCCTTCTGTAATATTGTTGTTATATTGGGAATTATATTTCTTTGT
AATTTTAAAAAGTGGTTTACCATATTCATTTTTTTCTGCCAACCTTTCTTTTCAGGCATTTCCTGCTTATCCA
AGTTCACCATTTCAGGTCACCACTGGATATCAGTTGCCTGTATATAATTATCAGGTAATGTAAGAAGGAGTAA
AATTATTTGCTTTCAGGTATTATTGAGGCCTTTAACTTGTTTATACAAATTTCCGGAATAGTTGGTCATTTTA
AACTAGTGAAGTGTACCTAAAATTTAAGGAAACACTTAGAATTAGTGTAGAATGAAGACCTCTGTCTTATTGA
GAAGTAATGAAGTCGAATTTTGACAGGAATATACTTGGGAATAACTTTCCTGTAGAACAGATTTCTGAGATTT
GGTGTCCCATTCTTCATTTCTGGATGTAGTTTTCATCTTTACTGTCAAATAACTGAATGAAACATCCAAACTG
ACTTTCATGAATTTTCTTAGGGAGATAGAGTGAAATAAAATTATGACCCACTTTTCAGAGCACAGAATTCCAA
CTATATTTTCATTTTAGCTGGCTGTTTCACGATAGCAATTCTCTGGGTCTCTTTTCACAGATACAAGTACATC
TATGCCCAATAATTATATCTATGGTAATAAACTGAAAGAGCTAGTATCTTTGAGGTTTCCACATTGCCAACTC
CCGAAAATGTGGAGAAGGGTGAAGTTTCTAATATAAAAGTAACAAGAATGTCATGGAGTAGAAACATAAAGTA
CTCAAGTTTTCCTTTCTGTTACTTGTATTATAATAAAAAAGGAGACAGCAGGATAAGTGCTTCAATATTGTGT
TTCTCATGTGTTTTTGAAAATGTGTAGGAATATTTTAATAGTTTTGGTTTCCTTTTTTTTTTTTTTTTTAAGA
TGCCACCATAGGGGCCTGTTGGGGAGCAAAGGGATTATGTTTTCCTTGATGTTAAGTGAATTAGCCAAACATA
GACTTCCTGTTCATTCTTGGTTTTTTTCCACGTCGTATATGCCTATTAC

**Supplementary table** XI: Tandem of 11 monomer copies (consensus length 5607) in contig NT_113819.1. First column: length of repeat copy. Second column: start position within contig. Third column: divergence with respect to consensus. The second and third copy are truncated by $\sim$ 40% with respect to consensus. The first six copies have divergence between 2 and 19%, while the last five copies in tandem are highly identical (divegence less than 1%).

| Length(bp) | Start | Divergence(%) |
|---|---|---|
| 5566 | 496682 | 3,8 |
| 3361 | 502248 | 13,4 |
| 3361 | 505609 | 12,4 |
| 5624 | 508970 | 5,6 |
| 5651 | 514594 | 18,8 |
| 5607 | 520245 | 2,2 |
| 5607 | 525852 | 0,8 |
| 5602 | 531459 | 0,2 |
| 5606 | 537061 | 0,1 |
| 5607 | 542667 | 0,1 |
| 5607 | 548274 | 0,2 |

**Supplementary table** XII: Human consensus sequence for 5607 bp HOR unit (5bp GGAAT primary repeat unit).

AAGGTCTCAAATGGAATTTATTCAATACAATGGAATCGAATGGAATGCAATAGAATGGAATGGAATCGAATGT
AATGGAATCAAATAGAATGGACCAGTATGGAATGGACTGCCATAGAACGGACTGCAGTGTAATGGATTGAATT
CTAATTCATTCAAATGGAATGGAATTGAATGGAATGGAATCCAATGGAATGGATAGGATTGTACTGGAATGGA
ATAGCATGGAATGCAACGGAGTGGAATGGAGTTGAATGAAGTGGAATGGAATCGATCGGAATGGAATCAAATG
GAATGGACGGGAATGGAATGGACTGGAAGAGAACAGACTCGAATTTAATGGATTGCAATGTAATTGATTCAAA
GGGAATGGAATCGAATGGAATGTAATAAAATTGAAGGGATTTGAGTTCAATGCAATGGAATAGAATGGAATGC
AAAGGATAGGAAAGGTACGGAGTGAAATCGAGTGTAATGGAATCGAATGGAATGAAATGGAATGGAATGGACT
CAAAAGAAATGGACGAGGGACAAAACGGAATCGAACTGATTGGAATCGAACGGAACGGAATGGAATGGAATGG
TCTCCATTGGATCGGAGTAGAACGGACTGGAATGGAATGGAATGAAATGGAATGGAAAGGAATAGAATGGAAT
GGAATGGAATGGAATGGAATGGAAGGTAATGGAAAGATATCGAACGGATTGGAAAGGAATGGAATGGACCCTA
ATGGAATGGAATGGAATTCAACAGAAACGAATGGAATGGACTGGAGTGAAATGGAGTCGAATGTAATTGACTG
GAGTGGAATGGACTCGAAAGGAATGGACTCGAATAGAATGGACTGGAATGGATTGTACTCGAATGGAGTGGAA
AGGAATAAAATGGATTGCACCAGATTGGAATGGAACAGAATGTAATGGAATGGAATGGAATGCAATGGAATGG
CTCCAATGGAATGGAGTCGAATGCAATGGAACAGAAAGGAAAGGAATTGAATGGAATTGAAAGTAATAGAACA
AAATGGAGTGCAAAGGAAAGATATTGAATGGAATGAATCGAAAAGAAATCGAATGGAATGGACAAGAATGGAA
TGGAATAGAATGGAATAGACTGGCGTGCAATGAAAACGAATGGAACGGAAACGAATGGAATGCAATGGAAAGG
AATGGAGTAGAATAAATACTATGGAATGGAATGGAGGCGAAAGGAAAAGAATGGATTGGAATGTCACCGAATG
GAAAGATATGGAATGGAAAGGAATGGATACGAATGGAATGGAATAGAAAGGAACGGAAAGGTAAAGAATGGAA
TGGAATCGGATAGAATGGAATGCAATGTAATGGAGTCGAATGGAAAATAATCGTGTAGAATGATATCGAATGG
AATGGAATGGAATGGAATGGACTCGAATGGAATGTACTCAAATGGATTAGAATAGAATGGAATGGAACTAAAC
GTAATGAACTCGAATGGAATGGACACAAATAGAATGGAAGAGAAGGGAATGGTATTGAATGGAATTTATTCGA
AAAGAGTGGAATTCAATGGAATGCAGCAGTGTGGCATGGAATCAAATGGAATGGAATCGAATGGAATGGACCC
GAGTGGAATGGACTCACATAGAACAGCCTCGAATGTAATGGATGACAATGTATTAGATTCGAAAGGACTGAAA
TCGAATGGAATGTAATCAAGTAGAACGGAATTGAATGCATGGAATGGCATAGAAAGTAACGCAATGGAATGGA
ATAGACTGGAATGGAATGGAATCGGATGGAATGTAATGAAATGTAATGGAAGGAATGCCATGGAATGGAATGG
AATGGAATGCAATGGGACGGTGTATAATGGAGTGCAATGGATTTCAGTGGAATGTAGTCAAAAGGAAAGAAAT
AGAATGGAATTCAATATAATGGAATGGCATCCAATGGCAAGGAATGGAGCGGACTCCAATGGAAACGACATGA
AAGGAATATAATAAAATGGAATGGCATTGAACGAAATGGAATGCAATGGAGTTAAAAGGTAAAATATCGAATG
GAAAAGAATTGAATGGACTCGAAAGGAATATAATGGAATGGAATGGACTCGAATGGAATGTACTAGAGTTGAA
TGGAATCGAATGGAATGGAAAACAATGGAAAGGAAAGGAAGGGAATTGAAAGGAAAGGAATAGAATGGAATGG
AATCGGATGGAACGGAATTGAATGGAATGGAAACTAAAGGAATAGAATAGAAAGGAATCGCATTGAATGGAAT
GGAATAGAATGGAATCAGATGGAACAGAAAGGAATGGAATAGAATCGAATGGAATGGCATCGAATGGATGGAA
TGGAATGTAATGGAATGGAATAGAAAGGAATGGAATGGACTCGAATGGAATGTACTCAAATGGAATAGAATAG
AATGGAATGGAAGTAAATATAATGGACTCGAATGGAATGCATTGGAATAAATTGGAATTGAGTGTATTGGATT
CGAATGGAAAGGAATGGAATGGAATGGAATGGAATGGAATGGAATGGAATGGATTCGAATGGAATGGAATCGA
ATGGAATGGAACGAATTGGAATGTAATTGAATGGAGTCAAAAACAGTAGAAAGAAATAAAGTTTCATCGAAAG
ATATCGAATGGAATTGAATGGAATGTACGCGAATGGAATGGACTGGAATGGAATGGAGTGACATGTAACGGAA
TCGAAAGGAATGGAATCCAATGAAATGGAATTGAATGGAATAGAAATGAATAGAATGGAATGGAGATTAACGG
AAAGATATTAAAATAATGGAATGGAATTGAGTGGACACGAATGGAATGGACTGGAATGGAAAGGACTCAAATG
AAAACGAGCGCAATAGAATGGACTCGAATGGAATGGATTGGAGTGGAATGGTCTCGAATGGATTGGAAAGGAA
TGGAATGGAAAGGAATAGAATGGAATGTAATCAAATGGAACGAAATGGAATGGAATGGATTCGACTGGAGCAG
AATTGAATGGAGTGGATTTGAATGGAATGGAATGCAATCGAATGGAATGGACACGAATCGAATAGAATGAAAT
GTAATGGCATAGAATGGAATGGAATGGAATGGAATGGAATGGAATGGAATGGAACGGAATTGAATGTCATGGA
ATGGAATGGCATGGCATGGAATGGAATGGAATGGAATGGAATGAAATGGATTGGAATGGGATGGGCCCAAAAG
TAATAGACTCAAATAAAAGGGACTCAAAGAGAATGAAGTGGAAAGAAACGGTCTCGAATGTAATTTATTCGAA
TAGAATGATATTGAATGGAATGCAATAGTATGGAATGGTATCGAATAGAATGGAATAGAATGGAATGGAATGG
AACGGAATGGAGTGCAATTGAACGGACTCAAATGCAATAAATTGCAATATAATTGATTCAAATGGAATGGAAT
CGAATAGAATGTAAACAAATGGAATGGAAGGCAATGCAATGGAAAGGAATCGAATGAAATGGAATAAATGGAA
TGGAATGGAATGGAAAGGACGCGAATATATTGGACTGTTAAGGAAAGGTGTCAAATCGAATTTATTCCAATAG
AATGGAATCGAATGGAATGCAATACTATTGAATCGAATCGAATGGAATGGAATTGAATGGAATGGACAGGAAT
GGAATGAACTGGAAGTGAATGGACAGGAACGTAATATATTGCAATGTAATTTATTCAAATGGAATGGAATGCA
ATCGAATGGAATGGACTCGATTGGAATGGACTGGAGTGGAATGGATTCAAATGGAATGGCAAGGAATGGAATG
GAATGGAATGGAAAGCAAAGGAATCTACTGGAATAGAATCGAACGGAACAGAAAGGAATGGAATGGAATGGAG
TGGAATGGACTCGAATGGAATGTATTCGAATGTAATGGACCTAAAAAGGAATGGAATCCAATGGAATGGAATT
GAATGGAATCAAAAGGAATAGAAAGGCATCGAGTGTAATTGAATGATATCGAAAGGAAGGGAATGGAATGAAC
TCGAATGGAATGCACTGGAATGGAATGGACTCGATCAGAACGGACTGGAGAGGAATGTACACAAATGGAATGG
AAACGAATGGAATGGAATGAAATGGAATGGAATGAAATGGAATTGAAAGGAAGGGAATCAAATGGAATGGAAT
GGAATGGATTGGAATAGAATGGATTCAAATAAAATAGAATCGATGGGAATGGTATTGAATGAAAGGACTTGA
ATGGAATGGAAAGCAATGGAAGATATTGGAATCGAATGGCATCGAATGAAATGGAATGGAACGGAATGGAACG

GAACCGAATGGAATGGAATGGACTCAAATGTAATGGACACCAATGGAATCGACTGAAATATAATAGTGTCGAA
AGGAATGGCCTCGAGCGGAATTTATTTGAATAGAATGGAATCAAATGGAATACAATACCATTGAATGGAATCG
AATGGAATGGAATCGAATGGAATGGAATCAAATGGAATGGAACGGAATTCAATATAATGGAGTAGAATGGAAT
GCATTGGAAAGGAGCAGAGTGGAATCAAGTGGAATGGAATCGAGTGGAATGGAATCGAGTGGAATGGAATCAA
TGGGAACAAAATCGAATTGAATGGACTTGAATGGAATTGACTCGAAAGGAATTGACTCGAAAGAAATGGACTG
GAACAAAAAGGAATCAAATGGACAGGAATGGGATGGAATGGACACGAATGGAATGGAGTCAAATGCAAACGCA
TCGAATGGAATGGATTGAAATGGAATGCAATGGAATGGAACAGAAAGGAAGAGAATGGAATTGAGAGTAATGG
AAAGATATCGATTGGAATGAAATGGAATGGAAAGGAATTGAATGGAAAGGAATGGAGTGGAAAGAAATGGATT
GGAATGGAATGGTCTCCAATGGAATGGACTGGAGTGGAATGGAATCGAATGGAATGAAAAGAATGGAACGGAA
TGGAATGGAAAGGAATAGAATGTTATGGAATCCGATTGGACAGAATGGAATGGAATGGAGTTTCATGAAATGG
AGTCGAATAGAGTGTCATCAAAAGGAATGGAATGGAATGGAGTGGACTCAAAAGGAATGGACTCGAAAGGAAT
GGAGTCCAACCAAATTGAATCAAATGGATTGGAGTCGAACAGAATGGAATGGAATGAAATGTACTCGACTGGA
GTAGAGAGGAATGTAAAGGAATAGAATGGAATGTAATCAAATGGATTGCAAGTGAATGGAATCAAAAATAATA
GAAAGGAATGGAGTGTAAAGGGATGATATTGAATATAATGGAATGGAATGGAATTTAATGGAATGGAGACGAA
GGAATGGACAGGAATGTAATGGACTCCAATGGAATGGAATGGATCAAAATGGATTTGAACAGATTGGAATCGA
ACGGAATGGAATGCAACGGCATGGAATGGACTCGAATGGAGAAGAGACAAATGGAATGGAAACGAATTCAATG
GAATTGAAAAGAATAGGATGGAATGGCGTGTAATGGTAAGATACTAAATGGAATGGAATTGAATGGAATGGAA
TGGACCCAAATGTAATGCACTCGAAAGGAATATACTCAAATAGAACGGAATCGAAAGGA

**Supplementary table** XIII: Chimpanzee consensus sequence for repeat unit 10762 bp.

```
CTCCAGCCCCCCACCCCCCGCCTTCCCTGCCCAAGCCTCCTCCGAGAAGCCCTTGGAGCTTGTGCCGGGTAGC
TAGGCATCCAGGCACACGCGGGCTGCGTGGCCTTTGGAATTGTGGGCATGGCAGCCCTGTGCCCTGACATCCT
CAGTGTGGCAAGCCATGAACATCTCTGTGTGTCACGAACACAGGAAACATCTCTCTTCGTTAGGCAGGCCAGG
TAGATGGTACGGAAGTAATACTGCAGATCCAGAGAAAACTCTCTGGTTCCTGGGGCTAGGGCGGCAGGGGTGT
CCTGGGGGAAGTGATCGGGGCGGGCACGTGGGAGGAAAGTCGCCTGCCTTATAAAAGATTAATCGTGAGGAGA
AAGTTATGCTTCGCATTACTACAAATACGCAAGTATGATTTCATCTAAAGCTGCAATCAGTCAATATAATTTG
TTTTTAATGTTTTATTTAAAATCCTTAATTTCAACAGGATTACTCAAGAAAAATAACGTTATTCGTATTAAAT
AATGTTGATGTATTCCCTTTAATTGTTGATTATTTCAAATGTACGTAAAATAGTAAATGGCACTGTACAATGT
AGTTTCATGAAGCATTCTTTATAGTTTTCATAAAATTGATAGTCTCCATGGAATATTTTAAGACTGAGGAAGT
TCCATATATCATTTTATTGTACTTTCACTTTGTTACTTCTTGCATGTCATAACTGATGGAAATAAAACTATGT
ATATTTACACATATGAAAAACATGGATTTTTGTTTACGTTTTCTAGTGAGAAAAAGTTACCAATAATTTTTCC
TATATAGGAATATTTTTACAAACCCAAAGTTCTAATCTGTCTTTTCTTTGAAGTTTCACATTTCAGTCTAGGT
ATGTAATGGAATTGGCTGGGATCATTCTTTGATTTCACTGTTATTTGTGAGTTTCTGATATGCTTTTAGGAAT
GTATAGAGTTTCAAGCTTGCTTTCTTCTTCTTCATCTACCTTTGGACCTGTATATGCGATGTCTGCAGTAATG
TGCAGTGCTATCTGACATACGGTTGCTGAAAGATACAAGCATATATACAATTCATTGTTTCAGTGAAGCTTGA
GGAACAGACAAGTAACCTGAGAGATAATTATGGTATGAATGTAAGCAAGCAGTTTATCATAGAGGTACAATAA
GGGTGAAAATAAATGTAAAAATACATGCCTCATCCAAAACATGAGGTAGTCAAAATGAAAAATTTAAGTTGGC
GTAAAGAACACTTTAAAAGTTCTGATTCTTTCTGGTGAGAGCAAGGAGCTCAGAAACCATGAGAAAGTCCTTC
AAAGCTGCATGTTGGATTTGCAGGTCAGGATGGAAAGCCTGGGTCTGGGGGAGGGTGCTAAGGTCCTGGTCTG
GTTGAGGTCCTTCTGGGGCTCAGGTGTGTCTCAGCGGGAAAGCTGGGAAGGGGAAACGCATGCTTCACCCCGG
CTAGAATGCCACCTCTGCCCACCTAGATGAAATTGCCCCTTCACAGCCCTGTTTCTCCTTCTTGGACAGGCAG
GTGGAGGAACTCGGCCACCCTGAATACAAGTGGTAGGAAGAAGTTTGCCTTTCATCACAACATTTACTTCGGA
AACAAAGTGATGACTAAGGAGTATTGCATTGGCATCCTCCATGAGGAGTAGAGGGGGTAGTACCTCGGAAGCT
GGGCCTGGCGTGAGCCTTCCTGACTCGTCTCCCTCCAGGATACAGGGCGACTGGCTCCACTGCAGTCCAGTGG
TTCCAGGGTCATGCAAGTGAAAGCCCGAGTTTCCCGCAGGTCACTGCCTGAGCTTCTTCAGCTGGTTGTCTGA
CTGTGACGGCCCAGGTTACGGCACGATTGCTGAGGTGGGGCAGCTATGGGGCATCATCGCAAAGGACCTTCTT
CAACATTCCTTGGCATCGGAGGAATTGGCTTTGAACCAGAACCTGACCTGTCACGGCCAATTTGCCCAGTCCA
CCAGATCATCAGCCAGGGCCTGTGGCTCTATATTCTGCAGCACTACCCAAGGGAGTTAGGCCCTCAGAGAGGG
AACAGAGAAGAGGCTAGGGAAGCAGCCCAGGGCTGGGGGTTGAGAGGCCTGTGGGTCCTGGAGGTAGGACACA
CATAGAGAAGCCAAGGCTCAGGGAGGAGACTGCAGTAAGGAAACTCAGGCCATCATGGGCTGGTGGAGAAATG
CCCATCAGGGAACTGTGGTACCCACATTTCACGATGGGGGAACCGTAATCTGCTTAATAGGCATAAGTAGCTA
AGGTCAATGGGTGGGAAGCCAGGATCAAGGGATAGCTGCCTCATCATCCCTTGCTAGCTACTTCCCTGTCCTG
AGGCTTGCTTCTACCTGGGGTTCAGTTTGGGCTCAACCAGGGATCTCTCACCCTCCACACAGATGCCCACCTG
AGGCCTGTCTAGGTCTGCGTCCTCCCAGAATGACTCTCCCAGGCCTGCTAAGTACCATCTGGATGACACCACG
CTCCACTGACATGCTTGCTTCCCTCCGCCATCCTCATTCACCCACCAACTCCCCACCCCAAAAAAGGCAGGCC
ACCGCACAGGGAATCTGGAGGATCACACAGGGCTCACAGGGGAGGAAATGTGAAGAGACGGCAAAACAGAACA
GGACATTCTGTGTGTTTCCAGAAGGCAATCTGCCTGGATATTAAGGCCCACCTCAGTATTGGTGAGGATACCC
AGTGTCTCTTGGCCCTGAGCATGTGCACACAAACACGCACATTGTCTAAACGGCATTGACATCACTACTACCT
GAGTCATCCTCAGATTCTATACAACCCCTGTAAAAATATCAATGACACAATCTTCTTAGAAAAACAATCTGGG
AATCCCAAATTTGCTATGAAATGGCAGAAGATCCTGAAAACCCAGAGCAATCCAGTAAAAAGCATAAAGCTGG
AGCCACCACACTACCTAACTTCATGATATACTACTACAAAACTTTTTGTACCAAAATACAATAGCACTGGCAG
AAAAGCAGAGACTAGAGCTCAGGAAAAACAATAGGAGCCCAGAACTAAGTCACTACATTTGCAGCTCACCGCC
TTTACCCGAAGAAGCAAGAACGCCCAATGCAAAATCAAGTATCTTCTATAAACTAGGTTGGGGAAATCTGAAT
AGCCACACAAAGGATTTTACAAGTGGATTATTTATCACCAAACTCCAGTGTCAGATCTGAAAGGATAAAAATA
GCAGAAGAGATCACAAGGAAGAAGCTCCATGGCGTCCGTGTGTTCAATGATGGTCTCAAAGTGACTGCAAGAA
CACAGTAAACACCATCAAAAACAGAGATTGGAATCATATCAAACTAAAGTGCTTCACCACACCATAGAAAACT
CAACATACAGAAGGGGCATCCTACAGGATGGGAGCAATGATTGAATAGTCACAGTACATAAGGAACTCCCAAC
AACTCAATAGCATGAAAACAAATGGGCGAAGGCTGCGAAGACTCATTTGTGAAACTGAGACATACAGTTGCCC
AGAAGACACACTAAAAGGTCCTCAGTATCCCCAATCCATCACGAAAATGCAAATCAAAAACACAATGAGATTT
CTTCTCACTTCAGTCAGAATGCATATTATCCGAAAGTCAAACAAAAAAGAAAGAAAAGAAAACCCTAATCTCT
GGTGAGGATGCAGAGAAAACGAATTCCCTGCTCACTTTTGGGGAGAATGTAAATTAGTGCTGGCATTAAAGAA
GCTTTATGGCTCTTATTTAAGTATAAACAGTCTTCAGAAATCTACAAGTAGAACCACCCACTATATGATCCAG
CAAATCAGAATACCCGGGCACGCCCACTAGTACACAGATCAGTATGTTGAAGTGGTGCGTGCACCCATGCAAT
TATTGCTGCACTCATTACGTTTTTGCTGTAGCCAAAATACGGAAGCAACCTGAGTGTCCCTCCATTGATAAAT
GGATTAAAAAATGCAGCAAAAACACGTATGCGCAATGGAAATATGTTGAATATGGGAATCTGCTGAATGTGTG
CATGCCATTCTGTTAAGTGACATAAGCCAGGTATCAGAAAGGAAAATAGCACATGATCTCATTCTTATATGAA
ATCAAAAAAGCGGACTTCAGAGAAGTAAGACTCCAAAGACTGCGGTGAAGAGGGTGCACTGACGAGATGCTGG
ATGAAGAACTCATACTTCTAGTTATAAAGGAGGAATAGGTTAAAAATATTTTCTTCAGCATGCTCACTATAAC
TAGTGGTAACATATTCTTTCTCTAAAAATATTTGAATACAGTGCATGCCATGTTTTTTCACAACAAAAATGAC
AACTATGTGAGGTCACACATATGTTGATTGGCTGGATGTATCCAATGCAGAATGTATATGACCTGTTGAACAT
```

CACGCCTTAAGTGGTAAATATGTATCATTTCATATGACATTTTTTAATTAAACCTACAATTTTTAAAATGCCT
TAACAAAATAAATGCAAATAAAATATTGTATTATAAAGCAGTGCTTTTCTTTTCTAGCAAAGTCTTTTTCATG
GCACAGGAAAGAATGCAAGCCTTTTGGTAACTTGAGAAATAAATACATTTGTGTACATGTATATATATATAATAT
ATACATGTATATACGTATATAAATGTGCATATATACGTATATACATGTATATACGTATATATGTGTGTATATA
TGTATTTTTATATATGTGTATATATATATGAAAATCCCTATGAATGCTGATGATGAGTTGAAAGATAGAAATT
CCAGGCACAGAGACTATAGTCCATGAATTGAAACCTTCAGTGCATGTTTCAAAACAAGACGTGAGGAGGAGGA
AGAAAAAAAGTAAAAAACACAAAGCCATGGCAGGTCCATGGGTTACACCTGTCATCCCAGCACTTTGGTAAGCT
GAGGTGGGAGGATTGCCTGCACTCAGGAGTTCCAGATGAGCCTGGGGCAACATGGACCCACATTCAAAAAGTA
AGTATTTAGTTAATTGGTACATAGCTTGGAGGGGTGGCATGCATCTGTACTGCCAGGTGTGTGAGAGTCTGAG
TTGAGAGGATCACATGGGTGTGTGGTGCCTGGGCTGCAGTGGGCTGAGATCGTGGGGCTGCTGTCCAACCTAG
AAGACAGAGTAAGACCCATTCTCGGAAAACAAACAAAAAACAGTCACATTAGGTAAATTAAAACTATGTAGTG
TGAGGAGAATCAAAATAAACGAAACATCATCAGAGCCTATGCGATCTGATGAAGGAAACCAGCTTTCACATAA
TAACAGCCCCAGCTGGGGAGAACAATGAGAAAGGGCAGAGAGAACACTGTAAATAATAACACGCCAAATTCCC
CAAATGAGTTAAAAGACATAAAAGTACAAAGAGTGCTTCTTTTCAATTCAATGCCCTTGAATTCAGAATTAGA
AAGTAAACCCAGAGAGAGAATAGAAAGATAGACGATACAGATGGAGAGCGTGTGTTGGGGAAGTAAGGGAAGG
ATGAAAGGAGGGGTGTAAAGGAAGGAAAGGAAAAAAGGAAGGGAGAGAGACTGATAGATGTTCAAAGACACAG
ATACAAAGTCTACAATGGTTGTAGAGATAGGCATGTGCAAATTGCCGCGGGGAGTGTGGAAAAAATATCGGAAC
CAACGAGACCTAGGTGGAGTCAGAGAAAATATACAAACTCGCACAGAGAAATAAACATACACAACCACAAACA
CACACGTGGTAGTTTAAACATGAAAAGACACCAAGTCCCTGTCGGTACAAATCACAGATGTGCTTCCGAGTTA
CTGAGGCACAATGCAAATTTGTCATTGCCCTTAGCATCTGTGGCCCATGTGCACGGATATTCAGTGGAAGAAG
TGTTACACAGCCTTTATAATTCAGCACGATCTGTGGTAATACCAGAAGAAGGGATCTCATGTGAAATCACTAG
ACTGAATTGCACGTAGGATTCAAGGAAGAAGCCCAGTCTGCTGCATTCACTCGGTGGGGTGGCAATATGGCTG
AGCCACCAACCCATGGCACGCCCATCCATTGTAGACAGTTCCTGGTTTGCTGCCTGCCTTGGAAAAAGCTCCT
CCCCTACCACCACTTTAAAACAGGCTAGCTCCAAAACTAGCCCTGGCATCCATTTACGGTCATTTTCTTATCT
ATTTACCTCCTAGAAAAATCATTGCAAGACCCTTTCCTCAACATTTTCCTATGCATTAAATTTGGGGAAACGC
ATTTTAAGACGACCTCGTTATAGGCAAGTCCCCAGACGTTTCCTAATCTGAGTTGCGCAGAGTGCACACACCA
ATCTGTTGCCCCATTGCCACTATACGGATACCGTACTGGACCACAGTGTCTTTGACATGCACACAGTAGGATA
GAGGGCAGCTTGAGGGGGCCAAAGAGTTCCGACTGTTTTCAGAATAATTTGCTTAGAAAACGTGTTTCTCCTG
TGTTTGTGGGTCAGGGGGACGGTAGTCAGGGAGGACAAGACTCCCGCTCCACAGCTTCAGCTGTCTGCATAGG
AGCAGGGACAAAACCGGGCGATAGATTTTCAAAGCTCAACTGCTTTGATACCGAGCAGAAGGGGTAGAATGCA
TACTGAAGGCACCACAACAGATTCAGGAACTTTGACTGTCAAACCCTCTTCCCTGAAACAACATAGCTCTTCT
CACAGAAGCTGTGCTGACAAGAGTCTATACGGGACAGGAATGTTAGCACTCTATTAGCGTGTGGTCAACATGG
ATGCTCATGTTGGAACTCTTTCATCTGGGAACAGGAAAGAAAGTTCTGCCTCCGACACTGAAATCCTCCTGCC
CCATCCTTGACAGAGGCAACCCCTTGTCTTGTGCATAGACACAGGTGTTCCTGGGAAGCAGCCTCCCACTCGC
GAATGAAAGCTGTATGTTTTGTCCTCCTGTGTGAGGCTTGCAACACATACTCTACAACTATATTTGCTTTACA
TTCTAAACCTTAGGCAAAGTATGCTGAAGAGGCCACAGAAAATTAAAGGGCCCTGGGCTCCAGAAACAATCTG
CAGTGCCAATCACGAGGGAGAATATAGAGACTCACTAGACTTTGCAAGAGCACAAAATGCACTCGTAGTGTTG
TTAGCTACATACGTTATGGGCTCCTCACCTAACATAGAATCTTGGAGAAAAGCTTAACCCAACTAAAGATGTA
AACATCCACAAGAGTGTCCATATCCAGGGTCATCAAGTGACAAGAGAGTCCCTGGATGGATTCTCCAACAATC
TTATATTCCACTAATCCACGCCCTTTCCCCTCACTTCTGTAAGTTTGTCTTTTCCCGTAGTCATCTATGCCAA
AAGCGTATCCTGAATGCCTTCCCACATGCCTCTGTCACCTTTCCCACAGTCCCTCCATACACCTTACATGCCC
ATTTCTTCTCACGTTGATGTTTCAGAAGTCCTGAGAGGCTGATTGTCCCAGAAAAGGATTATGCATTCACCTT
TGAAAGAACATGTGGATTCAACACGAAAGCGAACTTTAAGATTTCCATCATCCTGTGCTTATCTATTGTGTAT
GATGATACTCAAAATGAAGGATTTTGGAGGTCCCAGCAAACTGGGACCTGGAAACCCAGTAACCCCATTCCTT
GAACTATCTCTGCTTCCATAGGATGAAGTCAGCCTCCAACTAAGCTGTCTTTTGCTTTTACCTCCCCCACTCT
GTCCTGTAGGAAGAATCCCAACACATCCCACACCCATTCACTCTACAACTTTAGAGGCCCAGCTCCAACGCAG
ACTGGTAATTTCCATGAAGAGAATAAAGCACGTGGATGGATCAATTCATTATCACACCCGAATAAAGTGGATA
AACATACACACACACACACAAACACAAAGACACACTCACACACACACACAGACACAGAGTCACACATCCTTGA
GAATGTTTATTTTTCATTCCATACAATCCAAATTTACCCCCTCTTCCTGATTTCTGGTGACTCGATCTCTTTT
TCCTTTAGTTCCTGTGCATAAGACCATGCTGAGTACTGCCGTCCTGCATACTGTTGTAACTTTTTAGGAGTTC
TGCTGTATTAGGTAAAATCTGATGCTCCATCATATTCAACTCAACAACTGGGAGTCCCCTAGAGAAACACAAA
CTCACGTTAAAACGCATTTTCTCTGAGCCATACCTTGAAATGTTTCAATTGTGGGGCCCGCTGAGAAAAGGAT
ATCCCTTCCCCATTTGTGATCCCTTAAACTTCCTCCTACCACGTGTTACAAACTGTTCTGCGCAATCCCTGCC
CCATTCCCAGTATTGTCTGTGAGGGGAGTCAGCTAACAAGATGCACTGTACCCTAAAAGCACACAGAAGTCTG
ATGGGGCAACAGCTTAAGGAAATCCATCAATCTAAACAGTCCTTTGTGGTTTGGGGCAAGGATGATCAGGACG
CACATTCAGGGAGCCCAATCTTATGGGGTTGGTAGGATGACTGCCGGAGGGGGTTCACAGCCATGGAATCAAGT
GCCACAGACTGAACTGAATGATTTTCAGCTTTACTCCTCATTGATTCTGGAAATGGACGATTCTTCACTGGGC
TTAAGACTCCACAGCTATCACCTGCTTTGCGTGAAGTCTCTAATGTGCCTTTTCAGCCCAATGCCATGAACGT
CCTGGATTCTGTCACTCTCTGTCTTCCTCTCAAGGAATTTCTACATGTACCAAAGGAGCCTCAATTTCTACAT
TTCTGAAATGAGCACCCAGGCTCCCTGAATAGGCAGGTGCATCAACCCCCTTATACTAGGCATCAAACAGCTC
CAGTCCCAACTAACGGCTCACCTGACGTCTCTGTTCCCTCTTCAGGTGGCTTCATCCTCTTGTAGTATTGCAG
GGGATTGCGCCACAGCTCCTTACATAGGATCTGTCAGGGGACTCAATCGGGAAAGGCCTCATCAGGGCTCAGA

AAGGTGACCCAAGCAGCTGGGAACACATGGGGTCATTTCTCATGTTTCCCAGTGAGGACTCACCTCAGCAATC
TTGTTAGATCCTGCGAAGTTGTGGTCAGAGAACCAGTTGAAGAAGTTAAGGCTGCTGCTGTGGTGTCTGCGGC
GATAGGCCTCCACTTCATAATACGGATACCACTCAATTGGAGTGGAATGAGAAGCCCTGTATTCTACAGAGAC
AGGAGTTTTTGTGGGAAGGGGGCTGGATCACGTCGGCAATGATCCACCCGCCATCTTCCTTCCACTACCCATC
CTGGGAGCCACCTGTCACCTGTGATGTTCACCAGATATTCCTTGGTAATCACTTCATTCTGGAAGTAGGGGTT
ACTCCGAAAGAACAACATGATCTTGCAGAGATGAACAGGATGCTTCTCTTCTTCCACCTGTCAGGACAAGGTG
GAGAAAGCTTAAATACGTTTTCGGGTGAGGTGCTCACTCTTGCTTACAGGAATGAATTATTTCCCTTACCCTC
CCCCGCTAAACCCTCTAGCCTCAGTCTTCCTGGCCTCACCTCCAGGCTGACCATGTAGCTCAGCATGTCTTCA
TCTTCGTCAGTGATCAGGGCTGACATCTGGGGGTGGTTTGCAATCTGATTTAGGTCAAAGAGACTTTATACAC
GATGGAAGGGAAAGCGACGAGCAACAGGGAAGAAGGCCTAAGCGCACCCAGAGGCTGGGGTAGGGGATTTCTC
AGATCTGCTTCCATGTATGATCTCCTTTCACCTCCCCCTCCCCGTAAACTAAGGCCTCCTGTGTTCACAGAGG
GTGTATGATTCTGAGGCTGACTGCACTGACATGGGGAGGCGCGATTTGCAGAGACTTGCTGGTGTCTGAGGAG
TGGCAGAATCTGCTTAGAGCCGAAGACGCCCAGTCCCAGATCGGACTAGCAAGGGGCAGCAATCACACTCCCT
TAAAAATAGCTTGCTTCACCGAAAAACCTCTTCTGGTCTGAACTCGCTTCTGCTCTTCAAAAAGATGCCCCAA
ACGTCTGCTGCTCGGCATCACCAAGGGTTTCTCTGCCGCTTGCAGGACAATAGTACCCACGCCTGCTGTGGCT
TTCCGCAGCCACATTTGTCCGTGGCAACTCCCCTTTGTTCCCCAAAGAGTCACATCGACGCCGAGCTGCCCAT
CGGTCACTTACACTTCCCCGAGAGCACCTCTCCACTAGAAAGGCCGAAGAAACACTGAGAAGGATACAACATT
GGCCCAGAAGCCAGGGACGCTCTGGATGACGGCGCCTCTGCGGTCTAGGTGGGGCTTGCGCCTCCGCTCCATC
TTTTCCCGCTGCCGAGAAAAGGCCTTCCTGGCTTGGGCATTAACCGGCTCCAGCTCCACCTGAACGGCCAGCA
GCTCCTCCAGTGCAGACTCTGGGGTCATGGGCCCAGGGCCAGGCTGTGCCCGCTGGGCCTCCTCCTGCCGCTC
CACGAGGCCCTCCTCCTCCGCCACCACCTCCACCTCCGCCATTATGTCATCCAACAGCCGCACCGCCTCCTCC
CCCAAAGCCGCCTGCTCACTCTCCACCCCGGCCGCCCCCTCCTGTACAGCCTCCATCCTGAAGGCGGTGCCCT
CCTCGGCACTCGCACGCACCAAGGCCTGTGCTGCCCGACCCACGCCACAGGAACCCTGCCGCAGCCTCTATGG
CACCCGGTAGCTCAGCGAGCCCTCAGGGCGCATGCGCCGGGCTTCCAGGCGCCCCCTAAGGGACTGCGCGCGA
AGGGCCGAGGGGCCGCACCCAGGCCGACTTCCTCCCGTCGGGGCCAATCAATGGGAGGGCGGTGGGCGTCTCC
CTGGGCGGCACAGCCACTGGCGGGCCTGCAT

**Supplementary table** XIV: Human consensus sequence for repeat unit 20309 bp.

AGTCGCCCTGTATCCTGGAGGGAGACGAGTCAGGAAGGCGCACGCCAGGCCCAGCTCCCGAGGTACTACCCCC
TCTACTCCTCAGGGAGGATGCCAACGCAATACTCCTTAGTCATCACTTTGTTTCCGAAGTAAATGTTGTGATG
AAAGGCAAACTTCTTCCTACCCCTTGTATTCAGGGTGGCCGAGTTCCTCCACCTGCCTGTCCAAGAAGGAGAA
ACAGGGCTGTGAAGGGGCAATTTCATCTAGGTGGGCTGAGGTGGCATTCTAGCCGGGGTGAAGCATGCGTTTC
CCCTTCCCAGCTTTCCCGCTGAGACACACCTGAGCCCCAGAAGGACCTCAACCTGACCAGGACCTTAGCACCC
TCCCCCAGACCCAGGCTTTCCATCCTGACCTGCAAATCCAACATGCAGCTTTGAAGGACTTTCTCATGGTTTC
TGAGCTCCTTGCTCTCACCAGAAAGAATCAGAACTTTTAAAGTGTTCTTTATGCCAACTTAAATTTTTCATTT
TTACTACCTCATGTTTTGGATGAGGCATGTATTTTTAAATTTATTTTCACCCTTATTGTACCTCTATGATAAA
CTGCTTGCTTACATTCATACCGTAATTATCTCTCAGGTTACTTGTCTGTTCCTAAAGATTCACTGAAACGAAG
AATTCTATATATGCTTGTATCTTTCAGCAACCGTATGTCAGATAGCACTGCACATTACTGCAGACATCGCATA
TACAGGTCCAAAGGTAGAGGAAGAAGAAGAAAGCAAGCGTTAAACTCTATTCATTCCTAAAAGCATATCAGAA
ACTCACAAATAACAGTGAAATCAAAGAATGATCACAGCCAATTCCATTACATACCTAGACTGAAATACGAAAC
TTCAAAGAAAAGAAACATTAGAACTTTGGGTTTGTAAAAATTTTCCTATATAGATAAAATTATTGGTAACTGT
GTCTCACTAGAAAACGTAAACAAAAATCCATGTTTTTCATATTTGTAAATATACATAGTTTTATTTCCATCAG
TTATGACATGCAAGCAAGTAATAAAGTGAAAGTACAATCAAATGATATATGGAACTTCCTCAGTCTTAAAATA
TTCCATGGAGACTATCAATTTTATGAAAACTATAAAGAATGCTTCATGAAACTACATTGTACAGTGCCATTTA
CTATTTTACTGACATTTTAAATAATCAACAATTAAAGGGAATACATCAACATTATTTAATACCAATAACGTTA
TTTTTCTTGAGTAATCCTGTTGAAATTAAGGATTTTAAATAAAACATTAAAAACAAATTATATTGACTGATTT
CAGCTTTGGATGAAATCATACTTGTGTATTTGTAGTAATGCGAAGCATAACTTTCTCCTCACAATTAATCTTT
TATAACATCGGTGTTATAGTTTTCTCTGACACCAACATTGTGATATCGCACAGGTTTACTGCATGCATGCATT
ACATGCCTCCAGAGAGTAGGCTTCAAATATATGGAAAAATTATATTTATGAAAAAATTCTAGGAAAGGGAATG
GTGAAATGGAAGAGAATTTCTCACTTGCTAACTGTTGGACATGGATTTGTATATATTTGGATATAGACACATA
CTGGCACACTGTGAGTTTGCCCATGTATATATACACTTATATGAGAAACCCATAATATATGGGTTGTGTAATC
TTTTAATTAATCCATAATTGTATGTGTGTGAAATTAGATAAGCGGTTACCTTTTCTTTACTCAATTTGATGGA
AAGCCAAAAAAACTCTGTCCACCTTCATTTCAATTAATCCAATACTGTTAACTGCTGGTAGCTTCATTCTCCTT
GTTCTCTTACGGCAACCGGAAAGTTAATTCTCGCTCTAATTTGGCTTTCAAGGTGCGATCAACAAGAGTGTCA
CCTTGCTGTGGATTGTGACCTCTGACTCCACCTCTGTCTTCCTTTTGCAGTCCTACCTTTGCATAGGTAACAA
ACTTTGTACATGGTTAAAAGGATAAAAGTTCAGTGAAATGTCAAGCCATGCTGTGAAATGTTCCATAGTTTCT
ATATCTCTAATTGTCCTTTGATGTTATAGAGGCAAGAAAAAATAATTCAATGTTTTTCTTAGTATCTAGTCCAA
TGCACTCTTTCTTCATAATACTGCAAACAAGGCACTGACATGGAAACGTGGCTGGACGTCTCAAAATCTCTTC
TCATTAATTACCATTATGTTAATCACTGTTGCCCACAACTGGAATTGGACTTTGAAATCCCCTGGTGGAAATT
GCTATAATGGCTCAAACTACTGGAAAGACTATCTTTTTTTTACCTGAAAATATCTGATGAGCATAGACGTATG
CTATATACAGGAACATATTGTACATTAACAACATACCATCACTGCCACTCAATAATAGGTATCCCAAACCTTT
GAGCCAAACTGAGCTCAGGTGCTCCCACAAACCAAGCTTTTCCCTCCACAGATTTCTTATGTCAAAAAGCCAC
AACTCCAGGCCAGGCTTCGTGGCTCTTGTTGTAATTTCTACATTTTGGGAGGCCGAGGTTGGTGGGTCACTTG
AGGTCAGGAGTTGGAGACCAGCATGGGCAACATGGCAAAAAGCTGTCTCTACCAAAAATACAAAAATTAGCCA
GACCTAGTGGCACTTTCCTGTGGTCCCAGCTACTTGGGAGGCTGAGGCAGGAGAACCACCTGAACATGGGTGG
CAGAGATTGTATAGTAAGCCAAGATCAGACTACTGCACTCCAGCCTGGATGACACAGCGAGACCATGACTGAA
AAAAGAAAAAAAAAAAAATAAAGGCAACTCCACTCGTCCACTGGCTTAGGTAAAAAATACTGGAGTTGGCTGGG
CTCGGTGGCTCACACCTGTATTCCCAGCACTTTGGATTTTGGGAAGCTGAGTCGGGCGGGTCACCTGAGATCT
GTAGTAGGAGAGCAGCCTGGCCAACATGGTGAAGCCTGGCTTCTACTAAAAATACAAAACATTAGCTGAGCGT
GGTGATGCATGCTTGTAATCCCAGCTACTGCAGAGGCTGAACCTGGGAGGCGGAGGATGTGTTGAGCTGAGAT
CCTGCCACTGCGCTCCAGCCTGGTCTACAGAGCGAGAGTACCCTGTGAGAAACAAAGGTGAAGAGAACAAGAA
AAAAAAAAATGAGAAAAATAAGACCCACTGCAAAAGGTTGCCACAGAAAAGATTAAACATTTCAGCAACTTCTA
TCTTCTATCATGGAAGCCAAGGTTATTTGGACCAAACCTCCTGTCTTAGTTCATTTTCACGCTGCTGAAGAAG
ACATACCTGAAACTGGGAATAAAAGGAGGTTTAATTGGACTGACAGTTCCACATGGCTGTGGAGGCCTCAGAA
TCATGGTATACGAATAAAGGCACTTCTTACATGGCAATGCCAAGAGAGAATGAGGAAGAACCTGAGGCAGAAA
CCCCTGAAAAACCCATCAGATCCCGTGAGACTTCTTCACTGTCACAAGAATAGCATGAGAAAGACCGACCCCC
ATGATTCAATTACCTCCCCCTGGGTCCCACCCGCAACACGAGGGAATTCTGGGAGATACAATTGAAGCTGAGA
TTTGAATGGAGACACACCAAACCATGTCACTTCCCAAACAATTAAAAATTCCCAATAGAAGAAGCATTAATTA
TATCAAAAAGTGGTGGACCAAGAAGGAACTATTAGCCTCATATCTCAAGAAAGACTCCAGTCAAGGCCTAGGG
ACTACTCATGAAAAGAGTTTAATAGCCGACTCTCTCCCAGTGGATCTGGATTCCACCGGACTGTATCTTCACA
GTAAGGGTGAAACAGAAGCAAACCCATTCCTATTTCCAAGCTCAAGGAACTTTGGTCAAAGTTCTCTTGGAGC
TGAGCAGAACAAGGAGGCAAACAGAAAAGATTTGTGTCCCTGAGAAGTCATGGCCACAGGCTGGCTATCACAC
AGATTGTCAAGCCAGTTCCATATTGCATGGGTATTACAGAAAATCTCAAAACATAAATTTGTGTGTGGGTTGT
CCCAGAGTAGCAGGATCTGGCAGAAGGAAATTTCCTTCTAACCCTCAAAGAATCCACATAAATCTTGTTACAT
TTGGGATTTTACGATTTGCTTCAGGAATGAGAATGGCCTTAATTTTCATATCTTTTTCTACACTCAGTTTATG
GCTTGTTGGCGTCAAAGTTCTGCTTGCTTCACACAATGAGTTTAGGATTTTCCCTTTTTTATTCTATAGAATT
CTTCATATATATTGAAATGCTCTGCCTGGGGAAAAAAATCTGAGCCTAGCGTTTTATCTCTAGGAAGAATCCT
TTATTTCCTTGAACATTTATGAGACTATACAGATTATATATGTCTTCTTGTATCAATTTTACTAAGCTATATA

CATAGCTTATGTTTATATATTATATATATAAATGTAAGATACAAATATAAAAATTATGTATAAATATGAAAAT
ATATATAGAAAGCGATATATATGTCTATATATATAGACAGATTATAAATATCTGTCTATTTGACCTAAGTTTT
CAAATTTGTAGGTTAAGGTGTTAACGATATTTCCTTATTAGCTTCTTAATCTATGCTGTATCTATGGTTGTGT
ACCTTTTAAATTCTTAGTTTTATCTATGTTTTCTCCCTTTTTTTCTAAACTTGACTGACGGTTGCATCATTTA
TTATATTTCTCCAACAAGCAAAGGTTAGCTTTGTATGTTTTACTAATTTTGTCTACATCATTATTCCCACACT
TTAGTTTTTCAGAATTGATTCTGTTGTTTCTTTTCTAATTCTTTATTGAAATATCTAGTACATTAATTTTCAA
GTTATTAGAGAAATATTTGTCTGTAAACTCCTATTGTAATATCACTTTTCTTGCTACTCACAGATTTAATCTT
TAATATTGGCGGTATCATTGAGTTCTAAGTACATTTCAATTCCTAGTATGATAATCTATGAATTGCTGAGAAA
TAGTGTTTACAATTTTGTTGTTCTATTTCCACTTAAGTTTATTTTTACTTCTGCTAACTCAATTGAAAATTCT
TTACTAATTTTTAAAATCCTTGAACCCAAGAGATGGAGGTTGCAGTGAGCTGAGATCAGGCCACTGCATTCCA
GACTGAGTGACAGAGTGGAACGAGATTTCAAAACAAAACAAAACAAAACAAAACAAAACAGTCACTGGAAAGA
TAATAAAATACATAAATGTGGGATGTAATATGTAATCGTGATAAAATAAACTGGATTTTTTGTATAAGTTATA
CATATAAATGTAATGCCAAGACACTGATAAGACAACTCATGGTCTTATCTCAATACTTAGTGTCTTCATGTAA
CATATGTCCTTTAGGATAGTTATAGTCCGTTTTCTTTCCAGGAGAGACAGATGAGAATGCAGAAATGTTAAAG
TGCAAGGGACGGAAGCTTCCAGCTGTGCCCACCTGTAACCTGACGTAGACAGTTCCACCGTTTGCTTCATTAA
TCATGCCAAAGGCTCTAATGCAAATGTGGTACAGAGTCACATGTTTTTGTATCTACATGATAGAAACTATAAC
TTCATCCCTATATAGAAGGGTATATAGCATATGCCTCAGTGATAAATATAAGTGAATCATTGATCAGTAGGAA
ACCATTTTAAAAGTCTTTCATAACAGAACAAAATCCCTGAAAACATTTTCTTCTCAATCTCTGAGTTTTCTTA
CACGGCTTATGAATCTCTAGCCATACTAAAGAGATAGTATGCTGCTCTTCCCACAAATTATTCATTGTATATA
ATTCCTGTAATCTAATAACAGTACCTTTACACCTCAGGGTTTAAAATGACTCCAACCTTTTTCTGTTTCTCCA
ATTAAAATAACTTTTTTAAGGTTTAATCTTCAGTAATTTTTTGTAGTAATATTTTTGAAGGTATTTGACCAGG
ATGATTTGCTTATATACCTACCTGACGTCTCCCTTTCTTCTGAATACATATTTTATTACCCACCTATTAGATC
TAAGTTTAAGAAGTTGGAATAGGGATTTAAATCTAAATTCTACATTTGAATTTACAGGAGTCAGCGAGTCCGG
GAAGTGCCTTTATGCACAGACCAATATCTGGCAATGGCACTAGGAGACAAATAAGCTTTACCAGTCTCAAAGC
CCTGGCTACTACAGTGAATCCACCCTTCTCCTGGATCTTATCTACTTCAGCAAAAGAAGGCCACCCACTAAAC
CAGGCCCTTGTACTTTGGGTGGAAACTCCTAAGTCCTCTAGTCTCCTCAAACAGACAGCCAGGCTGCCAATTT
CCACAATAATAATTTCTATAGCACTGAGTCTTTGGTAGCCTTGTAACTATAGCTACTGATGCTACAGTCTGGT
CCCTGTATGATAAAACACCAGAGCAACAGAAACAAAAATATTGACTGAAGCCTTCTAAAATCTCTCTAAATAT
ACCTTCAATAAATATGGTTTTTTTTACAGAACGACTGCTTTCAGCTTCCTGAACTAACGCTTGGCCTTCGCTA
GTTGTCACTGTTGAAATTGATTCAAAAGTGTACATTTAACATGAAAGTCAACACAGAATTTCATGTGTCAGCA
ACTAAAATTTTCAAAATGTTGCAAAATACAAATGTGAAACTGTATTTGTGAAATTTACCATTCATTGAAATTA
TATTTTCATACCTACCCAGGCACAGAATTTTTTATAACTGTCTGCATGTTCTCCTCATGTGGGGGAAAAGCAG
CATCAGCAGGCAGAGGAATCCTTTGAAGCTGGAGGGAGAGGTTGCAGTGATCTGAGAGTTTGCCACTTGACTG
CAGCCTGGATGACACAGTGAGACTCCAACTGAAAAGAAACAAACACACACACACACACACACACACACACACA
CACCCCCAAAATTGATAAGTAAAAAAAAAAATCCATATTCGAAAACATGCTCACAGGCTAACTCCCATATCTAA
CACACACACACACACACACACACACACACACACACACACACAATTCCTTGAAAACGAAAGTTCCACAAGGGCAAA
ACAAGAAAACAAATTTAACACCCCCCAAAGAAAGTACAAAGAGTAACCTCAAAAGAACCGCAGGGGAAAACAA
TTCAAAATTTACAAGTATCTACCCTAAAAGAAGCTGAAAGTCCCTCAAAAACTTTCCAGAGGCCATGTCCTTG
TATTACAAAAATGATCATAAAAACTGGCAGGAGTAGACGAATAGAAATGCATCTTAAAACTTGCTAAACCCTT
CAAGTCTCCCATAAGAATTGTAATGGAAAATGGATCGGTCGGCAGCTTTTTCCATACAATTATGAACAAATTA
TATTTCTTCATACATAGATTTGTTTTTTCAATATTCTAAGGAATTAACTTTTATATTAATAGTAGGTGATGTA
AGAAAGCAGGCCTTTATCAAGATAACTGACACTGGATGTCCATACCATTACTCAGGTGGGCCTTAATTCCCAG
CCAGGTTCCCTCCCTGGACACACACTGAAGGTCCCCAGCCATTTGGCAATCTCTTCACATTCCCAGCCCTGGA
GGTAGCCCTAAAATACATGTACCTGAAGAAAATAAAACATTGCCTCACACTGGAGCCCAGTGTGGTCCTCCAG
ATTCCGTGTGAGGTGGACTAACTTATATGGGAAGGCAGGGCAGCGGGAGTGAGGATGGCAGAGAGGATTACAC
ATGTCAAGGCAGCCGGGGTCATGGAAACAAAACATGACTGGCCTGGGAGAAACACTGTGAAAGGACACACACC
TAGGTGGGCCTCAGGTGGACATCCTCGTGGAGAAAAAGGGGGCCCTGGTTGATCTCAAAATGAGCCCCAGGTG
GTAGCAGGTCTTACCGCAGGGCAGGGAGCTGGCGAGTAATGATGAGACAGCTATCCCTTAAGCCCTGCTTGTC
ACCCACTGACTTTAGCCACATATGCATCATAGTGGCTTAAGGTGCCCCGATCCTGAAATGTGGGTGTTACATG
TCCCTGATGGGCCTCTCTCCCCCAACCCACGGATTGCCTGGGATTGCTCACTGCAGTCTCCTCCCGGATCCTT
GGGTTCTCCATGTGGGGCCCAGATCCAGGTCAAAAGGCCTCTCAGTTCCCAGCCCTTCCCAGCCCTAGGCTGC
TCGCCTGGCCTCCTCTCTGTTCCGCCTCTAGGGCTGACCCTCTCTCCATGGGATAGAACTGCAATGGATTGAG
CCATAGGCCCTGGCTGATGATCTAGGGGACTGCAGAAGTGGGTCCAGGACAGTTCAGGTGACAGTTCAAAGCC
AATTCCCCAGAGACCAAGGAATGACCAGCTAGGTCCTTTCCCATGATGCCCCACGGCGAACCCCACCTCAGCA
ATCCTGCCAAAACCCGGGCAGTCATGTTCAGCCAAACAGCTGAATGAGCTCAGGTAGGAGGTGTACTGCCTGC
AGCTGGAGGCTTGACCTTCGTGATCCCAGAACCGCTGGACTGCAGTGGAATGAGACACCCTGTAGCCTGCAGG
GAGAGGAGTCAGGAAGGTTCATGCCAGTCCCACCCTCCCACACACCAGCTCCCCTACCATGCTGGGAGGCATT
CCTTACCGAGGATGCCAACACAGTGCTCCTTCATGATGATTTCACTGTGGAAATAAAGGTTGGGATGAAAGGA
AATCATCCTGCCACCGGTAACCGGGATGGCTGAGTTCCTCCACCTGCCGGATCAAGGAGAAAGAGGATGGATT
CAATGGGACCATCTCAACTAGCCGGGCTGAGGTGGCCTACTAGCTGTAGTGAACCATGAGTTTCCCCTTCCCA
GCTCTCCCACTGAGACAACCCTGGTCCCCAGGGGGACCTCAAACTGACTCAGACACTGGACTCCTCCCACAGA
CCCAGGCTCCCCAGCCTGACCTGCAAATCCATCACGTAGCAAAGCAGGACTTCCGCATGCTTTCCGACCCACG

CCGACATCTCGTGTGCCAAACAATCTACCTCTGCGCAAGAACTCTCCAGAGGATTGGGTGGGCAAGCCTCGTG
ACGCCTTGCAATTTCGCAAGAACACAGACAATGTGGAACAGGGCCATCTCCCAGACATTTGGCCAGTCACCCT
TCATTGTTGGCCCTCTATCTCTGTCTGGCGAGGAGGCAACGCCACAACTGTGGTGGTTTTTGGAGTGGGTGGA
CCCCGGCCAAGACGGCCTGGGCTGACCAGAGACGGGAGGCAGAAAAAGTGGGCAGGTGGTTGCAGCTGAGGGA
CGGGAGGGACCGGGGGTGGTGTGAGGCGGCTGCTTCTCTGAGTTTCTGAGATGCAGGAGGCCTTTGTGTGCTG
GGTGCTGGACATGCTCCGCTGATGTCCGGGTGTGTGGTGTCCTCTTATCCTAGTCTCCCTGAGGGGTGGGCCT
GTCCACCTGAGGGAAGCCTTGTAGTTAGAAGCCACAGCAGGGTCGTGCCTGGCGCTCTCCAAGGGAATTGCGT
GGGTCCAGAGGAAGTTATACAGGCTCAGGGCCTACACGCCTTTGAGTGCAGCGCCTGCAGTTGGATGAATGCG
CATCTGCGGAGCTGGTGCCCGCCGTCAGGTGGTCGGCAGCCCCATGCGCCGCGAACCCGTCTTAAGCACCTTG
TGTTTCTGGGGTGAGCCTGCTGGAAACAGGCACCGAGAGCAGGGGTGGTTCAATGGCTGGTAATGGCATACAG
ATTCCCCGTCCTCCAGGGACGTTCCCAGGGAAACGCGTCCTTCGAATTTGGGCTGTGCGCAAAGGGACCTTGG
CGCCGCGATTCTCCCTTGTCAGTGCTGGCCCTGGCTCCCCTTCCCTACCACGTGCTCCCAGGGCTGCTACAAG
CGAGCTGCCCTCACAGCTGCGGGAACGTGGCCTCGGCTCCCACGCTGTCCCCCATCCCCTGCCTCCTGGCTGA
CCCCACGTGCCTCCCACCTGGCTCCTCCCCCCAAACAGCCCCCATACCCCCCGAGGCCCGATGACTATCCCCT
GCTGCCCGCCATCCCAAATCGGCAGCCGCAAGGATATGGCTCTGGCTCACAAGGCGGAGATGCTCTGTGGCCT
GGGGCATTCACGGAGCCCAGCTCCAAGTGAAGGACCTCCAGCGAGTCCATTGACGGCCCCGGTGTGCTCGGTC
CAGGGCCAGGCTGTGCCCGCTGGCCCTCCTTCTGCCACCCCACGTCGGGCTCCACCTCAACCACCACCTCCAC
CTCAGCCATGATGTCTTCCACCTTCAGCACCGCCTCCTCTTCCAAGGCCGCCTCCTTGCTCTGTACCCCGGCC
GTCCTCTCCAGCATTGCCTCCAGCCTGAACACGGTTTTCTCCTGGGTGCTCCCACAGACCCTGGGCCTGCGCA
GCCCAGCCCAGCCCAGCCCATGCCCCGCACCCGTAGGCTCTGGGGGCCCGCTCCCCAGCAGACCCGCTCCCTG
CAAGACCCACGGGCGTCGCCCTGCTGTGAACCTGGTCCCACACCTACGTGGACCCAGGTTTCCTGAGGAGCTC
CGCTGGACCCGCAGATCCCGCACTGGCCAAAGGGCTCCGGTCCCCAGCAGGCTCAACTGCGCACAGGAGCTCG
GGAGCCAGAGGCCCCGGCCCTGGGCTTGCAGAGCCCCACCAACAGGCACCGCAACCGCTGCTGCGGGTGCGGG
AGCCTCTGGGTCGTCAAGGCAGCGCACAACAGCGTGCGCGCAGGCCGACAATGGCCAACCCTGGCGGCTGGCC
TCTGGTGTGCCCAGGGCATAGGACAAGAGGCCCCTTTGGAATGCTCCTTGGAGTACAGCATCCTCAGGGAGGAA
GCATGGTACTCGGAGCCTCTATTTGCCTCGACCTGTGAGAGTGTGTGCCGGGGCTCTGGCCTCTACAGCAGAT
CAATTCCACCTCAGCACCGGCAGGCGACTTTCCTCCCACGTGCCCGCCCCGATCACTTCCCCCAGGACACCCC
TGCCGCCCTAGCCCCAGCAACCAGAGAGAGTTCTCTGCATCTGCTGTATTACCTCCGTACCATCTACCTGGCC
TGCCTAACGAAGAGAGATGTTTCCTGTGTTCATGACACATAGAGATGTTCATGGCTTGCCACACTGAGGATGT
CAGGGCACAGGGCTGCCATGCCCACAATTCCAAAGGCCACGCAGCCCGCGTGTGCCCGGATGCCTAGCTACCC
GGCACAAGCTCCAAGGGCTTCTCGGAGGAGGCTTGGGCAGGGAAGGCGGGGGGTGGGGGGGCTGGAGATGCAG
GCCCGCCAGTGGCTGTGCCGCCCAGGGAGACGCCCACCGCCCTCCCATTGACTGGCCACGACGGGAGGAAGTC
GGCCTGGGTGCGGCCCCCCGGCCCTTCGCGCGCAGTCCCTTAGGGGGCGCCTGGAAGCCCGGCGCATGCGCCC
TGAGGGCTCGCTGACCTACCGGGTGCCAGAGAGGCTGCGGCAGGGTTTCTGTGGCGTGGGTCGGGCAGCACAG
GCCTTGGTGTGTGCGAGTGCCAAGGAGGGCACCGCCTTCAGGATGGAGGCTGTACAGGAGGGGGGCGGCCGGGG
TGGAGAGTGAGCAGGCGGCTTTGGGGGAGGAGGCGGTGCTGCTGTTGGATGACATAATGGCGGAGGTGGAGGT
GGTGGCGGAGGAGGAGGGCCTCGTGGAGCGGCGGGAGGAGGCCCAGCGGGCACAGCAGGCTGTGCCTGGCCCT
GGGCCCATGACCCCAGAGTCTGCACTGGAGGAGCTGCTGGCCGTTCAGGTGGAGCTGGAGCCGGTTAATGCCC
AAGCCAGGAAGGCCTTTTCTCGGCAGCGGGAAAAGATGGAGCGGAGGCGCAAGCCCCACCTAGACCGCAGAGG
CGCCGTCATCCAGAGCGTCCCTGGCTTCTGGGCCAATGTTGTATCCTTCTCAGTGTTTCTTCGGCCTTTCTAG
TGGAGAGGTGCTCTCGGGGAAGTGTAAGTGACCGATGGGCAGCTCGGCGTCGATGTGACTCTTTGGGGAACAA
AGGGGAGTTGCCACGGACCAGTGTGGCTGTGGAAAGCCGGAGCAGGCGTGGGTACTATTGTCCTGCATGCGGC
AGAGAAACCCTTGGTGATGCCGAGCAGCAGACGTTTGGGGCATCTTTTTGAAGAGCAGAAGCGAGTTCAGAGC
GGAAGAGGTTTTTCAGTGAATGAAGCTATTTTTAAGGGAGTGTGATTGCTGCCCCTTGCTAGTCCGATCTGGG
ACTGGGCGTCTTCGGCTATAAGCAGATTCTGCCACTCCTCAGACACCAGCAAGTCTCTGCAAATCGCGCCTCC
CCATGTCAGTGCAGTCAGCCTCAGAATCATACACCCTCTGTGAACACAGGAGGCCTTAGTTTACGGGGACGGG
GAGGCGAAAGGAGATCATACATGGAAGCAGATCTGAGAAATCCCCTACCCCAGCCTCTGGGTGCTCTTAGGCC
TTCTTCCCTGTTGCTCCTCGCTTTCCCTTCCATCGTGTGTAAAGTCTCTTTGACCTAAATCAGATTGCAAACC
ACCCCCAGATGTCAGCCCTGATCACTGACGAAGATGAAGACATGCTGAGCTACATGGTCAGCCTGGAGGTGAG
GCCAGGAAGACTGGGGCTAGAGGGTTTAGCGGGGGAGGGTAAGGGAAATAATTCATTCCTGTAAGCAAGAGTG
AGCACCTCACCCGAAAACCTATCTAAGCTTTCTCCACCTTGTCCTGACAGGTGGAAGAAGAGAAGCATCCTGT
TCATCTCTGCAAGATCATGTTGTTCTTTCGGAGTAACCCCTACTTCCAGAATAAAGTGATTACCAAGGAATAT
CTGGTGAACATCACAGGTGACAGGTGGCTCCCAGGATGGGTAGTGGAAGGAAGATGGTGGGTGGATCATTGCC
AACGGGATCCAGCCCCCTTCCCACAAAAACTCCTGTCTCTGTAGAATACAGGGCTTCTCATTCCACTCCAATT
GAGTGGTATCCGGATTATGAAGTGGAGGCCTATCGCCGCAGACACCACAACAGCAGCCTTAACTTCTTCAACT
GGTTCTCTGACCACAACTTCGCAGGATCTAACAAGATTGCTGAGGTGAGTCCTCACTGGGAAACATGAGGAAT
GACCCCGTGTGTTCCCAGCTGCTTGGGTCACCTTTCTGAGCCCTGATGAGGCCTTTCCCGATTGAGTCCCCTG
ACAGATCCTATGTAAGGACCTGTGGCGCAATCCCCTGCAATACTACAAGAGGATGAAGCCACCTGAAGAGGGA
ACAGAGACGTCAGGTGAGCCGTTAGTTGGCACTGGAGCTGTTTGATGCCCAGTATAAGGGGGGTTGACACACCT
GCCTATTCAGGGAGCCTGGGTGCTCATTTCAGAAATGTAGAAATTGAGGCTCCTTTCGTACATGTAGAAATTC
CTTGAGAGGAAGACAGAGAGTGACAGAATCCAGGACGTTCATGGCATTGGGCTGAAAAGGCACGTTAGAGACT
GCACTGCAAAGCGGGTGATAGCTGTGGAGTCTTAAGCCCAGTGAAGAATCGTCCATTTCCAGAATCAATGAGA

AGTAAAGCTGAAAATCATTCAGTTCAGTCTGTGGCACTTGATTCCACGGCTGTCAACCCCACCGGCAGTCATC
CCACCAACCCCATGAGATTGGGCTCCCTGAATGTGCGTCCTGGTCATCCTTGCCCCAAACCACAAAGGACTGT
TTAGATTGATGGATTTCCTTAAGCTGTTGCCCCATCAGACTTGTGTGTGCTTTTAGGGCCCAGTGCATCTTGT
TAGCTGACTCCCCTCACAGACAATACTGGGAATGGGGCAGGGATTGCGCAGAACAGTTTGTAACACGTGGTAG
GAGGAAGTTTAAGGGATCACAAATGGGGAAGGGATATCCTTTTCTCAGCGGGCCCCACAATTGAAACATTTCA
AAGTATGGCTCAGAGAAAATGCGTTTTAACATGAGTTTGTGTTTCTCTAGGGGACTCCCAGTTGTTGAGTTGA
ATATGATGGAGCATCAGATTTTACCTAATACAGCAGAACTCCTAAAAAGTTACAGCCATATGCAGGACGGCAG
TACTCAGCATGGTCTTATGCACAGGAACTAAAGGAAAAAGAGATCGAGTCACAAAAATTCAGGAAGAGGGGGT
AAATGTGGATTGTATGGAATGAAAAATAAACATTCTCAAGGATGTGTGACTCTGTGTCTGTGTGTGTGTGTGT
GTCTTTGTGTGTGTGTGTGTGTGTGTGTGTGTGTGTATGTTTATCCACTTTATTCGGGTGTCATAATGAATTG
ATCAATCCACGTGCTTTATTCTCTTCATGGAAATAACCAGTCTGCGTTGGAGCTGGGCCTCTAAAGTTGTAGA
GTGAATGGGTGTGGGATGTGTTGGGATTCTTCCTACAGGACAGAGTGGGAGAGGTAAAAGCAAAAGACAGCTT
AGTTGGAGGCTGACTTCGTCCTATGGAAGCAGAGATAGTTCAAGGAAAGGGGTTACTGGGTTTCCAGGGCCCA
GTTTGCTGGGACCTCCAAAATCCTTCATTTTGGGTATCATCATACACAGTAGCTAAGCACAGGATGATGGAAA
TCTTAAAGTTCGCTTTCGTGTTGAATCCACATGTTCTTTTAAAGGTGAATGCATGATCCTTTTCTGGGACAAT
CAGCCTCTCAGGACTTCTGAAACATCAACGTGAGAAGAAATGGGCATGTAAGGTGTATGGAGGGACTGTGGGA
AAGGTGACAGAGGCATGTGGGAAGGCATTCAGGATACGCTTTTGGCAGAGATGACTAAGGGAAAACAGAAACT
TACAGAAGTGAGGGGAAAGGGGGTGGATTAGTGGAATATAAGATTGTTGGAGAATCCATCCATGGACTCTCTT
GTCACTTGATGACCCAGGATATGGACACTCTTGTTGATGTTTACATCTTTAGTTGTTTTAAGCTTTTCTCCAA
GATTCTGTGTTAGGTGAGGAGCCAATAACGTATGTAGCTAACAACAGTACGAGTGCATTTTGTGCTCTTGCAA
AGTCTAGTGAGGCTCTATTCTCCCTCGTGATTGGCACTGCAGATTGTATCTGGAGCCCAGGGCCCCTAAATTT
TCTGTGGCCTCTTCAGCATAGTTTGCCTAAGGTTTAGAACGTAAAGCGAATATAGTTGCGGAATATGTTTTGC
AAGCCTCACACAGGAGGACAAAACATACAGCTTTCATTCGCGAGTGGGAGGCTGCTTCCCAGGAACACGTGTG
TCTGCACAAGACAAGGGGTTGCCTCTGTCAAGGATGGGGCAGGAGGATTTCAGTGTCGGAGGCAGAACTTTCT
TTCCTGTTCCCAGATGAAACAGTTCCAACACGAGCATCCATGTTGACCACACGCTACTAGAGTGCTAACATTG
CTGTCCCGTATAGACTCTGGTCAGCACAGCTTCTGTGAGAAGAGCTATGTTGTTTCAGGGAAGAGGGTTTGAC
AGTCAAAGTTCCTGAATCTGTTGTGGTGCCTGCAATATGCATTCTACCCCTCCTGCTCGGTGTCAAAGCAGTT
GAGCTTTGAAAATCTATCGCCCGGTTTTGTCCCTGCTCCTATGCAGACCTCTGAAGCTCTGGAGCGGGAGTCT
TGTCCTCCTCTGACTACCGTCCCCCTGACCCACAAACACAGGAGAAACAGGTGTTCTAAGCAAATTATTCTGA
AAACAGTCGGAACACTTTGGCCCCCTCAAGCTGCCCTCTATCCTACTGTGTGCATGTCAAAGACACTGTGGTC
CAGTACGGTATCCCTATAGCGGCAATGGGGCAACAGATTGGTGTGTGCACTCTGGGCAACTCAGATTAGGAAA
CGTCTGGGGACTTGCCTATAACGAGGTCGTCTTAAAACGTGTTGCCCCAAATTTAAGGCATAGGAAAATGTTG
AGGAAAGGGTCTTGCAATGATTTTTCTAGGAGGTAAATAGATAAGAAAATGACCGTAAATAGATGCCAGGGCT
AGTTTTGGAGCTAGCCTGTTTTAAAGTGGTGGTAGGGGAGGAGCTTTTTCCAAGGCAGGTAGCAAACCAGGAA
CTGTCTACGATGGATGGGCGTGCCACGGGTTGGTGGCTCAGCCATATTGCCACCCCACCGAGTGAATGCAGCA
GACTGGGCTTCTTCCTTGAATCCTACGTGCAATTCAGTCTAGTGATTTCACATGAGATCCCTTCTTCTGGTAT
TATCACAGATCGTGCTGAATTATACAGGCTGTGTAATGCTTCTTCCACTGAATATCCGTGCACGTGGGCCACA
GATGCTAAGGGCACTGACAAATTTGCACCGTGCCTCAGTAACTCGGAAGCACATCTGTGATTTGTACCGACAG
GGACTTGGTGTCTTTTCGTGTTTAAAGTAGCACGTGTGTGTTTGTGGTTGCGTATGTTTATTTCTCTGTGCGG
GTTTGTATATTTTCTCTGACTCCACCTGTGTCTCCGTGGTTCCGATATTTTTCCACACTCCCTGCGACAATTT
GCACATGCCTATCTCTACAACCATTGTAGACTTTGTATCTGTGTCTTTGAACATCTGTCACTCTCTCTCCCTT
CCTTTTTTCTTTTCCTTCCTTTACACCCCTTTTCATCCTTCCCTTGCTTCCCCACCACACTCTCTCCATCTGT
ATCGTCTATCTTTCTATTCTCTATCTGGGTTTACTTTCTAATTCTGAATTCAAGGGCATTGAATTGAAAAGAA
GCACTCTTCGTACTTTTATGTGTTTTAACTCATTTGGGGAATTTGGCGTGGTATTATTTACAGGGTTCTCTCT
GCCCTTTCTCATTGTTCTCCCCAGCCGGGGCTGTTATTATGTGAAAGCTGGTTTCCTTCATCACATCGCGTAG
GCTCTAATGATGTTTCGTTTATTTTGATTCTCCTCACACTACATAGTTTTAATTTACCTAATGTGACTGTTTT
TTTGTTTGTTTTCCGAGAATGGGTCTTACTCTGTCTTCTAGGTTGGACAGCAGCCCCACGATCTCAGCCCACT
GCAGCCCAGGCACCACACACCCATGTGATCCTGTCAACTCAGACTCTCACACACCTGGCAGTACAGGTGCATG
CCACCCCTCCAAGCTATGTATTAATTAACTAAATACTTACTTTTTGAATGTGGGTCCATGTTGCCCCAGGCTC
ATCTGGAACTCCTGAGTGCAGGCAATCCTCCCACCTCAGCTTATCAAAGTGCTGGGATGACAGGTGTGACCCA
TGGCCCTGCCATGGCTTTGTGTTTTTTGCTTTTTTCTTCCTCCTCCTCACGTCTTGTTTTGAAACATGCACTG
AAGGTTTCAATTCATGGACTATAGCCTCTGTGCCTGGAATTTCTATCTTTCAACTCATCATCAGCATTCATTG
GGATTTTCATATATATATATATATATATATATATATATATATATACATACCTATATAAGAATACCTATGTACACA
CATATATACGTATATACATGTATATACGTATATATGCACATTTATATACGTATATACATGTATATACGTATAT
ATATACATGTACACATATGTATTTATTTCTCAAGTTACGAAACGGCTTGCATTCTTTCCTGTGTCATGAAAAA
GACTTTGCTAGAAAAGAAAAGCACTGCTTTATAATAAAATATTTTATTTGCATTTATTTTGTTAAGGCATTTT
AAAAATTGTATGTTTGTTTAAAAAATGTCATATGAAATGATACATATTTACAACTTAAGGCGTGATGTTCAAC
AGGTCATATACATTATGCATTGGATACATCCAGCCAATCAACATATGTGTGACCTCACATAGTTGTCATTTTT
GTTGTGAAAAAACTTGACCTGCACTGTATTCGAATATTTTTAGAGAAAGAATATGTTACCACTAGTTATAGTG
AGCATGCTGAAGAAAATATTTTTAACCTATTCCTCCTTTATAACTAGAAGTATGAGTTCTTCATCCAGCATCT
CGTCAGTGCACCCTCTTCACCGCAGTCATTGGAGTCACTACTTCTGTGAAGTCCGCTTTTTTGATTTCATATA
AGAATGAGATCATGTGCTATTTTCCTTTCTGATACCTGGCTTATGTCACTTAACAGAATGGCATGCACACATT

CAGCAGATTCCCACACATTCTCACAACTGGCAGGATTTCCTGATTTCTTATTGCAGCGCATATTTCCGTTGCG
CATATGCGTTTTTGCCCCATTTTTTAATCCACTTATCAATGGAGGGACACTCAGGTTGCTTCCGCATTTTGGC
TACAGCAAAAATGTAATGAGTGCAGCAATAATTGCATGGGTGCGCGCACCGCTTCAACATACTGATCTGTGTA
CTGGCGGGCGTGCCCGGGTATTCTGATTTGCTGGATCATATAGTGGGTGGTTCTACTTGTAGATTTCTGAAGG
CTGTTTATACTTAAATAAGAGCCATAAAGCTTCTTTAATGCCAGCACTAATTTACATTCTCCCCAAAAGTGAG
CAGGGAATTCGTTTTCTCTGCCTCCTCACCAGAGATTAGGGTTTTCTTTTCTTTCTTTTTTTTTTTTTGTTTG
TTTGTCTTTCGGATAATATGCATTCTGACTGAAGTGAGAAGAAATCTCATTGTGTTTTTGATTTGCATTTTCG
TGATGGATTGGGGATAATGAGGAATTTTTAGTGTGTCTTCTGGGCAACTGTATGTCTCAGTTTCACAAATGAG
TCTTCGCAGCCTTCGCCCATTTGTTTTCATGCTATTGAGTTGTTGGGAGTTCCTTATGTACTGTGACTATTCC
CCCATGAACAGATGTATGGTGATCCAATCATTGCTCCCATCCTGTAGGATGCCCCTTCTGTATGTTGAGTTTT
CTATGGTGTGGTGAAGCACTTTAGTTTGATATGATTCCATTCTCTATTTTTGATGGTGTTTACTGTGTTCTTG
CAGTCACTTTGAGACCATCATTGCACACACGGACGCCATGGAGCTTCTTCCTTGTGATCTCTTCTGCTATTTT
TATCGTTTCACATCTGACACTGGAGTTTGGTGATAAATAATCCACTTGTAAAATCCTTTGTGTGGCTATTCAG
ATTTCCCCAACCTAGTTTATAGAAGATACTTGATTTTGCATTGGGCGTTCTTGCTTCTTTGGGAAAAGGCTGT
GAGCTGCAAATGCAGTGACTTAGTTCTGGGCTCCTGTTGTTTTTCCTAAGCTCTAGTCTCTGCTTTTCTGCCA
GTGCTATTGTATTTTGGTACAAAAAGTTTTGTAGTAGTATATCATGAAGTTAGGTAGTGGGGTGGCTCCAGCT
TTGTGCTTTTTACTGGATTGCTCTGGGTTTTCAGGATCTTCTGCCATTTCATAGCAAATTTGGGATTCCCAGA
TTGTTTTTCTAAGAAGAATGTGTCATTGATATTTTTACAGGGGTTGTATAGAATCTGAGGATGACTCAGGTAG
TAGTGATGTCAATGCCGTTTAGACAATGTGCGTGTTTGTGTGCACAAGCTCAGGGCCAAGAGACACTGGGTGT
CCTCACCAATACTGAGGTGGGCCTTAATATCCAGCCAGATTGCCTTCTGGAAACACACGGAATGTCCTGTTCT
GTTTTGCCATCTCTTCACATTTCCTCCCCTGTGAGCCCTGTGTGGTCCTCCAGATTCCCTGTGCGGTGGCCTG
CCTTTTTTGGGGTGGGGAGTTGCTGGGTGAATGAGGATGGCGGAGGGAACCAAGCATGTCAGTGGAGCGTGGT
GTCATCCAAACGGTACTTAGCAGGCCTGGGAGAGTCATTCTGGGAGGACGCAGACCTAGAGAGGCCTCAGGTG
GGCATCTGTGTGGAGGGTGAGAGATCCCTGGTTGAGCCCAAACTGAACCCCAGGTAGAAGCAAGCCTCAGGAC
AGGGAAGTAGCTAGCAAGGGATGATGAGGCAGCTATCTCTTGACCCTGGCTTCCCACCCATTGACCTTAGCTA
CTTATGCCTATTAAGCAGATTACGGTTCCCCCATCGTGAAATGTGGGTACCACAGTTCCCTGATGGGCATTTC
TCCACCAGCCCATGATGGCCTGAGTTTCCTTACTGCAGTCTCCTCCCTGAGCCTTGGCTTCTCTATGTGTGTC
CTAACTCCAGGACCCACAGGCCTGTCAACCCCCAGCCCTGGGCTGCTTCCCTGGCCTCTTCTCTGTTCCCTCT
CTGAGGGCCTAACTCCCTTGGGTAGTGCTGCAGAATATAGAGCCACAGGCCCTGGCTGATGATCTGGTGGACT
GGGCAAATTGGTCGTGACAGGTCAGGTTCTGGTTCAAAGCCAATTCCTCCGATGCCAAGGAATGTCGAAGAAG
GTCCTTTGCCATGATGCCCCATAGCTGCCCCACCTCAGCAATCGTGCCGTAACCTGGGCCCTCACAGTCAGAC
AACCAGCTGAAGAAGCTCAGGCAGTGACCTGCGGGAAACTCGGGCTTTCACCTGCATGACCCTAGAACCACTG
GACTGCAGTGGAGCC

**Supplementary table** XV: Chimpanzee consensus sequence for repeat unit 10853 bp.

CATACAGAAATACAGATTTCTAAATGAATGACTGACACGAAGAAACAAATATTCTCTGTCAAGTGCTACCCTT
TGGGCGGGGAGGGGGAAGAGACAAATCACAAAACAAGTGACTGTTGCACCGGCCAAAGTCCACCATATTTATA
CTGTGTACTTATGCCCACCCAGAAGTTATTTCTTACGCTGGTGATAAGGCTCTATTAAGACAGATTTCAACGT
AAGTTAAAATAATACATTTGCTCTTTCTCTGCCAAAATACTTCTAGACTGTTTGCTATCTGACGATATTATAG
GGTAATACTGTAGTTCTTCGACAGATGTTACGGCTTTCTCTGTACTTCATTTCCACAAATTAAGGGCAGTAAA
TAAGCCACAGCTGGAAAAGAGACAGTATAATGTCTTCTACTTTTCAATAAATACTTACTGATTAAAAACATAC
AGGTAGCATCATTCATCAATACACCCACATTCAGTAATGGCTCACAGTAAATGCTACAAACAAGTAGGGCTTT
TCTTCTAGCCATTGCTCAGAGAAGGAAAAAGAAGAAGAGGTGGACCCTACACGTTTCAAGTACACGGAAAATG
TCAACAAATGAGAGACACTGAAGAACTAATTCACTACTATTTGGTTACTTTATTTTCCATCGAAGAAAATCTC
TTTTAAACTAACACATAAATAAAATGAACGAAGAACAAACTAAACGTTATTTATCACCAGTAAGTGACAAGAG
TATGTCAAATCCTACTTTAAATATCAAAGCAACCAGCATCAGAGAAATTACATGCCAGAAACTCACGGGATTT
CTAGATAGAGCAAAAGAGATCAGAAATCTACCCATCCCAGAACCAGAATGTACCCAGAAGTCAAGCAATTTAT
ATGAGGAGGCATCTGGAAATCATTGCAAGTAAAGAATAGCTAGGTTAACTGCTAACCTTAGAGAACAATAAAC
TAGGCAGACACATAAGGAGGGCTGCTTCCAAATACTTTAGGAACTAGTTATATGAGGTGAAAGAGGCAGAGAT
AGGAAGAGATTTGTTCATGTGTCTACAGAGGTCATTTCTAAGAGAAAGCTTCGCCAAGTATACAGAAGATTCT
TAGCTCAAATGACGAACACGAAGAATAAGAAATTTCTAACAAAAGTAACAGATTTCCCGTTACTCACACTGTT
CAAACAGGGATTCTATTGCCACTTACTATGGAAAGTGTAGATACAATTCCACAGAGGGAAGGATGACTACAAT
AAACAAGAGAACAGGAACATAAGCAGTTCTTACCTGAACGTGCTGAGTTATAGGACTCGGCGTGATGTGGGGC
TGCAGGTAGGTTTCAGTGTTTGGATTCCGCCGGACGTTCTGAAACTGTGGTGGAGGAGGAGGATTAACTACCA
AAGGACGTGGCTGCACATGACGAGCACCTTTTTAAAAAGCAAGAAGAAAAAAGCCTATTTTTAGTTATTTGAA
AAGCTACACGGGTCAAAAAAGAACAATTTCGTTTCCTACTCACATAACTTTTGTTTCCTGATTGCAGGGCCCA
GCTTCAGCTTTTTACCATGGAAATGTATCTGTGACTGAAAATAGAACCGTTAACAAAACTAGAATCAATTTTC
AAGTGTTAGCTTCCAAGACTTGGGTAAACACCTGAAGTCTTCTAAAGTACCTAGCATCATAGAAGGTCGGGGA
CAACCACGCACCAAATTAAAATTTGTCATCACGAAGCTACCTTACTTACCCTTACTACTCTAATCAGTGTCAA
GAGGCATCAAGTGAAAGTTGATCAAAAACTTTCCATCACCCTGTCTCCAACCCTTCCTGTCTGTAGTTCATGA
AACTAGGTGTCCAGTCAAAAATAAGCAGGATCAAACAAGCTATGTGAGGTTACTCTGAGTTTGGATTTTGAAC
AGGAAGTCTGTCTTTCCCCAAATTTTACACAAGTCCGAGTATATCACTGACACTAAACGTTGTAGCAATAAGA
TAAATAAGAGATTTTTCTATTAGATTACTTACTCCTACTATCTTCTGGACATCCACGTCATTAACAAACGAAA
CAAATCCATAGCTATAAAGGCAGACAAATGAAGCATAAAATCACCATCATACAGCACGTGGTTCAGAAGTTCT
ACTCTTCTATATACAGAAGTGATCATGACAAAAGACGAATAGTATACCATGATAAGTGTTTGCTAAGATGTAC
ATGACAGATCCTCTACAAATACCACTTTTTCTTAAGCAGAACTATGTCAAAATGTGCTAGGATTAGGGCAGTG
TGAAAACTTTATTGACTAACAAAGAATTCATATCTGTGAACCTGAATTTAGCTTACTGTCTAAGACAAGGTGG
TTAAAATTTAAGATGCTGTGCAGTGTATGAAGAAAACAATTATTTGAGAAGACTGATTAACTCATCTGTATGA
AATAGAAACTGGAGACATTTAAAAACAAACATTAGAAAAATGGTCAAATAGAAGAACTGGTAATAGCCTTTTA
TCCCCTACGTGAAAGAAATTAACACTGCAGAATATTTCATTTATACAAGGGTCAGAATATCAGTTTTGAAGTC
TTGTCTGATACTTATAGAATAGGTGACTGGAGTTCACATATTTTTGATAAGATTACTCACCCTTTGGACACAC
CAGTTCGATTCCTGATTCTCTTCACTTCTTTCACTGAACCGTATCTACCAAAGAAGCTTCTAATCTCAGTTTC
ATCCGTCTATGGAAAAGAATTGAACGTCAGAGTAAAAATTCAGCATTCAAAAATTTCAACTTTACTACAATTT
TACTACCATGAGGTGGAAATTTCTCCCCCATTTATCCCCGAATGACCAGCAGCCCTTTGTCAAAGATATTTTT
AGTACCTATGGGTCAAACCTAAAAGCAATTCTAAACCTCCAGGAAGTACAAAAAAAAAACATTTAAGTTTGTA
ACAGGGCCCAAATCCCATTGTTCATGATGTATTTTAAGGTAAAAATGAGGTACGAATACAATACCCTATCATC
AATTCCACCAACAAAAACAGTGTTTGGCACGATTTTGCCTTCTGGTAACACCCAGCCTTGGCTAGCTGCAGCT
GATGAAGACTGGGTGCTGGCCTCTCTGGAGATGGTTGAGTTTGGAGTCTCAGGATTGGCAGCAGACTGTAATT
TGGAAAGCAGACATCATAATTACGTATGCAGGCAAAACCCATACGTAATGTGAAATACCATTTTTGTATTTTA
AGTATATTTTATATAAATTACTTTCATTGTAAATTAGTCACCAGTGCAGCTCAGTTCAGGCTCAGGATTTAAA
CTTATCAGAGTACATCAGCATGGAATTTTAACCGAAGGATACAGTACTTTCTTAAACCTAGTGCCGCTCATCA
CCGAGTCTTGTATAATGCTGTGGAAGAATACCCATTTAGTATTTGTGAAAGTACTGTGTGAAGTAGTTAAAAA
AGACACCCAAAACTAGAGAGTTTAGATTTGTAAAAATTAAAGTTATTAAAATCATCCTGTTCTATATTCATAA
ACAACTTTTCACTTTACTGAGTAGACTAAAGATAAATCTTAAAAAAAAAAAAAAAAAAAAAAAGCCCCACCAAA
AAGAAAATAAGCCTCAACGTTTTAAACCAATTTGTTGCAATCCTCTTCCCTAACGCTAGGGTGTTCAAAGCAT
CTTTTGAAATAACATTTTACTTCCTGAGTAACACGGAATCAGTCTGACTGATAATTCTGATTTTCACAGTGGG
CTGATAGATATAAATGATACCATCTTTATTTTCAGATAAAAAAACAAAGACATATAACTCACTAATTTTCTAG
ATTCTGATCAGAACTGTCTTTATTCTTTCCACAGCAGACTCTAAGGTTAATGTAAAATTTTCTGAAGTAGTAT
TCATAAGTAATACATACGTTGGAGAAACAATATAGCATAGTGAAACAAAAATTAATTCAGTCAGGAGGTCTAG
GTTTATGTCCCTTACACGTAAGTGGTTATAAGCCACCTACTTGCCAGCTACGTATCTGTGGGCAAAGTGCTTT
GAGAATGACATGAGATCACATCTGTGAATTCATTTTGTACGTATAAAGTGGTACAAGTGGTGTGCCAATGTAA
CTTAGTGTCCTGTTATTTGAATTTATTTTCAGCCGATTTGTTTTCAAGTTTCTTTTTTGGCTTCACTATTTAG
CTGACTTATTTTGAGAAAATTTTAATTAAGAACTAACTGACACATCAGGAAACTATGACACATCATTAATTTA
AAAATCATTGGTGAAGTGCTGTTGACTTCACAAATGTCAGTACAAAATGCTGCAAAAGAGAAAGCTATTACAC
ATATACCTGTCTGAAAGAAAACAAAAGACAAAAGAAACTGTGTTATCTTTTTGAACACAGTAATGTTACAGAA

GTTAATAAGAAAGGAGGGTTCCTGCTTTGTTAATTAGAGCCTAGAAGTTACTGATTCTACACAGCTTTACTAG
AGATGAAATCTAAATTGTCAAATCAACTAAAGCCGAGGTTACTGCATTTCTCTATTCTTTCGTGCTTGTACTT
GCTATTTTGGGTTTGTAACTAAGTCCTAATTCTTTCCTTTAACAGCGTTATTTCATGACAATGATGTGAAAGA
AAAATTTAAAACACTGTTTTTAAAGTTTTCCCTTTCAAAAATGTCTCACATTACTGTTTTTTTCCAAATGACA
TTAAGCTGCACTACCTTGAACTACTGGGAACCTGATTAGATCTCCCTTCCCTATAGACAATTTACCAATTCCT
TCTCCGTTCATTCAGAAATCCCAAACAGAATAAAACAAAACAAAACAAATTCTGAAATTCTTGTAGTTTCTTT
TTCTCCTTTCCAATTCCCCCTTGATTTGTGGATGAACTTTGGGTATGTGTTTCCTTGATAAACAAGCTATATG
ACAGTATTGTCTCGGCACCATAGTGTTTGGATGTATTCTAATTTAGAAATGTAACATCTGGCAGAAAACTGTG
TCAGACTATGAGAGGTTATGGAAATGCACTGATTCTCAACTGGGCAAGATTTTTGAGCCCCAGGGGCATTTAG
CGACGTTTAGAGATTGGCTGTCACAACTGAGATGTATTCCTGGAATCTGATGGGCCGAAGGCCAGGCACACTA
CTGCGCATCCTACAGTGTAAAGACAGCCTCCTACAACAAGGAAGTATTTGGTGCGCAATTTGAAAAGGGTCTG
GTTAAGAAACCTTGTCACCGTGCCACAAGAATTGAAGAGGAAAATTCTTCTTTGGGAAGAACCTGATTTCCAT
CGCTCACTAAAGTGAATCTTTTCATGACCTCGGTTTCAGCTTCCTTGCTTGAAAACGAATGGCCGGAAAAGAC
CTCGGGTGTCTCTTCTGATTCTCATACTCATTTGGATACGCGAAATAACCGTAGTTTGGTAAAGAAGAAAAAA
GGCACTTGATATGATTAAGAAGTTTGACTTTAGCTTGGATCTTACAAACCGGCTACCTGCTTAACTGGAATCG
TACATATAAAATTCACTGAATCTCTTTAATAGCGTCATAATACTTTAAATTAAGGAAGTAATGATCATGTCCT
AGTCCTCAGTCAGCAGGTGGCGCTCAAAGCTAACAAGGTTAAGCAATGTACTTCGTTTTCTGCAATGTACTTC
ACTTTTACCATGGCTCGAGTAGCAGGGATTGTTCAATTCCGACTGTGTACTTATACATAATTATATAACGCAT
ATATAAAAATCCACAATCAATAGACAATCTTTGGTTAGTTTTAAACTACGGCCAAAAATATAAATGAATGCTT
CGGATAAGCCAACGTTTAATTTTAAAGAAAGTACCATCGTAACCGTCAATGGCATCCTGAAAACAAACTGCAT
TAAAGAAGTAATTTTCTTAACCGTATCTTCAAGTGAGTTGTTGAATTTTCAAATGAGAAATGTTGCAATAGTA
AACAGGGGTGAGCTTCAACACCATCATACACGCAACTCTCACTGCTACATAGGGCAACTACATTCCTTGTTAC
ATGTGGACAACCAAGTGACAACGACAGCTATAGGCTGCAAAAAAAATTATCGTTATTTAAACTTCTGGCATGTC
AGCTCCTTTGCCAGTATTATCTAATTCAATTACTATGTCAACCTGTCAGCAAACTGATACTTATATAAACTGA
CCAGGAAAAAGTCTATCATTTGTAGTCAGCAAAGTTACATTCACAGCAATAGAAGAGAAGCAAATAAAGAGAG
TGATAAAATTAAGAAAATATGACATGAAAATCAGAATCAAAACCTTAAGCAAATCAAAGAGCAGATTCTCGGG
GAGTGGTGCGTGGGGAGGATGAAATTCAAGCAATAAACAATCCTGGCAAAACAAAGCAAGAAAACACAAGAAA
GCAAAAGTATACATGAGACCTGAAAAATGGGTTGCGGCCACAGATAATAGAAGAATGCTATGCAGAAACTCTA
TTTTCAATGAGGAATAAGGTATTTCTCAACGCGTTTTACAAAGCTAAAAGCATATAGGTAACAAAGCCTCATC
CAGATGATCCATCCCTGCCCTCAACACAAATGCAAAATTCCAGCAGTATATAAAGAGTCTAAGTTTACATTGG
GAATGCAAGAATACTCCATTCGCAGGATACATTACTTTAGTTCATCACTGAAAATCATTTGATAAAATACAGC
ACTCATAATTTAAATTTTTTAAAAACCCAAGTAAACTAGAGGTAGAGGAATCTTATTTTCTATCAATCTCATT
CTACCCTATCATCAAGCTTACAAGTGAAATAGTTGAGTCAACTCAATTGAAAGTAGGAATGAGGTAAGGGCAC
CAGGGCACCTCCTTATTACTCCTACATATGTTTTCCACTGTGTATGACAAAAGTGAATACTAATACAAAGTAT
TCTTATGAATCAGTAAGAAAATAAAATTAAAAAGGTAATTTTTAAAAAGCTAAAGATCAATGATCAACTTCAA
TGACGATTTTTAAAAGTGCACATCAACATAATGTAATATTTTCCAGCTATTAGGCTGACAATTTAAAAAATAC
TAGTAACTTTCACTGGAATGGGTGTGGAAAAGAGAGCACTCTACACACCATCAGTGAGAAAATACTAATACGT
GATTTACCAAGAGTACTTTGGAAAAGCTGTATCATAATTTGATAAGCGGGGATACTCACCACTATACTAAAAA
GGAGAATTCATTATAAAATTGTTATACAAGGGGCAAAGTGCTTTCACCTAGCAATTCCACTTATAGCAATTCA
TCTCAAGAAATTAATAGTACAAGCGTGCCAAGATATTTACACAAAGATATTCACAGCGTTGTTCTTTTTGAGA
CTGAGTCTCTCTTTGCCGCCTAGGCTGGAGTGCAGTGGCACAATCTCAGCTCACAGCAATCTGCGCCCCAGGA
TCACGTGATTCTGCTGCCTCAGCCTCCCGAGTAGCTGGGATTACAAGTGTGCGCCACCACGCCTGGCTAATTT
TTCTGTATTTTTAGTAGAGACAGGAAACAAAAATCATCCAAATATTCCTTCACATTTTCAAAAACACATGAGA
TAACACAACATTGAAGTACATACGCTGGTTCCTTTAATTTGTTATTATAATAAAAGAAACAGAATGGAAAAAA
GAATTACTTCAAGTTTCTAATCCCTGACGTTCTTGTTGTTACTTCTATATGTAAAACCTCAACTTTTTCCCAA
TTTTCTGGGGTTGGTATTGTGGAAATCTCGAGGATATTAGTTCTTTGAATGTATTACCATAGATATGATCATG
GGTCATATATACAGTCATATCTATGAAAAGAGACACAGAGGACTACTATTGTGAAGCAGCCAGCTAAAATAAA
AATATAATTCAAATTCTGTGCTCTAAAAAGTGGGTAATAATTTTATTTCACTCTGTCTCTCTAAAAAAACTGAT
AAAAGTCAGTCTGGATGTTTCGGCTATTTGACGGCAAAGATTAAAAAAAAAAAAAAAAAAAAAAAACACATGCTA
CAATATAGAAGGGGACACCAAATCTCAAAAAAACGATTCTACATTAAAGTTTTTGCTAAGTACACTCCTGTCAA
AATATTACTCAATTACTTCTAAATAATACAGAGGCCTTCATTCTAGACTAATTTGAAGTGTTGTCTTAAATTT
TAGGTACATTTCACTTCTTTAAAATGGCAAACTATTCAAGCAATTTGTATAAACAAAGGGCTCAATAATATCT
GAAAGTAAATCATTTTACTCCCTCTTAAATTACCTGATAATTATATACAGGCAAATGATATCTAGTGATGCCG
TGAACTGCTGAATTTGGGTAAGTAGTGTGTGCCTATAAATAAAGTTTACAGTAAGAATGAATGAATACGGTAA
AAGATTTTGTTAATTAGAAATACTATTCCCAATATAAAAAACTATGAAAAAGTTTTAAAACATTACTTTTCTA
TATACAGCACTGCAGAATTCTAAATGAGTGACTGATTTTATGAAGAAAGAAATATTCTGTCAAGTGAGGCCCT
TTGGCTGGGGAAGGGGAACAGACAAATGACAAAAGAAGGGACTATTTCACCAGACAAGTTTACCTTATTTATA
CTGTGTACTTACGCCCGCCCAGAAGTTATTTCTTACGCTGGTGATAAGGCTCTATTAAGACAGACTTCAACTG
TAAGTTAAATTAATCCATTTGCTATTTCTTTGTTAAAATACTTCTAAAGGGTTTTCTATTTGACAATATTATA
GGGTAATATGAAGTTCTCCTACAAATGTTACGGCTTTTTCCGTACTTCATTTCAAAAAACTAAGGGCAGTATA
TGATCCACAGCTGGAAAAGAGACAGTATGGTGTCTTCTACGTTTCAATAAATACTTACTGATTGAAAACTATA
CGTAGCATCACACATGAATACACCCAGATTACATAATGGCTCACCGTAAATGTGAGAAACAGGGCTTTTTTC

TAGTCATCGTTCAGAGGACAAAAAAGAAGCAGAGGTATACCCTACCTGTTTCAAGCACATGGAAAACGTCAAC
AAACGAGAGACACTGAAGAACTATTTCACCACTATTTTGTTACTTTATTTTCCATCAAAGAAAATGTCTTTTA
AACTAAGACATCAATAAAACAAACTAAAAAGAAAATAAACGTTACTTATCCCCAGTAAGTGACAGAGTATGTC
AAATCCTACTTTAAATATCAAGGTAACCAGCATCAGAGAAATCACATGCCCGAAACTCATGGGATTTATAAAT
ATAGTAAAACACATCAGAAATCTACCCATTCCAGAACCAGAATATATCCAGAAGTCAGCAATCTATATGAGGA
GACGTCTGGAAATCATTGCAAGTAAAGAACAGCTGGATGAATTGCTAACCTTCGGGAAGAATAAACTAGGCAG
ACACACAAAGACAGCTGCTTTCAAATATTTTCGGAACTAGTTATGTGGGGGGAAAGCAGTTCGGGTGTTTTAG
AGGTAATACTCTTTTTTCTTCCTACTCTTATTTAAGAGTAATTAATAGCAAAACATTTCTGTTCCTCTTAAAC
ACTTTTTTTTTTTTTTTTTTTTTTTTTTTTTTTTTTTACGGAGGGTAAAGCCAGAGGCAGATTCCAGGCAGAT
ACATGCTCATTCTAAAGCCACTATTAATACTACCTTTCATGGAGTGTATAGTCTATCAAAAAGTTACTGAATT
CTTATCATTATGTGTACGAGCCATTCCTTAAGCATGCAAAAACCTGACAGAGAAAAAGGCACTGTTGCTCCCA
TAGGAGTTTAAAATTGGGTTAAAAAGAAAGTAACAAAATGTGCCACATTAATACAAAGAACGATTTAAAAAAT
TTATAGGCATATATGACATAGAAAAAAAAGAAAGAACAGGGAGTATAGGTTCGGCGCATTCACTTTATCTGAG
GCACAGCGTAACTCCTTTGCTCCCCAACAGGCCACTGTGGTGGCAACTTGAAAAAAAAAAAAAAAAAAAAGGA
AACCAATATTATTCAAATATTCCTGTACTTTTTCAAAAACACATGAGATACATAATATTGGAGTATTTATCAT
GATGGCTCCTTTGTTATAATAAAAGAAACAGAATAGAAAAAAGAAGTACTTTAGGTTTCTAATCCCCAAAGTT
CTTGTTGTTACTTCTACACAGAAAACCTCACCTTTTTCCCAATTTTATGGAAATAGAATTGTGGAACCCTCAA
AGATATTAATTCTTTGAATTTGTTACCACAGATACAATTATGGGTCACAGATAATAGTTGTACCGTTGAAAAG
AGACCCAGAGAACTGCTATCATGAAGCAGCAAGCTAAAATAAAAATACAATTGGAATTCTGTGCTCTAAGAAT
TCGGTAAAGCTTTTATTTCACTCTGTATCTCTACAAGATTCATGAAAGTCAGTCTGGATGTTTCAGCTCTTTG
ACAGCAAAGATAACAAAATACATGCTGAAACAAAGAAGGGAACACCAAATCTCAGAAACTGTTCTGCAGAAAA
GTTATTGCTAAGTACCCTCCTGTCAAAATCTTATTTCATCACTTCTAAATAAAACAGAGGTCCTCATTACACT
AATTCTAAGTGATTTCTTAAATTTTAGGTACAGTTCACTAGTTTAAAACGACAACCTATTCAAGCAATTTGTA
TAAGCAAGTTGAAGGCCTCAATAGTAGCTGAAAGTAAATCATTTTACTCCCTCTTCAATCACCTGATAATTAT
ACACAGGCAACTGATACCCAGTGATGACCTGACCTGGTGAGTTTGGATAAGGAGAATAAGCCGAGAATAAAGT
TTACAGAAAGAATGGATTAATACGGTAAAATGTGTTTGTTTGTTTTTTTTTAACTAGAAAGCAATATCATTCC
CAAAATAACAAAAATACGAAAAACCTTGAAATGGTAATTATTTTTCTAC

**Supplementary table** XVI: Human consensus sequence for repeat unit 10848 bp.

```
GTACTTTAGGTTTCTAATCCCCAAAGTTCTTGTTGTTACTTCTACACAGAAAACCTCACCTTTTTCCCAATTT
TATGGAAACAGAATTGTGGAACCCTCAAAGATATTAATTCTTTGAATTTGTTACCACAGATACAATTATGGGT
CACAGATAATAGTTGTACCATTGAAAAGAGACCCAGAGAACTGCTATCATGAAGCAGCAAGCTAAAATAAAAA
TACAACTGAAATTCTGTGCTCTAAGAATTCGGTAAAGCTTTTATTTCACTCTGTATCTCTACAAGATTCAGGA
AAGTCAGTCTGGATGTTTCAGCTCTTTGACAGCAAAGATAACAAAATACATGCTGAAACAAAGAAGGGAACAC
CAAATCTCAGAAATTGTTCTACGGAAAAGTTATTGCTAAGTACCCTCCTGTCAAAATCTTATTTCATCACTTC
TAAATAAAACAGAGGTCCTCATTACACTAATTCTAAGTGATTTCTTAAATTTTAGGTACAGTTCACTAGTTTA
AAAGGACAACCTATTCAAGCAATTTGTATAAGCAAGTTGAGGCCTCAATAGTAGCTGAAAGTAAATCATCTTA
CTCCCTCTTCAATTACCTGATAATTATATACAAGCAACTGACATCCAGTGATGACCTGACCTGGTGAATGTGG
ATAAGCAGAGTAAGCCTGAAAATAAAGTTTACAGAAAGAATGGATTAATACGGTAAAACATTTTCTTTAACTA
GAAAGAAATATCATTCCCAAAATAACAAAAATACGAAAAACCTTGAAATGGTAATTATTTTTCTACATACAGA
AATACAGATTTCTAAATGAATGACTGACATGAAGAAACAAATATTCTCTGTCAAGTGCTACCCTTTGGGCGGG
GAGGGGGAAGAGACAAATGACAAAACAAGTGACTGTTGCACCGGCCAAAGTCTACCATATTTATACTGTGTAC
TTATGCCCACCCAGAAGTTATTTCTTACGCTGCTGATAAGGCTCTATTAAGATAGATTTCAACGTAAGTTAAA
ATAATACATTTGCTCTTTCTTTGGCAAAATACTTCTAGACTGTTTGCTATCTGATGATATTATAGGGTAATAC
TGTAGTTCTTCGGCAGATGTTACGGCTTTCTCTGTACTTCTTTTCCACAAATTAAGGGCAGTAAGTAAGCCAC
AGCTGGAAAAGAGACAGTATAATGTCTTCTACTTTTCAATAAATACTTACTGATTAAAAACATACAGGTAGCA
TCATTCATCAATACACCCACATTCAGTAATGGCTCACAGTAAATGCTACAAACAAGTAGGGCTTTTCTTCTAG
CCATTGCTCAGAGAAGGAAAAAGAAGAAGAGGTGTACCCCACACGTTTCAAGTACATGGAAAATGTCAACAAA
TGAGAGACACTGAAGAACTAATTCACTACTATTTGGTTACTTTATTTTCCATCGAAGAAAACCTCTTTTTAAA
AACTAACACATAAATAAAATGAACGAAGAACAAACTAAACGTTATTTATCACCAGTAAGTGACAAGAGTATGT
CAAATCCTACTTTAAATATCAAAGCAACCAGCATCAGAGAAATTACGTGCCAGAAACTCACGGGATTTCTAGA
TAGAGCAAAAGAGATCAGAAATCTACCCATCCCAGAACCAGAATATACCCAGAAGTCAAGCAATTTATATGAG
GAGGCATCTGGAAATCACTGCAAGTAAAGAATAGCTAGGTTAACTGCTAACCTTAGAGAACAATAAACTAGGC
AGACACATAAGGAGGGCTGCTTCCAAATACTTTAGGAACTAGTTATATGAGGTGAAAGAGGCAGAGATAGGAA
GAGATTTGTTCATGTGTCTACAGAGGTCATTTCTAAGAGAAAGCTTCGCCAAGTATACAGAAGATTCTTAGCT
CAAATGACGAACACGAAGAATAAGAAATTTCTAACAAAAGTAACAGATTTCCCGTTACTCACACTGTTCAAAC
AGGGATTCTATTGCCACTTACTATGGAAAGTGTAGATACAATTCCACAGAGGGAAGGATGACTAGAATAAACA
AGAGAACAGGAACATAAGCAGTTCTTACCTGAACGTGCTGAGTTACAGGATTCGGCGTGATTTGGGGCTGCAG
GTAGGTTTCAGTGTTTGGATTCCGCCAGACGTTCTGAAACTGTGGTGGAGGAGGAGGATTAACTACCAAAGGA
CGTGGCTGCACATGACGAGCACCTTTTTAAAAAGCAAGAAGAAAAAAGCCTATTTTTAGTTATTTGAAAAGCT
ACACGGGTCAGAAAAGAACCATTTCTTTTCCTACTCACATAACTTTTGTTTCCTGATTGCAGGGCCCAGCTTC
AGCTTTTTACCATGGAAATGTATCTGTGACTGAAAATAGAACCGTTAACAAAACTAGAATCAATTTTCAAGTG
TTAGCTTCCAAGACTTGGGTAAACACCTGAAGTCTTCTAAAGTACCTATCATCATAGAAGATCGGGGACAACT
ACGCACCAAATTAAAATTTGTCATCACGAAGCTACCTTACTTACCCTTACTACTCTAATCAGTGTCAAGAGGC
ATCAAGTGAAAGTTGATCAAAAACTTTCCATCACCCTGTCTCCAACCCTTCCTGTCTGTAGTTCATGAAACTA
GGTGTCCAGTCAAAAATAAACAGGATCAAACAAGCTACGTGAGGTTACTCTGAGTTTGGATTTTGAACAGGAA
GTGTGTCTTTCCCCAAATTTTACACAAGTCCGAGTGTATCACTGACACTAAACGTTGTAGCAATAAGATAAAT
AAGAGATTTTTCTATTAGATTACTTACTCCTACTATCTTCTGGACATCCACGTCATTAACAAACGAAACAAAT
CCATAGCTATAAAGGCAGACAAATGAAGCATAAAATCACCATCATACAGTACGTGGTTCAGAAGGTCTACTAT
TCTATATACAGAAGTGGTCATGACAAAAGACGAATAATATACCATGATAAGTATTTGCTAAGATGTACATGAC
AGATCCTCTACAAATACCACTTTTTCTTAAGCAGAACTATGTCAAAATGTGCTAGGATTAGGGCAGTGTGACA
ACTTTATTGATTAGCAAAGAATTCATATCTGTGAACCTGAGTTTAACTTACTGTCTAAGACAAGGTGGTTAAA
ATTTAAGATGCTCTGCAGTGTATGAAGAAAACAATTATTTGAGAAAACTGATTAACTCATCTGTATGAAATAG
AAACTGGAGACATTTAAATACAAACATTAGAAAAATGGTCAAATAGAAGAACTGGTAATAGCCTTTTATCCCC
TACGTGAAAGAAATTAACACTGCAGAATATTGCATTTATACAAGGGTCAGAATATCAGTTTTGAAGTCTTGTC
TGATACTTATAGAATAGGTGACTGGAGTTCACATATTTTTGATAAAATTACTCACCCTTTGGACACACCAGTT
CGATTCGTGATTATCTTCACTTCTTTCACTGAACCGTATCTACCAAAGCAGCTTCCAATCTCAGTTTCATCCA
TCTATGGAAAAGAACTGAACGTCAGAGTAAAAATTCAGCATTCAAAAATTTCAACTTTACTACAATTTTACTA
CCATGAGGTGGAAATTTCTCCCCCATTTATCCCCGAATGACCAGCAGCCCTTTGTCAAAGATATTTTTAGTAC
CTATGGGTCAAACCTAAAAGCAATTCTAAACCTCCAGGAAGTACAAAAAAAAAATTTAAGTTTGTAACAGGGCC
CACATCCCATTGTTCATGATGTATGTTAAGGTAAAAATGAGGTACGAATACAATACCCTAGCATCAATTCCAC
CAACAAAAACAGTGTTTGGCACGATTTTGCCTTCTGGTAACACCCAGCCTTGGCTAGCTGCAGCTGATGAAGA
CTGGGTGCTGGCCTCTCTGGAGATGGTTGAGTTTGGAGTCTCAGGATTTGCAGCAGACTGTAATTTGGAAAGT
AGACATCATAATTACGTATGCAGGCAAAACCCATACATAATGTGAAATACCATTTTTGTATTTTAAGTATATT
TTATATAAATTACTTTCATTGTAATTCAGTCACCAGTGCAGCTCAGTTCAGGCTCAGGATTTAAACTTATCAG
AGTACATCAGCATGGAATTTTAACCGAAGGATACAGTACTTTCTTAAACCTAGTGCCGCTCATCACCGAGTCT
TGTATAATGCTGTGGAAGAATACCCATTTAGTATTTGTGAAAGTACTACGTGAAGTAGTTAAAAAAGACACCC
AAAACTAGAGAGTTTAGATTTGTAAAAATTAAAGTTATTAAAATCATCCTGTTCTATATTCATAAACAACTTT
TCACTTTACTGAGTAGACTAAAGATAAATCTTAAAAAAAAAAAAAAAAAAAAAAAGCCCCACCAAAAAGAAAATA
```

AGCCTCAACGTTTTAAACCAATTTGTTACAATCCTCTTCCCTAACGCTAGGGTGTTCAAAGCATCTTTTGAAA
TAACATTTTTCTTCCTGAGTAACACGGAATCAGTCTGACTGATAATTCTGATTTTCACAGTGGGCTGATAGAT
ATAAATGATACCATCTTTATTTTCAGATAAAAAAACACATACATATAACTCACTAATTTTCTAGATTCTGATC
AGAACTGTCTTTATTCTTTCCACAGCAGACTCTAAGGTTAATGTAAAATTTTCTGAAGTAGTATTCATAAGTA
ATATATACGTTGGAGAAACAATATAGCATAGTGAAACAAATAATTCAGTCAGGAGATCTAGGTTTATGTCCCT
TACAGGTAAGTGGTTATAAGCCACCTACTTGCCAGCTATGTATCTGTGGGCAAAGTGCTTTGAGAATGACATG
AGATCACATCTGTGAATTCATTTTGTACGTATAAAGTGGTACAAGTGGTGTGCCAATGTAAGTTAGTGTCCTG
TTATTTGAATTTATTTTCAGCCGATTTGTTTTCAAGTTTCTTTTTTGGCTTCACTATTTAGCTGACTTATTTT
GAAAAAATTTTAATTAAGAACTAATTGACACATCAGGAAACTATGACACATCATTAATTTAAAAATCATTGGT
GAAGTGCTGTTGACTTCACAAATGTCAGTACAAAATGCTGCAAAAGAGAAAGCTATTACACATATACCTGTCT
GAAAGAAAACAAAAGACAAAAGAAACTGCGTTATCTTTTTGAACACAGTAATGTTATAGAAGTTAATAAGAAA
GGAGGGTTCCTGCTTTGTTAATTAGAGCCTAGAAGTTACTGATTCTACACAGCTTTACTAGAGATCAAATCTA
AATTGTCAAATCAACTAAAGCCGAGGTTACTGCATTTCTCTATTCTTTCGTGCTTGTACTTGCTATTTTGGGT
CTGTAACTAATTCCTAATTCTTTCCTTTAACAGCGTTATTTCATGACAATGATGTGAAAGAAAAAATTTAAAAC
ACTATTTTTAAAGTTCTTCCTTTCAAAAATGTCTCACATTATTGCTTTTTCCAAATGACATTAAGCTGCACTA
CCTTGAACTACTGGGAACCTGATTAGATCTCCCTTCCCTATAGACAATTTACCAATTCCTTCTCAGTTCATTC
AGAAATCCCAAACAGAATAAAACAAAACAAAACAAATTCTGAAATTCTTGTAGTTTCTTTTTCTCCTTTCCAA
TTCCTCCTTGATTTGTGGATGAACTTTGGGTATGTGTTTCCTTGATAAACAAGCTATATTACAGTATCGTCTC
TGCACCATAGTGTTTGGATGTATTTTAATTTAGAAATGTAACATCTGGCAGAAAACTGTGTCAGACTACGAGA
GGTTATGGAAATGCACTGATTCTCAACTGGGCAAGATTTTTGAGCCCCAGGGGCATTTAGCGACGTTTAGAGA
TTGGCTGTCACAACTGAGATGTATTCCTGGAATCTGATGGGCCGAAGGCCAGGCACACTACTGCGCATCCTAC
AGTGTAAAGACAGCCTCCTACCATAAGGAAGTATTTGGTGCACAATTTGAAAAGGGTCTGGTTAAGAAACCTT
GTCACCGTGCCACAAGAATTGAAGAGGAAAATTCTTCTTTGGGAAGAACCTGATTTCCATCGCTCACTAAAGT
GAATCTTTTCATGACCTCGGTTTCAGTTTCCTTGCTTGAAAACGAATGGCCGGAAAAGACCTCGGGTGTCTCT
TCTGATTCTCATACTCATTTGGATACTCGAAATAACCGTAGTTTGGTAAAGAAGAAAAAAGGCATTTGATATT
ATTAAGAAGTTTGACTTTAGCTTGGATCTTACAAACCGGCTGCCTGCTTAACTGGAATCGTACATATAAAATT
CACTGAATCTCTCTAACAGCGTCATAATACTTTAAATGAAGGAAGTAATGATCATGTCCTAGTCCTCAGCCAG
CAGGTGGCGCTCAAAGCTAACAAGGTAAGCAATGTACCTCGTTTTCTGCAACGTACTTCACTTTTACCATGGC
TCGAGTAGCAGGGATTGTTCAATTCCGACTGTGTACTTATACATAATTATATAATGTATATATAAAAATCCAC
AATCAACAGACAATCTTTGGTTAGTTTTAAACTACGGCCAAAAATATAAATGAATGCTTCGGATAAGCAAAAG
TTTAGTTTGAAAGAAAGTACCATCGTAACCGTCAATGGCATCCTGAAAACAAACTGCATTAAAGAAGTAATTT
TCTTAACCGTATCTTCAAGTGAGTTGTTGAATTTTCAAATGAGAAATGTTGCAATAGTAAACAGGGGTGAGCT
TCAACACCATCATACACGCAACTCTCACTGCTACATAGGGCAAATACATTCCTTGTTACATGTGGACAACCAA
GTGACAACGACAGCTAAAAGCTGCAAAAAAATTATCGTTATTTAAACTCCTGGCATGTCAGCTCCTTTGCCAG
TATTATCTAATTCAATTACTATGTCAACCTGTAAGCAAACTGATACTTATATAAACTGACCAGGAAAAAGCCT
ATCATTTGTAGTCAGCAAAGTTACATTCACAGCAATAGAAGAGGAGCAAATAAAGAGAGTGATAAAATTAAGA
AAATATGACAGGAAAATCAGAATCAAAACCTTAAGCAAATCAAAGAGCAGATTCTCGGGGAGTGGTGCGTGGG
GAGGATGAAATTCAAGCAATAAACAATCCTGGCAAAACAAAGCAAGAAAACACAAGAAAGCAAAAGTATACAT
GAGACCTGAAAAATGGGTTGCGGCCACAGATAATAGAAGAATGCTAAGCAGAAACTCTATTTTCAATGAGGAA
GAAAGTATTTCTCAACGCGTTTTACAAAGCTAAAAGCATATAGGTAACAAAGCCTCATCCAGATGATCCATCC
CTGCCCTCAACACAAATGCAAAATTCCAGCAGTATATAAAGAGTCTAAGTTTACATTGGGAATGCAAGAATAC
TCCATTCGCAGGATACATTACTTTAGTTCATCACTGAAAATCATTTGATAAAATACAGCACTCATAATTTAAA
TTTTTTAAAAACCCAAGTAAAATAGAGGTAGAGGAATCTTATTTTCTATCAATCTCATTCTACCCTATCATCA
AGCTTACAAGTGAAATAGTTGAGTCAACTCAATTGAAAGTAGGAATGAGGTAAGGGCACCAGGGCACCTCCTT
ATTACTCCTGCATATGTTTTCCACTGTGTATGACAAAAGTGAATACTAATACAAAGTATTCTTATGAATCAGT
AAGAAAAATAAAATTAAAAAGGTAATTTTAAAAGCTAAAGATCAATGATCAACTTCAATGATGATTTTTAAAA
GTGCACATCAACATAATGTAATATTTTCCAGCTATTACGCTGACAATTTAAAAAATACTAATAACTTTCACTG
GAATGGGTGTGGAAAAGACAGCACTCTACACACCATCAGTGAGAAAATACTAATACGTGATTTACCAAGAGTA
CTTTGGAAAAGCTGTATCATAATTTGATAAGCGGGGATACTCACCACTATACTAAAAAGGAGAATTCATTATA
AAATTGTTATACAAGGGGCAAAGTGCTTTCACCTAGCAATTCCACTTATAGCAATTCATCTCAAGAAATTAAT
AGTACAAGCGTGCCAAGATATTTACACAAAGATATTCACAGCATTGTTCTTTTTGAGACTGAGTCTCTCTTTG
CCGCCTAGGCTGGAGTGCAGTGGCACAATCTCAGCTCACAGCAATCTGCGCCCCAGGATCACGTGATGCTGCT
GCCTCAGCCTCCCGAGTAGCTGGGATTACAAGTGTGCGCCACCACGCCTGGCTAAATTTTTTGTATTTTTAGT
AGAGACAGGAAACAAAAATCATTCAAATATTCCTTCACATTTTCAAAAACACATGAGATAACACAACATTGAA
GTACATACGCTGGTTCCTTTAATTTGTTATTACAATAAAAGAAACAGAATGGAAAAAAGAATTACTTCAAGTT
TCTAATCCCTGACGTTCTTGTTGTTACTTTTATATGTAAAACCTCAACTTTTTCCCAATTTTCTGGGGTTGGT
ATTGTGGAAATCTCAAGGATATTAGTTCTTTGAATGTATTACCATAGATATGATCATGGGTCATATATACAGT
CATATCTATGAAAAGAGACACAGAGGACTACTATTGTGAAGCAGCCAGCTAAAATAAAAATATAATTCAAATT
CTGTGCTCTAAAAAGTGGGTAATAATTTTATTTCACTCTGTCTCTCTAAAAAACTGATAAAAGTCAGTCTGGA
TGTTTCGGCTATTTGACGGCAAAGATTTAAAAAAAAAAAAAAAAAAAAAAAAAACATGCTACAATATAGAAGGGG
ACACCAAATCTCAAAAACCTATTCTACAGTAAAGTTTTTGCTAAGTACATTCCTGTCAAAATATTACTCAATT
ACTTCTAAATAATACAGAGGCCTTCATTCTAGACTAATTTGAAGTGTTGTCTTAAATTTTAGGTACATTTCAC

TTCTTTAAAATGGCAAACTATTCAAGCAATTTGTATAAACAAAGGGCTCAATAATATCTGAAAGTAAATCATT
TTACTCCCTCTTAAATTACCTGATAATTATATACAGGCAAATGATATCTAGTGATGCCGTGAACTGCTGAATT
TGGGTGAGTAGTGTGTGCCTATAAATAAAGTTTACAGTAAGAATGAATGAATACGGTAAAACATTTTGTTAAT
TAGAAATACTATTCCCAATATAAAAAACTATGAAAAAGTTTTAAAACATTACTTTTCTATATACAGCACTGCA
GAATTCTAAATGAGTGACTGATTTTATGAAGAAGAAATATTCTGTCAAGTGAGGCCCTTTGGCTGGGGAAGGG
GAACAGACAAATGACAAAAGAAGGGACTATTTCACCAGACAAGTTTACCTTATTTATACTGTGTACTTACGCC
CGCCCAGAAGTTATTTCTTACGCTGGTGATAAGGCTCTATTAAGACAGACTTCAATTGTAAGTTAAATTAATC
CATTTGCTATTTCTTTGTTAAAATACTTCTAAAGGGTTTTCTATTTGACAATATTATAGGGTAATACGACGTT
CTCCTACAAATGTTACGGCTTTTTCTGTACTTCATTTCAAAAAACTAAGGGCAGTATATGATCCACAGCTGGA
AAAGAGACAGTATGGTGTCTTCTACGTTTCAATAAATACTTACTGATTGAAAACTATACGTAGCATCACACAT
GAATACACCCAGATTACGTAATGGCTCACCGTAAATGTGAGAAACAGGGCTTTTTTGCTAGCCATCGTTCAGA
GGACAAAAAAGAAGCAGAGGTATACCCTACCTGTTTCAAGCACATGGAAAACGTCAACAAACGAGAGACACTG
AAGAACTATTTCACCACTATTTTGTTACTTTATTTTCCATCAAAGAAAATGTCTTTTAAACTAAGACATCAAT
AAAACAAACTAAAAAGAAAATAAACATTACTTATCCCCAGTAAGTGACAGAGTATGTCAAATCCTACTTTAAA
TATCAAGGTAACCAGCATCAGAGAAATCACATGCCCGAAACTCACGGGATTTATAAATATAGGAAAACACATC
AGAAATCTACCCATTCCAGAACCAGAATATATCCAGAAGTCAGCAATCTATATGAGGAGACATCTGGAAATCA
TTGCAAGTAAAGAACAGCTGGATGAATTGCTAACCTTCGGGAAGAATAAACTAGGCAGACACACGAAGACAGC
TGCTTTCAAATATTTTCGGAACTAGTTATGTGGGGGGAAAGCAGTTCGGGTGTTTTAGAGGTAATACTCTTTT
TTCTTCCTACTCTTATTTAAGAGTAATTAATAGCAAAACATTTCTGTTTCTCTTGAACACTTTTTTTTTTTTT
TTTTTTTTTTTTTTTTTACGGAGGGTAAAGCCAGAGGCAGATTCCAGGCAGATACATGCTCATTCTAAAGCCA
CTATTAATACTACCTTTCATGGAGTGTATAGTCTATCAAAAAGTTACTGAATTCTTTCTTATCATCATGTGTA
CGAGCCATTCCTTAAGCACGCAAAAACCTGACAGAGAAAAAGGCACTGTTGCTCCCATAGGAGTTTAAAATTG
GGTTAAAAAGAAAGTAACAAAATGTGCCACATTAATACAAAGAACGATTTAAAAAATTTATAGGCATATATGA
CACAGAAAAAAAAGAAAGAACAGGGAGTATAGGTTCGGCGCATTCACTTTATCTGAAGTACAGCATAACTCCT
TTGCTCCCCAACAGGCCACTGCGGTGGCAACTTGAAAAAAAAAAAAAAAAAAGGAAACCAATATTATTCAAATA
TTCCTGTACTTTTTCAAAAACACATGAGATACACAATACTGAAGTACTTCTCATGCTGGCTCCTTGGTTAATA
TAACGAAAGAAACAGAATAGAAAAAAAGAAGTACTTTAGGTTTC

**Supplementary figure** 1: GRM diagram for the 5607 bp consensus sequence computed by using key string ensemble of: (**a**) 8 bp key strings, (**b**) 3 bp key strings. For description see the text.

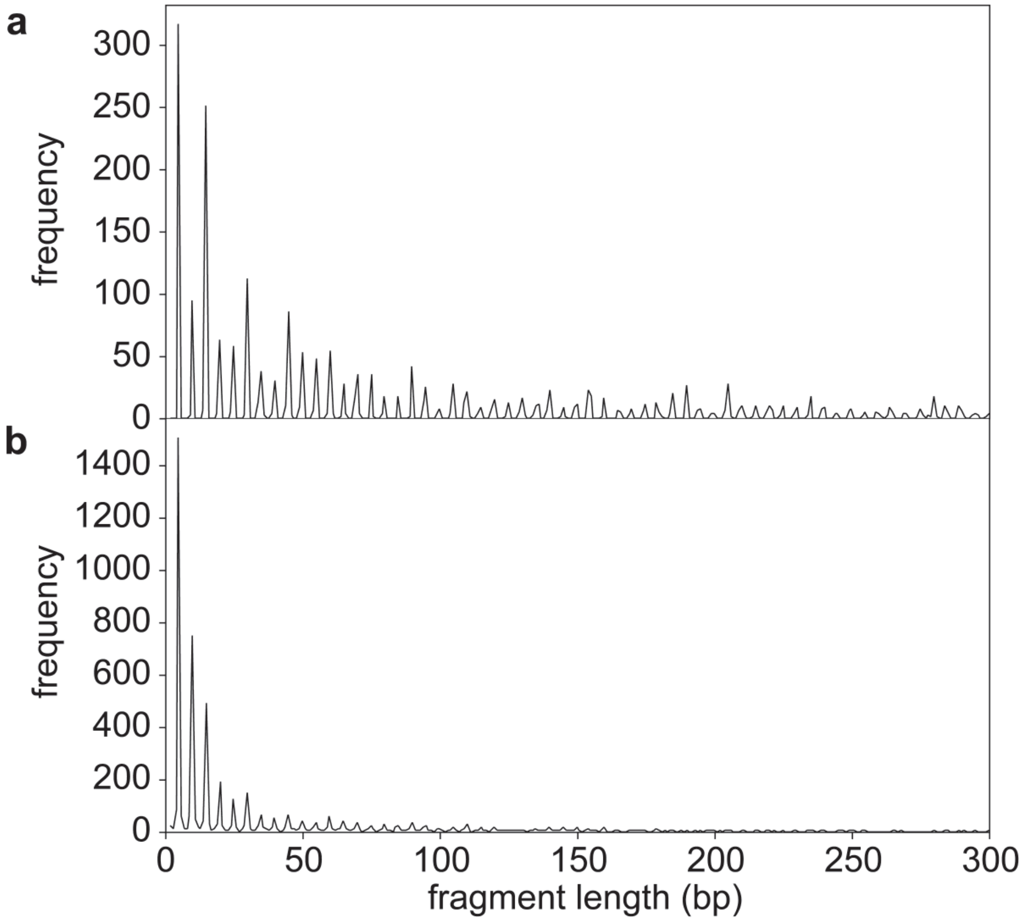

**Supplementary figure** 2: The GRM diagram computed for the human 10848 bp consensus repeat unit exhibiting a moderate peak at 2452 bp.

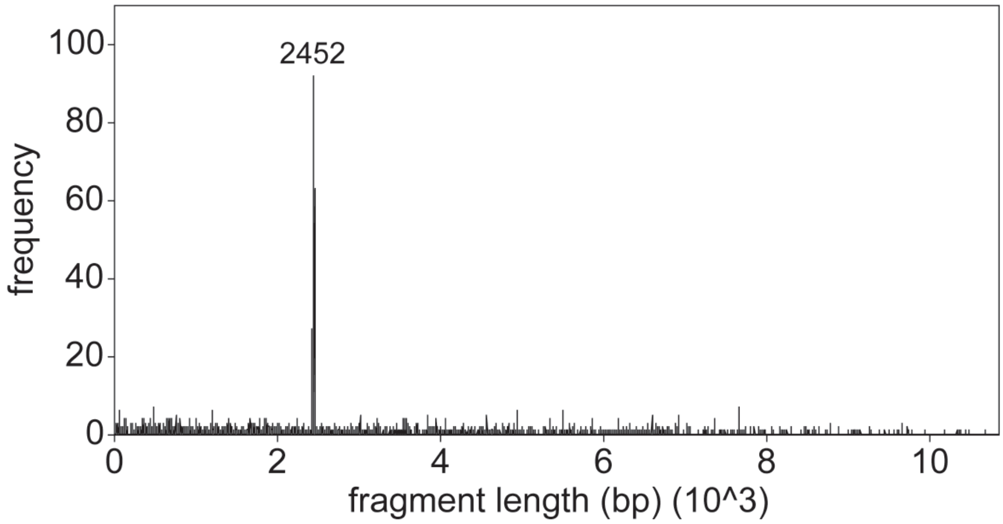

Supplement: Supplementary file 1 [file supplementary.pdf]
